# Supplementary material for: A Brief History of Fr\'echet Distances: From Curves and Probability Laws to FID
Source: arXiv:2604.21745 source file (2026-04-23)
Supplement: Supplementary file 1 [file frechet1906_fr.tex]

% This LaTeX document needs to be compiled with XeLaTeX.
\documentclass[10pt]{article}
\usepackage[utf8]{inputenc}
\usepackage{amsmath}
\usepackage{amsfonts}
\usepackage{amssymb}
\usepackage[version=4]{mhchem}
\usepackage{stmaryrd}
\usepackage{mathrsfs}
\usepackage{bbold}
\usepackage[fallback]{xeCJK}
\usepackage{polyglossia}
\usepackage{fontspec}
\usepackage{newunicodechar}
\IfFontExistsTF{Noto Serif CJK SC}
{\setCJKmainfont{Noto Serif CJK SC}}
{\IfFontExistsTF{STSong}
  {\setCJKmainfont{STSong}}
  {\IfFontExistsTF{Droid Sans Fallback}
    {\setCJKmainfont{Droid Sans Fallback}}
    {\setCJKmainfont{SimSun}}
}}
\IfFontExistsTF{Noto Serif CJK KR}
{\setCJKfallbackfamilyfont{\CJKrmdefault}{Noto Serif CJK KR}}
{\IfFontExistsTF{Apple SD Gothic Neo}
  {\setCJKfallbackfamilyfont{\CJKrmdefault}{Apple SD Gothic Neo}}
  {\IfFontExistsTF{UnDotum}
    {\setCJKfallbackfamilyfont{\CJKrmdefault}{UnDotum}}
    {\setCJKfallbackfamilyfont{\CJKrmdefault}{Malgun Gothic}}
}}

\setmainlanguage{french}
\IfFontExistsTF{CMU Serif}
{\setmainfont{CMU Serif}}
{\IfFontExistsTF{DejaVu Sans}
  {\setmainfont{DejaVu Sans}}
  {\setmainfont{Georgia}}
}

\title{\Large MEMORIE E COMUNICAZIONI. \\
SUR QUELQUES POINTS DU CALCUL FONCTIONNEL}

\author{Maurice Fréchet}
\date{}

%New command to display footnote whose markers will always be hidden
\let\svthefootnote\thefootnote
\newcommand\blfootnotetext[1]{%
  \let\thefootnote\relax\footnote{#1}%
  \addtocounter{footnote}{-1}%
  \let\thefootnote\svthefootnote%
}

%Overriding the \footnotetext command to hide the marker if its value is `0`
\let\svfootnotetext\footnotetext
\renewcommand\footnotetext[2][?]{%
  \if\relax#1\relax%
    \ifnum\value{footnote}=0\blfootnotetext{#2}\else\svfootnotetext{#2}\fi%
  \else%
    \if?#1\ifnum\value{footnote}=0\blfootnotetext{#2}\else\svfootnotetext{#2}\fi%
    \else\svfootnotetext[#1]{#2}\fi%
  \fi
}

% \newunicodechar{Σ}{\ifmmode\Sigma\else{$\Sigma$}\fi}

\sloppy

\begin{document}
\maketitle

 Par M. Maurice Fréchet (Paris)\footnote{Thèse présentée à la Faculté des Sciences de Paris pour obtenir le grade de Docteur ès Sciences.}
 
Adunanza del 22 aprile 1906.

\section*{INTRODUCTION.}
\textbf{1.}
 On s'accorde assez généralement à considérer un nombre $y$ comme fonction de la variable $x$, quand à toute valeur numérique de $x$ correspond une valeur bien déterminée de $y$. Lorsqu'on impose à cette correspondance certaines conditions de continuité, dérivation, etc., on obtient des classes de fonctions jouissant de propriétés précises. C'est l'étude de ces propriétés qui constitue le principal objet de l'Analyse moderne.

La notion de fonction ainsi comprise a été progressivement étendue dans plusieurs directions (par exemple en ce qui concerne l'uniformité) et en particulier au point de vue de ce qu'on doit prendre pour variable. Depuis longtemps, on a considéré des fonctions de deux, de trois, ou même de $n$ variables numériques. Les autres généralisations sont plus récentes. Ainsi, M. \textsc{Le Roux} a été amené à étudier les fonctions dont la valeur dépend non plus de $n$, mais d'une suite infinie de variables indépendantes (\textsc{xviii})\footnote{Les chiffres romains renvoient à la bibliographie rejetée à la fin du Mémoire.}. MM. \textsc{Volterra} (\textsc{xv}) et \textsc{Arzelà} (\textsc{v}) paraissent avoir été les premiers à étudier systématiquement les fonctions dont la valeur dépend de la position et de la forme d'une ligne variable. M. \textsc{Hadamard} (\textsc{xi}) a considéré une classe particulière de fonctions dont la variable est la forme d'une fonction ordinaire.

Nous nous placerons dans ce Mémoire à un point de vue tout à fait général qui embrasse ces différents cas.

Pour cela, nous dirons qu'une \textit{opération fonctionnelle} $U$ est définie dans un ensemble $E$ d'éléments \textit{de nature quelconque} (nombres, courbes, points, etc.) lorsqu'à tout élément $A$ de $E$ correspond une valeur numérique déterminée de $U: U(A)$. La recherche des propriétés de ces opérations constitue l'objet du \textit{Calcul Fonctionnel}.

\textit{Le présent travail est une première tentative pour établir systématiquement quelques principes fondamentaux du Calcul Fonctionnel et les appliquer ensuite à certains exemples concrets.}\\

\textbf{2.}
Dans ce but, il a d'abord fallu généraliser la théorie des ensembles linéaires qui a fait faire tant de progrès à celle des fonctions d'une variable. On pourrait objecter que pendant longtemps la théorie des fonctions a pu se passer de la considération des ensembles ponctuels. Mais l'étude préalable des ensembles s'impose avec bien plus de force dans le Calcul Fonctionnel. Rien en effet (au début, du moins) ne vient jouer, dans le Calcul Fonctionnel, le rôle de l'intervalle dont la considération a suffi pendant si longtemps aux analystes pour la théorie des fonctions.

L'utilité de cette étude préalable des ensembles étant admise, une difficulté se présentait. La première généralisation qu'il était naturel de se proposer est celle de la notion de fonction continue. Or, si on veut l'étendre à des opérations dont la variable soit un élément \textit{de nature quelconque}, il faut d'abord savoir ce que l'on doit entendre par éléments voisins ou par limite d'une suite d'éléments. Cela parait impossible: on a l'habitude de donner une définition spéciale de la limite pour chacune des catégories d'éléments considérés jusqu'ici : points, courbes, etc. J'ai tourné la difficulté par une méthode analogue à celle qui permet dans la théorie des groupes \textit{abstraits} de raisonner sur un mode de composition non défini explicitement.

Après avoir développé ce point de vue, je remarque que presque toutes les définitions classiques de la limite (mais non toutes) peuvent se traduire de la manière suivante: Pour la catégorie d'éléments considérée, on peut faire correspondre à tout couple d'éléments $A, B$, un nombre $(A, B) \geqslant 0$, ayant des propriétés très analogues à celles de la distance de deux points et tel que: $\mathrm{1}^{\circ}\, B$ coïncide avec $A$ si $(A, B)=0$ et $2^{\circ}\, B$ tend vers $A$ si $(A, B)$ tend vers zéro. En adoptant cette hypothèse moins générale, mais cependant très étendue, on obtient des résultats plus précis et plus nombreux.

\textit{La voie que nous venons d'indiquer nous a conduit à la généralisation de presque tous les théorèmes sur les ensembles linéaires et sur les fonctions continues (du moins, de ceux qu'on peut énoncer d'une manière indépendante de la nature des éléments que l'on considère)}.

Il fallait d'abord voir comment transformer les énoncés des théorèmes pour qu'ils conservent un sens dans le cas général. Il fallait ensuite, soit transcrire les démonstrations dans un langage plus général, soit, lorsque cela n'était pas possible, donner des démonstrations nouvelles et plus générales. Il s'est trouvé que les démonstrations que nous avons ainsi obtenues sont souvent aussi simples, et quelquefois même plus simples, que les démonstrations particulières qu'elles remplaçaient. Cela tient sans doute à ce que la position de la question obligeait à ne faire usage que de ses particularités vraiment essentielles. D'ailleurs, nous n'avons eu besoin dans cette \textsc{Première Partie} que des notions les plus élémentaires (en dehors de la définition et des propriétés de la puissance d'un ensemble).

Dans la \textsc{Seconde Partie} nous avons appliqué les résultats généraux ainsi obtenus, à diverses catégories d'éléments, chacune d'une nature déterminée. La seule difficulté consistait à montrer que chacune de ces catégories se trouvait répondre aux conditions générales nécessaires pour la validité des théorème de la \textsc{Première Partie}. Cela fait, il ne restait plus qu'à énoncer ces théorèmes dans chaque cas. Nous attirons en particulier l'attention sur la définition que nous avons donnée de «l'écart» de deux courbes, de deux fonctions holomorphes, etc. Il semble que ce soit par ce seul moyen qu'on puisse (en généralisant ainsi la notion d'intervalle) s'affranchir un peu de la considération des ensembles.

Chemin faisant, nous avons précisé la définition de deux courbes et complété un théorème important de M. \textsc{Arzelà} sur les ensembles «compacts» de courbes.

D'ailleurs une table des matières indique en détail les divisions adoptées.

J'ose espérer que les propositions nouvelles que j'ai pu obtenir dans le cas des courbes par exemple, justifieront l'utilité des considérations générales dont je les ai déduites. Mais si la preuve restait à faire de cette utilité pour les applications, elle résulterait manifestement de l'usage qui a été déjà fait des cas particuliers classiques; par exemple par M. \textsc{Arzelà} en ce qui concerne les ensembles de fonctions (\textsc{vi, viii}) et par M. \textsc{Le Roux} pour l'espace à une infinité de dimensions (\textsc{xix}).\\

\textbf{3.}
Pour plus de netteté, les propositions que je crois nouvelles sont les seules imprimées en italiques. Quelques-unes d'entre elles ont d'ailleurs été déjà présentées à l'Académie des Sciences les 21 Novembre 1904, 2 Janvier, 27 Février, 20 Mars et 27 Novembre 1905, ou publiées sous une autre forme dans une Note des \textit{Transactions of the American Mathematical Society} (\textsc{xxvii}). Enfin, pour ne pas être trop long, j’ai laissé de côté des recherches se rapportant à d'autres parties du Calcul Fonctionnel et que j'avais publiées ailleurs (\textsc{xxvii}).

Je ne veux pas terminer cette \textsc{Introduction} sans exprimer la reconnaissance que je garde à mes maîtres pour les encouragements qu'ils n'ont cessé de me donner. Je dois remercier tout particulièrement M. \textsc{Hadamard} qui a bien voulu s'intéresser au développement de ce travail et dont les précieuses remarques m'ont amené à en perfectionner en bien des points la rédaction.

\newpage
\section*{PREMIÈRE PARTIE.}
\section*{INTRODUCTION DE LA NOTION DE LIMITE DANS LES ENSEMBLES ABSTRAITS.}
\section*{Chapitre I.} 
\subsection*{Notions générales sur les ensembles d'éléments d'une classe ($L$).}

\textbf{4.}
\textit{\textbf{Objet du Calcul Fonctionnel.}}---Considérons un ensemble $E$ formé d'éléments quelconques (nombres, points, fonctions, lignes, surfaces, etc.) mais tels qu'on en sache discerner les éléments distincts. A tout élément $A$ de cet ensemble faisons correspondre un nombre déterminé $U(A)$; nous définissons ainsi ce que nous appellerons une \textit{opération fonctionnelle} uniforme dans $E$.

L'étude de ces opérations est l'objet du \textit{Calcul Fonctionnel}. Il est à présumer que les propriétés de chaque opération dépendront, d'une part des propriétés de l'ensemble dans lequel elle est définie, d'autre part de la nature de la correspondance qui définit l'opération, c'est-à-dire de la correspondance (non univoque) entre les éléments de $E$ et certains nombres qui sont les valeurs de l'opération. On voit donc que le calcul fonctionnel comprend nécessairement une théorie préliminaire des ensembles.\\

\textbf{5.}
\textit{\textbf{Théorie des ensembles.}}---Les résultats qu'on obtiendra dans une telle théorie seront d'autant plus étendus qu'on s'adressera à des ensembles plus généraux. Pour obtenir la plus grande généralité possible, il y aurait donc lieu de chercher d'abord des résultats applicables à des ensembles abstraits, c'est-à-dire dont on ne spécifie pas la nature des éléments.

Les résultats les plus importants qui ont été obtenus jusqu'ici dans cet ordre d'idées sont ceux qui concernent les notions (introduites par M. G. \textsc{Cantor}) de puissance d'un ensemble et d'ensemble ordonné.

Pour la \textsc{Première Partie} de ce travail, je n'aurai à supposer connus (en dehors des notions mathématiques les plus élémentaires) que ces résultats, et même seulement les plus simples d'entre eux\footnote{Voir par exemple \textsc{ii}, pages 1, 2; et \textsc{iii}, pages 27, 28.}. En particulier, je n'aurai pas à utiliser la théorie des ensembles linéaires et des fonctions continues qui apparaîtra, au contraire, comme un corollaire très particulier de notre théorie générale.\\

\textbf{6.}
\textit{\textbf{La notion de limite dans les ensembles abstraits.}}---Les résultats les plus connus et en fait les plus importants de la théorie des ensembles sont ceux que l'on déduit de la notion de limite d'une suite d'éléments. Or, on n'introduit jamais cette notion qu'après avoir abandonné l'étude des ensembles abstraits et en spécifiant bien nettement la nature des éléments que l'on considère. C'est le même fait qui se produisait lorsqu'on développait séparément les théories des groupes de mouvements, de substitutions, de transformations, etc., où chaque catégorie d'éléments donnait lieu à un mode de composition parfaitement défini, mais dont la définition variait d'une catégorie à l'autre. On ne put arriver à une théorie commune qu'en \textit{s'abstenant} de donner une définition générale de ce mode de composition, mais en recherchant les conditions communes aux définitions particulières et en ne retenant que celles qui étaient indépendantes de la nature des éléments considérés (\textsc{xxiv}). C'est aussi d'après le même point de vue qu'on a été amené à simplifier l'étude des forces, des vitesses, des rotations, etc., en les faisant précéder d'une théorie des vecteurs. Cette idée se retrouve un peu modifiée dans l'usage qui tend à se répandre des définitions « descriptives » particulièrement préconisées par M. \textsc{Drach} (\textsc{xxi}). Telles sont, par exemple, les définitions de la mesure d'un ensemble qui ont été proposées par M. \textsc{Borel}\footnote{«Dans tous les cas, elle procède de la même idée fondamentale: définir les éléments nouveaux que l'on introduit à l'aide de leurs propriétés essentielles, c'est-à-dire de celles qui sont strictement indispensables pour les raisonnements qui doivent suivre» (I, page 48).} et M. \textsc{Lebesgue} (\textsc{iv}, page 102); la définition de l'aire introduite par M. \textsc{Hadamard} dans ses Leçons de Géométrie Élémentaire (\textsc{Armand Colin}, 1898), etc. Mais il y a cette différence que dans la définition « descriptive» on énonce des propriétés \textit{caractéristiques} de l'être que \textit{l'on veut définir} (\textsc{iv}). Au contraire, dans la théorie des groupes abstraits, le mode de composition est supposé défini à l'avance dans chaque cas particulier; mais on ignore volontairement cette définition pour ne retenir que certaines conditions générales qu'elle remplit \textit{mais qui ne la déterminent} pas.

En procédant ainsi, il arrive que certaines démonstrations sont rendues plus difficiles puisqu'on se prive d'une représentation plus concrète. Mais ce que l'on perd ainsi, on le regagne largement en se dispensant de répéter plusieurs fois sous des formes différentes les mêmes raisonnements. On y gagne souvent aussi d'apercevoir plus nettement ce qui dans les démonstrations était véritablement essentiel et de les simplifier ainsi en les débarrassant de ce qui ne tenait qu'à la nature propre des éléments considérés. C'est ce que nous allons essayer de faire pour le Calcul Fonctionnel et en particulier pour la théorie des ensembles abstraits.\\

\textbf{7.} 
Si l'on examine avec soin les diverses définitions classiques de la limite d'une suite de nombres ou d'une suite de points ou d'une suite de fonctions, etc., on remarque immédiatement que toutes ces définitions satisfont à deux conditions I et II que l'on peut énoncer indépendamment de la nature des éléments considérés. Ce sont ces conditions qui nous suffiront tout d'abord pour généraliser certaines propositions de la Théorie des Fonctions.

\textit{Dorénavant, nous nous limiterons donc à l'étude des ensembles tirés d'une classe ($L$) d'éléments de nature quelconque mais satisfaisant aux conditions suivantes: on sait distinguer si deux éléments de la classe ($L$) sont distincts ou non. De plus, on a pu donner une définition de la limite d'une suite d'éléments de la classe ($L$). Nous supposons donc qu'étant choisie au hasard une suite infinie d'éléments (distincts ou non) de la classe ($L$), on puisse dire d'une façon certaine si cette suite $A_{1}, A_{2}, \ldots, A_{n}, \ldots$ a ou non une limite $A$ (d'ailleurs unique). Le procédé qui permettra de donner la réponse (autrement dit la définition de la limite) est d'ailleurs absolument quelconque, assujetti seulement à satisfaire aux conditions I et II dont nous avons parlé et qui sont les suivantes:}

I) \textit{Si chacun des éléments de la suite infinie $A_{1}, A_{2}, \ldots, A_{n}, \ldots$ est identique à un même élément $A$, la suite a certainement une limite qui est $A$.}

II) \textit{Si une suite infinie $A_{1}, A_{2}, \ldots, A_{n}, \ldots$ a une limite $A$, toute suite d'éléments de la première suite pris dans le même ordre: $A_{n_{1}}, A_{n_{2}}, \ldots, A_{n_{p}}, \ldots$ (les nombres entiers $n_{1}, n_{2}, \ldots, n_{p}$ iront donc en croissant) a une limite qui est aussi $A$.}\\

\textbf{8.} 
\textit{\textbf{Les définitions usuelles de la théorie des ensembles ponctuels étendues aux ensembles abstraits.}}--- Il nous est actuellement possible, dans l'hypothèse où nous nous sommes placés, de généraliser les définitions qui sont ordinairement adoptées dans la théorie des ensembles ponctuels.

Nous considérons donc un ensemble quelconque $E$ d'éléments d'une classe ($L$) où l'on sait définir conformément aux conditions I et II, la limite d'une suite d'éléments.

Nous dirons qu'un élément $A$ de la classe ($L$) est un \textit{élément limite} de $E$ lorsqu'il existe une suite infinie d'éléments de $E: A_{1}, A_{2}, \ldots, A_{n}, \ldots$ qui sont distincts et tendent vers $A$. Nous appellerons \textit{ensemble dérivé} d'un ensemble $E$ et nous désignerons par la notation $E^{\prime}$ l'ensemble des éléments limites de $E$. Nous dirons qu'un ensemble est \textit{fermé} lorsqu'il contient son ensemble dérivé; qu'il est \textit{parfait} lorsqu'il coïncide avec son dérivé. Enfin, considérant un ensemble donné $H$ comme ensemble fondamental, nous dirons qu'un élément $A$ d'un ensemble quelconque $E$, formé d'éléments de $H$, est \textit{intérieur} à $E$ \textit{au sens étroit} lorsque $A$ est un élément de $E$ qui n'est limite d'aucune suite d'éléments distincts $A_{1}, A_{2}, \ldots, A_{n}, \ldots$ appartenant à $H$ sans appartenir à $E$.

Ces définitions sont usuelles dans le cas particulier des ensembles ponctuels. Nous introduirons encore avec M. \textsc{Lindelöf} (\textsc{ii}, page 4) la notion d'élément de condensation d'un ensemble. Mais nous donnerons une définition différente de la sienne (qui ne se prête pas à la généralisation actuelle), quoique équivalente dans le cas où il se place, celui des ensembles ponctuels. Nous appellerons \textit{élément de condensation} d'un ensemble $E$, un élément limite de $E$ qui est aussi un élément limite de tout ensemble obtenu en supprimant de $E$ une infinité \textit{dénombrable} (\textsc{ii}, page 2) d'éléments. On voit qu'un ensemble ne peut donner lieu à un élément limite que s'il possède une infinité d'éléments distincts et qu'un ensemble ne peut donner lieu à un élément de condensation que s'il possède une infinité non dénombrable d'éléments.\\

\textbf{9.} 
\textit{\textbf{Les ensembles compacts.}}---Nous verrons par la suite qu'il y a utilité à introduire une nouvelle notion, celle d'ensemble \textit{compact} qui joue le même rôle dans la théorie des ensembles abstraits que la notion d'ensemble limité dans la théorie des ensembles ponctuels. Nous dirons qu'un ensemble est compact lorsqu'il ne comprend qu'un nombre fini d'éléments ou lorsque toute infinité de ses éléments donne lieu à au moins un élément limite \footnote{Voir plus loin un exemple d'ensemble compact ( $\mathrm{n}^{\circ} 86$ ) et d'ensemble non compact ( $\mathrm{n}^{\circ} 85$ ).}. Lorsqu'un ensemble est à la fois compact et fermé nous l'appellerons ensemble \textit{extrémal}; cette dénomination se justifiera plus loin ($\mathrm{n}^{\circ}$ II). Le rôle de l'ensemble extrémal dans la théorie des ensembles abstraits est assez semblable à celui de l'intervalle dans la théorie des ensembles linéaires. Il y a aussi une grande analogie entre les ensembles compacts et les ensembles \textit{limités} ponctuels. Cette analogie est mise en évidence par les remarques suivantes qui résultent immédiatement de la définition: \textit{Tout ensemble contenant un ensemble non compact est non compact. Toute partie d'un ensemble compact est compacte. Tout ensemble formé d'un nombre fini d'ensembles compacts est un ensemble compact.} L'analogie se retrouvera d'ailleurs constamment par la suite.

\textit{Si on considère une suite d'ensembles $E_{1}, E_{2}, \ldots, E_{n}, \ldots$ formés d'éléments d'un même ensemble compact $E$, chacun fermé, contenu dans le précédent et possédant au moins un élément, il y a nécessairement un élément commun à tous ces ensembles.}

En effet, il y a au moins un élément $M_{1}$ dans $E_{1}, M_{2}$ dans $E_{2}$, etc. S'il y a une infinité d'éléments distincts dans la suite $M_{1}, M_{2}, \ldots$, soient $M_{n_{1}}, M_{n_{2}}, \ldots$ ceux-ci. L'ensemble $E$ étant compact, cette dernière suite a au moins un élément limite $M$; comme elle est contenue dans $E_{n_{p}}$ à partir de $M_{n_{p}}, M$ sera un élément limite de $E_{n_{p}}$ et par conséquent appartiendra à l'ensemble fermé $E_{n_{p}}$. Ainsi $M$ appartient à $E_{n_{p}}$ et par suite à $E_{1}, E_{2}, \ldots, E_{n_{p}}$. Comme cela a lieu quelque soit $p$, il en résulte que $M$ est commun à tous les ensembles $E_{1}, E_{2}, \ldots$ Si, au contraire, il n'y a dans la suite $M_{1}, M_{2}, \ldots$ qu'un nombre fini d'éléments distincts, c'est qu'il y a au moins un élément $M$ qui est répété une infinité de fois dans cette suite, soit $M \equiv M_{n_{1}} \equiv M_{n_{2}} \equiv \ldots$. Alors $M$ est contenu, quelque soit $p$, dans $E_{n_{p}}$ et par suite dans $E_{1}, E_{2}, \ldots, E_{n_{p}}$. Il est donc commun à tous les ensembles $E_{1}, E_{2}, \ldots, E_{n}, \ldots$ \footnote{ La démonstration précédente est un exemple caractéristique du genre de démonstration que nous emploierons constamment par la suite. Toutes les fois que nous aurons affaire à un ensemble extrémal, nous aurons toujours à extraire une suite d'éléments de l'ensemble, tendant vers un élément de l'ensemble. Pour se rendre compte de la transformation qu'il faut effectuer sur les démonstrations ordinaires relatives aux ensembles ponctuels, voir la démonstration correspondante de M. \textsc{Baire} (\textsc{iii}, page 18), où il utilise la division d'un intervalle en intervalles moitiés, ce qui n'est pas généralisable.}.

\subsection*{Les opérations continues.}

\textbf{10.}
Il nous est maintenant possible de définir la continuité d'une fonction dans un ensemble abstrait. Nous dirons qu'une opération fonctionnelle $V$ uniforme dans un ensemble $E$ d'éléments d'une classe ($L$) est continue dans $E$, si, quel que soit l'élément $A$ de $E$ limite d'une suite d'éléments $A_{1}, A_{2}, \ldots, A_{n}, \ldots$ de $E$, on a toujours :
$$
V(A)=\lim _{n=\infty} V\left(A_{n}\right) .
$$

Au contraire, nous ne pouvons pas encore généraliser la notion de continuité uniforme. Nous verrons plus loin comment on peut l'introduire en considérant des classes d'éléments moins générales que la classe ($L$) (voir $\mathrm{n}^{\circ}$ 47).\\

\textbf{11.} 
Nous généraliserons d'abord un résultat indépendant de la notion de continuité et qui a été énoncé d'abord par \textsc{Weierstrass} pour les ensembles ponctuels, puis par M. \textsc{Arzelà} pour les ensembles de courbes \footnote{Voir v, page 347. M. \textsc{Arzelà} y suppose en outre que $E$ est un ensemble \textit{continu} au sens que j'indique un peu plus loin (n$^{\circ} 12$), condition qui n'est pas nécessaire.}.

\textsc{\textbf{Théorème.}}---\textit{Étant donnée une opération $U$ uniforme dans un ensemble extrémal $E$, il existe au moins un élément $A$ de $E$ tel que la limite supérieure \footnote{On appelle limite supérieure d'un ensemble de nombres, une quantité $\mu$. telle que tout nombre de l'ensemble soit au plus égal à $\mu$. et que, quel que soit $\varepsilon>0$, il y ait au moins un nombre de l'ensemble supérieur à $\mu\text{---}\varepsilon$. Lorsqu'un tel nombre $\mu$ n'existe pas, on dit que la limite supérieure est infinie.} $\mu$ (finie ou non) de $U$ dans $E$ soit égal à la limite supérieure de $U$ dans tout ensemble $K$ d'éléments de $E$ auquel $A$ est intérieur au sens étroit }[\textit{en considérant $E$ comme l'ensemble fondamental} ($\mathrm{n}^{\circ} 8$ )].

Le théorème est évident si $E$ ne comprend qu'un nombre fini d'éléments ou si $U$ atteint sa limite en un élément déterminé de $E$.

Dans le cas contraire, on pourra trouver, quel que soit $n$, un élément $A_{n}$ de $E$ tel que $U\left(A_{n}\right)>\alpha_{n}, \alpha_{n}$ étant égal à $\displaystyle \mu-\cfrac{I}{n}$, si $\mu$ est fini, ou à $n$, si $\mu$ est infini.

Un même élément $B$ ne peut être tel que $U(B)>\alpha_{n}$ pour une infinité de valeurs de $n$, sans quoi l'on aurait $U(B)=\mu$, ce qui est contraire à notre hypothèse. Il y a donc une infinité d'éléments distincts dans la suite $A_{1}, A_{2}, \ldots, A_{n}, \ldots$, et comme $E$ est compact, cette infinité a au moins un élément limite $A$. En définitive, il y a une suite $A_{n_{1}}, A_{n_{2}}, \ldots$, extraite de la première et qui tend vers un élément $A$ de $E$, car $E$ est fermé.

Je dis que $A$ satisfait à la condition annoncée.

En effet, si $K$ est un ensemble auquel $A$ est intérieur au sens étroit, les éléments de la suite $A_{n_{1}}, A_{n_{2}}, \ldots$, sont tous des éléments de $K$ à partir d'un certain rang $q$ (sans quoi $A$ serait limite d'une suite d'éléments de $E$ n'appartenant pas à $K$). Mais alors la limite supérieure $\mu_{\mathrm{1}}$ de $U$ dans $K$ est au moins égale à $U\left(A_{n_{p}}\right)>\alpha_{n_{p}}$ quel que soit $p>q$. On a donc $\mu \geqslant \mu_{\mathrm{1}}>\alpha_{n_{p}}, \alpha_{n_{p}}$ tendant vers $\mu$. D'où $\mu_{\mathrm{1}}=\mu$.

Le théorème précédent s'énoncerait de la même manière pour la limite inférieure.

On en déduit immédiatement l'important corollaire suivant:

\textsc{\textbf{Corollaire.}}---\textit{Toute opération continue dans un ensemble extrémal $E: \mathrm{1}^{\circ}$ est bornée dans cet ensemble; $2^{\circ}$ atteint en au moins un élément de cet ensemble sa limite supérieure, et en au moins un élément de cet ensemble sa limite inférieure.}

Ainsi, lorsqu'un ensemble $E$ est extrémal, toute opération continue y atteint chacun de ses extrema. C'est cette circonstance qui nous a fait adopter la dénomination d'ensemble extrémal qui se trouve encore justifiée par la suite ($\mathrm{n}^{\circ}$ 51).

On peut donner un corollaire plus étendu en un certain sens que le corollaire précédent en considérant les opérations semi-continues supérieurement \footnote{Cette définition est une généralisation de celle qui a été proposée par M. \textsc{Baire} (\textsc{iii}, page 71) pour les ensembles ponctuels.}. Nous dirons qu'une opération $U$ uniforme dans un ensemble $E$ est semi-continue supérieurement dans $E$ si, quel que soit l'élément $A$ de $E$ limite d'une suite d'éléments de $E$ distincts : $A_{1}, A_{2}, A_{3}, \ldots, A_{n}, \ldots, U(A)$ est au moins égal à la plus grande des limites \footnote{Étant donnée une suite infinie de nombres $u_{1}, u_{2}, \ldots, u_{n}, \ldots$, la plus grande des limites de cette suite est un nombre $\lambda$ tel que, quel que soit $\varepsilon$, on puisse trouver un entier $p$ de façon que l'on ait $u_{n}<\lambda+\varepsilon$ pour $n>p$ et qu'il existe un entier $m>p$ pour lequel $u_{m}>\lambda-\varepsilon$. S'il n'y a aucun nombre $\lambda$ satisfaisant à ces conditions, on dit que la plus grande des limites est infinie.} de la suite $U\left(A_{1}\right), U\left(A_{2}\right), U\left(A_{3}\right), \ldots, U\left(A_{n}\right), \ldots$.

\textsc{\textbf{Corollaire.}}---\textit{Toute opération semi-continue supérieurement dans un ensemble extrémal $E$: $1^{\circ}$ est bornée supérieurement dans $E$; $2^{\circ}$ atteint en au moins un élément de $E$ sa limite supérieure \footnote{Ce théorème est utilisé par exemple dans la recherche des géodésiques, car la longueur d'une courbe est une fonction semi-continue inférieurement de la courbe elle-même (n$^{\circ}\, 95$). (Voir aussi \textsc{xvii}).}.}

La démonstration est la même que précédemment; mais on ne peut plus rien dire sur la limite inférieure.\\

\textbf{12.} 
\textsc{\textbf{Théorème.}} --- \textit{Si $U$ est une opération continue dans un ensemble continu $E, U$ prend en au moins un élément de $E$ toute valeur comprise entre deux quelconques des valeurs prises par $U$.}

J'appelle ensemble continu, un ensemble tel qu'étant donnés deux quelconques de ses éléments $A, B$, on peut extraire de $E$ un ensemble $F$ dont chaque élément correspond à un point de l'intervalle $(0,1)$ sur un axe o$t$ et inversement. La correspondance est supposée telle que si deux éléments $A_{1}, A_{2}$ de $F$ correspondent à deux points $t_{1}, t_{2}, A_{1}$ tend vers $A_{2}$ quand $t_{1}$ tend vers $t_{2}$. Le théorème précédent a été démontré pour les fonctions de lignes par M. \textsc{Arzelà} (\textsc{v}, page 348). Sa démonstration se généralise immédiatement au cas actuel et revient à considérer dans $F$, l'opération $U$ comme une fonction de $t$.

\subsection*{Les séries d'opérations continues.}

\textbf{13.}
\textit{\textbf{Convergence uniforme et quasi-uniforme.}} --- Considérons une suite d'opérations continues dans un même ensemble $E$; soient:
$$
U_{1}, U_{2}, U_{3}, \ldots, U_{n}, \ldots
$$

Lorsque cette suite est convergente en tout point de $E$, la limite définit une opération uniforme dans $E$, soit $U$. Il est souvent utile de savoir si cette limite est ou non une opération continue dans $E$. Il n'y a aucune raison pour qu'il en soit toujours ainsi.

Un cas très général où l'on est assuré de la continuité de $U$ est celui où la convergence de la suite est uniforme. Nous dirons qu'une suite d'opérations quelconques uniformes dans $E$ \textit{converge uniformément} dans $E$ vers une opération $U$ si, quel que soit le nombre $\varepsilon>0$, on peut trouver un entier $p$ tel que $n>p$ entraîne $\left|U_{n}(A)-U(A)\right|<\varepsilon$ en tout élément $A$ de $E$.

On démontre facilement que si une suite d'opérations $U_{1}, U_{2}, \ldots$, continues dans un ensemble quelconque $E$ converge uniformément vers une opération $U$, celle-ci est continue dans $E$.\\

\textbf{14.}
Mais la limite peut être continue sans que la convergence soit uniforme. On a donc été amené à chercher une condition moins restrictive pour la convergence. M. \textsc{Arzelà} est parvenu à résoudre le problème par l'introduction de la convergence quasi-uniforme. Sa démonstration assez compliquée ne s'applique qu'aux fonctions d'une variable (\textsc{ix}). Mais M. \textsc{Borel} a donné ensuite une démonstration plus simple (\textsc{ii}, page 42) qui se généralise immédiatement aux ensembles d'éléments d'une classe ($L$) avec une légère modification nécessitée par notre hypothèse plus générale.

Nous dirons qu'une suite d'opérations $U_{1}, U_{2}, \ldots, U_{n}, \ldots$, uniformes dans un ensemble $E$ \textit{converge quasi-uniformément} vers une opération $U$, lorsque, étant donnés le nombre $\varepsilon>0$ et un entier quelconque $N$, on peut déterminer, une fois pour toutes, un entier $N^{\prime} \geqslant N$ tel que, à tout élément $A$ de $E$, on puisse faire correspondre un entier $n_{A}$ tel que
$$
N \leqslant n_{A} \leqslant N^{\prime}, \quad\left|U(A)-U_{n_{A}}(A)\right|<\varepsilon\,.
$$

Lorsqu'il y a convergence uniforme, il y a aussi convergence quasi-uniforme. Dès lors, le théorème que nous avons énoncé plus haut est une conséquence du suivant:

\textit{Lorsqu'une suite d'opérations $U_{1}, U_{2}, \ldots, U_{n}, \ldots$ continues dans un ensemble quelconque formé d'éléments d'une classe ($L$) converge quasi-uniformément dans $E$ vers une opération $U$, celle-ci est continue dans $E$.} La démonstration est la généralisation directe de celle de M. \textsc{Borel} (\textsc{ii}, page 42). Ce théorème admet une réciproque, mais celle-ci ne s'applique qu'à un ensemble $E$ extrémal.

Il suffit de généraliser la seconde démonstration de M. \textsc{Borel} (\textsc{ii}, page 43-44); cependant, pour démontrer qu'une certaine quantité $n_{A}$ déterminée en tout élément $A$ de $E$ est bornée dans $E$, il est impossible de diviser comme lui en intervalles de longueurs décroissantes. Mais si $n_{A i}$ n'est pas borné, on peut former, \textit{puisque $E$ est extrémal}, une suite d'éléments de $E: A_{1}, A_{2}, A_{3}, \ldots$ qui tendent vers un élément de $E$ et tels que $n_{A_{p}}$ tende vers l'infini avec $p$. Le reste de la démonstration s'ensuit.

On peut cependant donner un énoncé de la réciproque applicable à un ensemble quelconque. En la combinant avec le théorème direct, on obtient la proposition suivante:

\textit{Pour qu'une suite d'opérations $U_{1}, U_{2}, \ldots, U_{n}, \ldots$ continues dans un même ensemble $E$ formé d'éléments d'une classe ($L$) converge vers une opération continue dans $E$, il faut et il suffit que cette suite converge quasi-uniformément dans tout ensemble extrémal formé d'éléments de $E$.}

Il suffit de montrer que si un élément $A$ de $E$ est limite d'une suite d'éléments de $E: A_{1}, A_{2}, \ldots, A_{n}, \ldots$, on a:
$$
U(A)=\lim _{n=\infty} U\left(A_{n}\right)
$$

Or l'ensemble $F$ formé des éléments $A, A_{1}, A_{2}, \ldots$ est extrémal. On peut donc lui appliquer la réciproque déjà démontrée dans ce cas.\\

\textbf{15.} 
\textit{\textbf{Les opérations également continues.}} --- Considérons une famille $\mathfrak{F}$ d'opérations continues dans un même ensemble $E$ formé d'éléments d'une classe ($L$). Dans un grand nombre de questions de l'Analyse, il serait utile de savoir si la famille $\mathfrak{F}$ est telle que de toute infinité d'opérations de $\mathfrak{F}$ distinctes, on peut tirer une suite $U_{1}, U_{2}, \ldots$, $U_{n}, \ldots$ qui converge uniformément vers une limite $U$ nécessairement continue dans $E$. Nous dirons qu'une telle famille $\mathfrak{F}$ est \textit{compacte}.

M. \textsc{Arzelà} qui a montré comment le fait de savoir qu'une famille est compacte simplifierait bien des démonstrations de l'Analyse, est parvenu à résoudre cette question dans le cas où les éléments de $E$ sont des nombres (\textsc{v}, page 1).

Il utilise pour cela la notion d'\textit{égale continuité} introduite par M. \textsc{Ascoli} (\textsc{xxii}). Comme nous nous plaçons à un point de vue bien plus général que ces deux auteurs, nous allons donner une définition de l'égale continuité indépendante de la notion d'intervalle. Nous reconnaîtrons ensuite qu'elle coïncide avec la définition de M. \textsc{Arzelà} dans les ensembles considérés par lui. La démonstration de M. \textsc{Arzelà} est compliquée et ne se généralise pas à notre point de vue actuel. Nous donnerons une démonstration différente dont la marche générale est au fond la même que celle de M. \textsc{Hilbert} pour l'existence des géodésiques (\textsc{xx}). Mais M. \textsc{Hilbert} n'avait pas vu que sa \textit{méthode} pouvait se généraliser beaucoup plus loin que celle de M. \textsc{Arzelà}, tandis que son \textit{résultat} est au contraire une conséquence immédiate du théorème de M. \textsc{Arzelà}.

Nous dirons que des opérations uniformes dans un même ensemble $E$ formé d'éléments d'une classe $(L)$, constituent une famille $\mathfrak{F}$ d'opérations également continues en $A$ dans $E$, si, étant donné un nombre $\varepsilon>0$ et une suite quelconque d'éléments de $E$ : $A_{1}, A_{2}, \ldots, A_{n}, \ldots$, ayant pour limite un élément $A$ de $E$, on peut trouver un entier $p$ tel que l'inégalité $n>p$ entraîne
$$
\left|U(A)-U\left(A_{n}\right)\right|<\varepsilon,
$$
quelle que soit l'opération $U$ de la famille $\mathfrak{F}$.

Il est d'ailleurs bien entendu que le nombre $p$ indépendant de $U$ peut au contraire varier avec la suite $A_{1}, A_{2}, \ldots, A_{n}, \ldots$. Il résulte immédiatement de la définition, et comme il le fallait, que des opérations \textit{également continues} dans $E$ sont en particulier chacune continue dans $E$. Inversement, si des opérations \textit{en nombre fini} sont continues dans $E$, elles sont \textit{également continues} dans $E$. Mais cette remarque n'est plus exacte pour une infinité d'opérations distinctes.

Pour arriver au but que nous nous sommes proposé, nous démontrerons une série de propositions intéressantes en elles-mêmes, mais impliquant pour $E$ et $\mathfrak{F}$ des hypothèses différentes. En les combinant dans le cas où toutes ces hypothèses sont simultanément réalisées, on obtient le résultat cherché.\\

\textbf{16.} 
\textsc{\textbf{$1^{\text {er }}$ Lemme.}} --- La limite $U$ d'une suite convergente $U_{1}, U_{2}, \ldots, U_{n}, \ldots$ d'opérations également continues dans un ensemble $E$, est une opération continue dans $E$. De plus, si $E$ est extrémal, la convergence est nécessairement uniforme dans $E$.

En effet, si on considère un élément quelconque $A$ de $E$, limite d'une suite d'éléments de $E: A_{1}, A_{2}, \ldots, A_{n}, \ldots$, on a
$$
\left|U_{q}(A)-U_{q}\left(A_{n}\right)\right|<\varepsilon, \text { pour } n>p,
$$
quel que soit $q$. Si on fait croître $q$ indéfiniment, on aura à la limite
$$
\left|U(A)-U\left(A_{n}\right)\right| \leqslant \varepsilon, \text { pour } n>p \, .
$$

Cela prouve que $U$ est continue en tout élément $A$ de $E$.

De plus, on voit que si les opérations d'une famille $\mathfrak{F}$ sont également continues dans $E$, il en sera de même des opérations de la famille $\mathfrak{F}_1$, formée par l'ensemble de opérations limites dans $E$ d'une suite infinie d'opérations de $\mathfrak{F}$ (s'il y en a).

Supposons maintenant que $E$ soit un ensemble extrémal. Si des opérations également continues $U_{1}, U_{2}, \ldots$ convergent vers une limite $U$ dans un ensemble extrémal $E$, la convergence est nécessairement uniforme. Sans quoi, on pourrait trouver un nombre $\varepsilon>0$ tel que, quel que soit $n$, il y ait un élément $A_{n}$ de $E$ et un entier $p_{n}>n$ pour lesquels
$$
\left|U_{p_{n}}\left(A_{n}\right)-U\left(A_{n}\right)\right|>\varepsilon ;
$$
et puisque $E$ est extrémal, on peut supposer que $A_{1}, A_{2}, \ldots$ tendent vers un élément $A$ de $E$. On aura donc:
$$\left|U_{p_{n}}\left(A_{n}\right)-U\left(A_{n}\right)\right| \leqslant\left|U_{p_{n}}\left(A_{n}\right)-U_{p_{n}}(A)\right|+\left|U(A)-U\left(A_{n}\right)\right|+\left|U(A)-U_{p_{n}}(A)\right|.$$
Puisque $U_{p_{n}}(A)$ tend vers $U(A)$ et que les opérations $U_{1}, U_{2}, \ldots$ sont également continues, on pourra trouver $k^{\prime}$ et $k^{\prime \prime}$ de façon que le dernier terme soit inférieur à $\displaystyle \cfrac{\varepsilon}{3}$ pour $n>k^{\prime}$ et que les deux premiers soient inférieurs chacun à $\displaystyle \cfrac{\varepsilon}{3}$ pour $n>k^{\prime \prime}$. On aura donc pour $n>k^{\prime}+k^{\prime \prime}$ :
$$
\left|U_{p_{n}}\left(A_{n}\right)-U\left(A_{n}\right)\right| \leqslant \varepsilon .
$$

Nous arrivons donc bien à une contradiction.\\

\textbf{17.} 
\textsc{\textbf{$2^{\text {ème }}$ Lemme.}} --- Considérons une suite d'opérations $U_{1}, U_{2}, \ldots$ convergente dans un ensemble $D$. Si ces opérations sont également continues dans l'ensemble $F$ formé des éléments de $D$ et de son ensemble dérivé $D^{\prime}$, la suite considérée est aussi convergente dans $F$.

Il suffit de démontrer que la suite est convergente en tout élément $A$ limite d'une suite d'éléments de $D: A_{1}, A_{2}, \ldots, A_{n}, \ldots$ Or, on peut, étant donné $\varepsilon>0$, trouver $p$ tel que:
$$
\left|U_{q}(A)-U_{q}\left(A_{n}\right)\right|<\cfrac{\varepsilon}{3},
$$
pour $n>p$, quel que soit $q$, puisque les opérations sont également continues. Prenons une valeur déterminée de $n>p$, par exemple $n=p+1$. Puisque la suite $U_{1}\left(A_{p+1}\right), U_{2}\left(A_{p+1}\right), \ldots$ est convergente, on peut trouver un entier $r$ tel que l'on ait:
$$
\left|U_{r+k}\left(A_{p+1}\right)-U_{r}\left(A_{p+1}\right)\right|<\cfrac{\varepsilon}{3},
$$
quel que soit $k$.

Alors on aura, quel que soit l'entier $k$,
$$
\begin{aligned}
\left|U_{r+k}(A)-U_{r}(A)\right| \leqslant & \left|U_{r+k}(A)-U_{r+k}\left(A_{p+1}\right)\right|+\left|U_{r+k}\left(A_{p+1}\right)-U_{r}\left(A_{p+1}\right)\right| \\
& +\left|U_{r}\left(A_{p+1}\right)-U_{r}(A)\right|<\varepsilon .
\end{aligned}
$$

D'après un théorème de \textsc{Cauchy}, cela prouve que la suite $U_{1}(A), U_{2}(A), \ldots$ est convergente.\\

\textbf{18. \textsc{$3^{\text {ème }}$ Lemme.}} --- Pour que des opérations continues dans un même ensemble extrémal $E$ forment une famille compacte $\mathfrak{F}$, il faut qu'elles soient également continues et bornées dans leur ensemble.

Si ces opérations n'étaient pas bornées dans leur ensemble, il y en aurait une: $U_{n}$ quel que soit $n$, dont la valeur absolue serait supérieure à $n$ en quelque élément $A_{n}$ de $E$.

Puisque la famille $\mathfrak{F}$ est compacte, on peut supposer que $U_{1}, U_{2}, \ldots$ convergent uniformément vers une opération $U$ continue dans $E$, et que $U_{n}\left(A_{n}\right)$ tend encore vers l'infini. Alors on aura
$$
\left|U_{n}\left(A_{n}\right)\right| \leqslant\left|U_{n}\left(A_{n}\right)-U\left(A_{n}\right)\right|+\left|U\left(A_{n}\right)\right| .
$$

Lorsque $n$ croît indéfiniment, le premier terme du second membre tend vers zéro; le second reste fini puisque $U$ est une opération continue dans un ensemble extrémal ($\mathrm{n}^{\circ}$ 11). Il est donc impossible que le premier membre croisse indéfiniment.

De même, si les opérations de $\mathfrak{F}$ n'étaient pas également continues, on pourrait trouver une suite d'éléments de $E: A_{1}, A_{2}, \ldots$, tendant vers un élément $A$ de $E$, et un nombre $\varepsilon$ tels que, quel que soit $n$, il existe une opération de $\mathfrak{F}$ : $U_{n}$ et un entier $p_{n}>n$ pour lesquels:
$$
\left|U_{n}(A)-U_{n}\left(A_{p_{n}}\right)\right|>\varepsilon .
$$

Comme la famille $\mathfrak{F}$ est compacte, on peut dire en somme qu'il existe une suite d'éléments de $E: A_{1}^{\prime}, A_{2}^{\prime}, \ldots$ tendant vers un élément $A$ de $E$, et une suite d'opérations de $\mathfrak{F}$: $U_{1}^{\prime}, U_{2}^{\prime}, \ldots$ qui convergent uniformément vers une opération $U$, de façon que l'on ait:
$$
\left|U_{n}^{\prime}(A)-U_{n}^{\prime}\left(A_{n}^{\prime}\right)\right|>\varepsilon .
$$
(Il suffit d'extraire convenablement ces deux suites des suites $A_{p_{1}}, A_{p_{2}}, \ldots$ et $U_{1}, U_{2}, \ldots$ ).

Mais alors:
$$
\left|U_{n}^{\prime}(A)-U_{n}^{\prime}\left(A_{n}^{\prime}\right)\right| \leqslant\left|U\left(A_{n}^{\prime}\right)-U_{n}^{\prime}\left(A_{n}^{\prime}\right)\right|+\left|U_{n}^{\prime}(A)-U(A)\right|+\left|U(A)-U\left(A_{n}^{\prime}\right)\right|
$$
et, prenant $n$ assez grand, on voit comme précédemment qu'on pourra rendre le second membre inférieur à $\varepsilon$, d'où la contradiction annoncée.

Afin d'arriver au théorème général, j'énoncerai une dernière proposition qui est démontrée plus loin sous une autre forme ($\mathrm{n}^{\circ}$ 66).

Si l'on considère pour chaque valeur entière de $n$, une suite infinie $S_{n}$ de nombres $x_{1}^{(n)}, x_{2}^{(n)}, \ldots x_{p}^{(n)}, \ldots$, compris pour chaque valeur de $p$, quel que soit $n$, entre deux nombres fixes $\lambda_{p}$ et $\mu_{p}$, on peut extraire de la suite $S_{1}, S_{2}, \ldots$ une suite $S_{n_{1}}, S_{n_{2}}, \ldots$ d'indices croissants tels que $x_{p}^{\left(n_{q}\right)}$ tende vers une limite $x_{p}$, quel que soit le nombre fixe $p$ quand $n_{q}$ croît indéfiniment.\\

\textbf{19.} 
Nous sommes maintenant en mesure d'énoncer le théorème général suivant:

\textsc{\textbf{Théorème.}} --- \textit{Pour que des opérations continues dans un même ensemble extrémal $E$ formé d'éléments d'une classe ($L$), qui appartiennent à un même ensemble dénombrable $D$ ou à son dérivé $D^{\prime}$, forment une famille compacte $\mathfrak{F}$, il faut et il suffit que les opérations de $\mathfrak{F}$ soient également continues et bornées dans leur ensemble en tout élément de $E$.}

La condition est nécessaire d'après le dernier Lemme. Pour démontrer qu'elle est suffisante, il suffit de démontrer que, de toute suite infinie d'opérations de $\mathfrak{F}: U_{1}, U_{2}, \ldots$ on peut extraire une suite qui converge uniformément dans $E$ vers une opération qui sera nécessairement continue dans $E$.

En effet, appelons $A_{1}, A_{2}, \ldots$ la suite des éléments de l'ensemble dénombrable $D$ et considérons la suite $S_{n}$ des nombres $x_{1}^{(n)}=U_{n}\left(A_{1}\right), \ldots, x_{p}^{(n)}=U_{n}\left(A_{p}\right), \ldots$ Puisque les opérations de $\mathfrak{F}$ sont bornées dans leur ensemble en tout élément de $D$, ces nombres $x_{p}^{(n)}$ sont, pour chaque valeur de $p$, compris, quel que soit $n$, entre deux nombres fixes $\lambda_{p}$ et $\mu_{p}$. D'après la dernière proposition que nous avons rappelée, on pourra donc extraire de la suite $S_{1}, S_{2}, \ldots$ une suite $S_{n_{1}}, S_{n_{2}}, \ldots$ d'indices croissants, telle que $x_{p}^{\left(n_{q}\right)}=U_{n_{q}}\left(A_{p}\right)$ converge vers une certaine limite $x_{p}$ et cela quel que soit $p$. Cela veut dire qu'on peut extraire de la suite $U_{1}, U_{2}, \ldots$ une suite d'opérations $U_{n_{1}}, U_{n_{2}}, \ldots, U_{n_{q}}, \ldots$ convergente en tout élément de $D$.

D'après le deuxième Lemme, cette suite d'opérations sera aussi convergente en tout élément de $E$; d'après le premier Lemme la convergence sera uniforme, et par suite la limite continue dans $E$.

\textsc{\textbf{1$^\text{ére}$ Remarque.}} --- Si l'on ne suppose plus que l'ensemble $E$ est extrémal, la démonstration précédente prouve encore quelque chose. Elle prouve que si les opérations de $\mathfrak{F}$ sont également continues et bornées dans leur ensemble en tout élément de $E \equiv D+D^{\prime}$, on pourra extraire de toute infinité d'opérations de $\mathfrak{F}$ une suite qui tend vers une opération continue dans $E$. Mais on ne saura pas si la convergence est uniforme. D'ailleurs, on peut citer des exemples où, dans ces conditions, la convergence est non uniforme. Elle sera toujours uniforme dans tout ensemble extrémal contenu dans $E$.

\textsc{\textbf{$2^{\text {ème }}$ Remarque.}} --- Il pourrait sembler que la condition $E \equiv D+D^{\prime}$, où $D$ est dénombrable, est une condition introduite artificiellement dans le seul but d'assurer l'exactitude du résultat. Nous verrons plus loin que c'est au contraire le cas général qui se présente dans les applications ($\mathrm{n}^{\mathrm{os}}$ 45, 52).\\

\textbf{20.} 
\textbf{\textit{L'opération limite supérieure d'un ensemble d'opérations.}} --- Considérons une famille $\mathfrak{F}$ d'opérations uniformes dans un ensemble $E$. En chaque élément $A$ de $E$, nous pouvons définir un nombre $L(A)$ qui soit la limite supérieure des valeurs en $A$ des opérations de $\mathfrak{F}$. Si les opérations de $\mathfrak{F}$ sont bornées dans leur ensemble en tout élément de $E$, nous déterminerons ainsi une opération uniforme dans $E$, que nous appellerons la limite supérieure de $\mathfrak{F}$.

\textsc{\textbf{Théorème.}} --- \textit{Étant donnée une famille $\mathfrak{F}$ d'opérations bornées dans leur ensemble et également continues dans un ensemble quelconque $E$, la limite supérieure de $\mathfrak{F}$ est une opération continue dans $E$.}

Ce théorème a été démontré par M. \textsc{Arzelà} (\textsc{v}, page 9) dans le cas où les éléments sont des points d'une droite. Sa démonstration se généralise immédiatement au cas actuel en se souvenant que notre définition de la continuité rend inutile l'emploi des intervalles.\\

\textbf{21.} 
\textsc{\textbf{Remarque.}} --- Nous avons vu dans ce qui précède comment on peut arriver à généraliser certains théorèmes connus dans les classes si étendues que nous avons appelées classes $(L)$. Néanmoins le petit nombre des hypothèses que nous avons faites sur les classes ($L$) ne nous permettra pas de poursuivre cette extension. On s'aperçoit bien vite que certaines propositions fondamentales de la théorie des ensembles linéaires et des fonctions continues, dont l'énoncé mis sous forme convenable peut garder un sens pour les classes $(L)$, que ces propositions, dis-je, ne sont plus vraies pour toute classe ($L$). Par là-même échoue toute tentative de généralisation des propositions ultérieures auxquelles elles servent de base.

\subsection*{Les ensembles dérivés.}

\textbf{22.}
Nous donnerons en exemple l'une des plus importantes d'entre elles: l'ensemble dérivé d'un ensemble linéaire est fermé. Cette proposition est elle applicable à des ensembles d'éléments d'une classe ($L$) quelconque? \textit{La réponse est négative.}

Considérons en effet la classe ($C$) des fonctions d'une variable $x$ définies dans un intervalle fixe $J: 0 \leqslant x \leqslant 1$ et convenons de dire qu'une suite de telles fonctions : $f_{1}(x), f_{2}(x), \ldots$ tend vers une fonction $f(x)$ si, pour chaque valeur $x$ de l'intervalle $J$, $f_{n}(x)$ a une limite finie $f(x)$. Cette définition satisfait bien aux conditions I et II du n$^{\circ}$ 7. Donc cette classe ($C$) est une classe ($L$). Cependant l'ensemble dérivé d'un ensemble quelconque d'éléments de la classe ($C$) n'est pas nécessairement fermé.\\

{
\small 

\footnote{Dans la \textsc{Première Partie}, les sujets qui exigent des connaissances un peu spéciales sont imprimés en petits caractères.} Il suffit de considérer l'ensemble $E$ des fonctions continues dans $J$. L'ensemble $E^{\prime}$ des fonctions limites de fonctions continues est l'ensemble des fonctions de classes 0 ou 1 au sens de M. \textsc{Baire} (\textsc{iii}, page 126). Or on sait qu'il y a des fonctions de classe 2 (même citation), c'est-à-dire qu'il y a des fonctions limites de fonctions de $E^{\prime}$ et n'appartenant pas à $E$.

\textbf{23.} 
\textit{\textbf{Limites de fonctions limites.}} --- Nous nous écarterons un moment de notre sujet pour signaler une proposition à laquelle l'exemple précédent donne un certain intérêt.

Considérons un ensemble de fonctions $f_{n}^{(p)}(x)$ définies dans l'intervalle $J$ et telles que: $1^{\circ}$ la suite:
$$
f_{n}^{(1)}(x), \quad f_{n}^{(2)}(x), \quad \ldots \quad f_{n}^{(p)}(x), \quad \ldots
$$
ait une limite déterminée $f_{n}(x)$ et ceci quel que soit $n$; $2^{\circ}$ la suite:
$$
f_{1}(x), f_{2}(x), \ldots, f_{n}(x), \ldots
$$
ait une limite déterminée $f(x)$.

D'après ce qui précède, il ne sera pas toujours possible de trouver deux suites d'entiers $n_{1}$, $n_{2}, \ldots, p_{1}, p_{2}, \ldots$ telles que l'on ait: $\displaystyle f(x)=\lim _{r=\infty} f_{n_{r}}^{\left(p_{r}\right)}(x)$.

Cette remarque justifie l'intérêt qui s'attache au théorème suivant:

\textsc{\textbf{Théorème.}} --- Considérons des fonctions $f_{n}^{(p)}(x), f_{n}(x), f(x)$ définies dans un mime intervalle $J$, quels que soient les entiers $n, p$ et telles que:
\begin{equation*}
f(x)=\lim _{n=\infty} f_{n}(x), \quad f_{n}(x)=\lim _{p=\infty} f_{n}^{(p)}(x) . \tag{ \textsc{i}}
\end{equation*}

S'il est en général impossible de choisir des entiers $n_{r}, p_{r}$ tels que l'égalité
$$
f(x)=\lim _{r=\infty} f_{n_{r}}^{\left(p_{r}\right)}(x)
$$
soit vérifiée en tout point de $J$, du moins est-il toujours possible de les déterminer de façon que cette égalité soit vérifiée en tout point de $J$ sauf en un ensemble de points de mesure nulle\footnote{Voir pour la signification de cette expression: \textsc{ii}, page 16}.

Pour le démontrer, je m'appuierai sur deux remarques préliminaires : $1^{\circ}$ Supposons pour simplifier que l'intervalle $J$ soit l'intervalle $(0,1)$ : Si on considère une suite d'ensembles de points de $J$ : $E_{1}$, $E_{2}, \ldots$ ayant pour mesures $1-m_{1}, 1-m_{2}, \ldots$, l'ensemble des points communs à tous ces ensembles a une mesure au moins égale à $1-\left(m_{1}+m_{2}+\ldots\right)$. $2^{\circ}$ M. \textsc{Borel} a démontré (\textsc{ii}, page 37) que, quel que soit le nombre fixe $\varepsilon>0$, l'ensemble de points où le reste de rang $n$ d'une série convergente de fonctions de $x$ dans $J$ est en valeur absolue plus grand que $\varepsilon$, est un ensemble dont la mesure tend vers zéro avec $\cfrac{1}{n}$.

Soient alors $\varepsilon$ et $\sigma$ deux nombres quelconques compris entre 0 et 1 ; on peut trouver un entier $q$ tel que la mesure de l'ensemble de points où $\left|f-f_{n}\right|<\cfrac{\varepsilon}{2}$ soit supérieure à $1-\cfrac{\sigma}{2}$ pour $n>q-1$. Puis, on pourra trouver, $q$ étant fixé, un nombre $r$ tel que la mesure de l'ensemble des points où $\left|f_{q}-f_{q}^{(r)}\right|<\cfrac{\varepsilon}{2}$ soit aussi supérieure à $1-\cfrac{\sigma}{2}$. 
En tout point commun aux deux ensembles précédents, on aura $\left|f-f_{q}^{(r)}\right|<\varepsilon$ et l'ensemble de ces points communs a une mesure au moins égale à $1-\left(\cfrac{\sigma}{2}+\cfrac{\sigma}{2}\right)=1-\sigma$. Il en est donc de même a fortiori de l'ensemble des points tels que $\left|f-f_{q}^{(r)}\right|<\varepsilon$.

Ceci étant, donnons à $\varepsilon$ et $\sigma$ deux suites successives de valeurs $\varepsilon_{1}, \varepsilon_{2}, \ldots ; \sigma_{1}, \sigma_{2}, \ldots$ Quel que soit $r$, on pourra déterminer des entiers $n_{n}, p_{r}$ tels que l'ensemble $G_{r}$ des points où l'on a $\left|f-f_{n_{r}}^{\left(p_{r}\right)}\right|<\varepsilon_{r}$ ait une mesure supérieure à $1-\sigma_{r}$. 
Appelons maintenant $H_{r}$ l'ensemble des points communs à $G_{r}, G_{r+1}, G_{r+2}, \ldots, G_{r+n}, \ldots$. 
Sa mesure est au moins égale à $1-\left(\sigma_{r}+\sigma_{r+1}+\ldots\right)$ et en chacun de ses points on a $\left|f-f_{n_{r+q}}^{\left(p_{r+q}\right)}\right|<\varepsilon_{r+q}$, quel que soit l'entier $q$.

Or supposons qu'on ait choisi, comme cela est possible, les nombres $\varepsilon_{r}$, $\sigma_{r}$ de façon que les $\varepsilon_{r}$ tendent en décroissant vers zéro et que la série $\sigma_{1}+\sigma_{2}+\ldots$ soit convergente. Par exemple, admettons qu'on ait $\varepsilon_{r}=\sigma_{r}=\cfrac{1}{r^{2}}$. Alors on voit qu'on aura en tous les points de $H_{r}:\left|f-f_{n_{r+q}}^{\left(p_{r+q}\right)}\right|<\cfrac{1}{(r+q)^{2}}$ quel que soit $q$, donc en tout point de $H_{r}$ la suite $f_{n_{1}}^{\left(p_{1}\right)}, f_{n_{2}}^{\left(p_{2}\right)}, \ldots$ converge vers $f$. Dès lors, l'ensemble $H$ des points où cette suite converge a une mesure au moins égale à celle de $H_{r}$ quel que soit $r$, c'est-à-dire au moins égale à $1-\left(\cfrac{1}{r^{2}}+\cfrac{1}{(r+1)^{2}}+\cdots\right)$, quel que soit $r$. Autrement dit, l'ensemble $H$ a même mesure que $J$.\\

\textbf{24.} 
\textsc{\textbf{Remarques.}} --- 1$^{\circ}$ Il y a un cas particulier important, où on peut s'arranger pour que l'ensemble $H$ \textit{coïncide} avec l'intervalle $J$. C'est celui où $f_{n}^{(p)}(x)$ tend \textit{uniformément} vers $f_{n}(x)$, quel que soit $n$. En effet, dans ce cas, on peut choisir pour toute valeur de $n$ un entier $p_{n}$ tel que l'on ait:
$$
f_{n}(x)=f_{n}^{\left(p_{n}\right)}(x)+\cfrac{\varepsilon_{n}(x)}{n} \, \text { avec } \, \left|\varepsilon_{n}(x)\right|<1 \,,
$$
quel que soit $x$. Alors on aura:
$$
f(x)=\lim _{n=\infty} f_{n}(x) \quad \text { et } \quad 0=\lim _{n=\infty} \cfrac{\varepsilon_{n}(x)}{n},
$$
d'où:
$$
f(x)=\lim _{n=\infty} f_{n}^{\left(p_{n}\right)}(x)
$$

$2^{\circ}$ Si les égalités (\textsc{i}) n'étaient pas vérifiées nécessairement partout, mais l'étaient chacune dans un ensemble de mesure $\geqslant m$ ($m$ nombre fixe), on pourrait s'arranger pour que l'ensemble $H$ fut aussi de mesure $\geqslant m$. En particulier, si les égalités (\textsc{i}) étaient chacunes vérifiées sauf dans un ensemble de mesure nulle, la démonstration précédente prouverait encore qu'on peut s'arranger pour que $H$ coïncide avec $J$ sauf en un ensemble de mesure nulle.

Appliquons la remarque $1^{\circ}$ en prenant pour les $f_{n}(x)$ des fonctions continues quelconques. 
On sait qu'on pourra prendre pour les $f_{n}^{(p)}(x)$ des polynômes avec convergence uniforme de $f_{n}^{(p)}$ vers $f_{n}$. Donc, d’après $1^{\circ}$ les fonctions limites de fonctions continues sont aussi limites de polynômes. Appliquons maintenant notre théorème en prenant pour $f_{n}$ une fonction de première classe; d'après ce que nous venons de dire, on pourra prendre pour les $f_{n}^{(p)}$ des polynômes. Donc les fonctions de classe 2 sont limites de polynômes sauf en un ensemble de mesure nulle. Appliquons maintenant la remarque $2^{\mathrm{o}}$ en prenant pour $f_{n}$ une fonction de classe 2. D'après ce qui précède, on pourra prendre pour les $f_{n}^{(p)}$ des polynômes, la convergence ayant lieu dans $J$ sauf en un ensemble de mesure nulle. Donc les fonctions de classe 3 sont aussi des limites de polynômes sauf en un ensemble de mesure nulle. Plus généralement, \textit{toute fonction $f(x)$ rentrant dans la classification de M. \textsc{Baire} (\textsc{iii}, page 126) peut être considérée comme la limite d'une suite de polynômes sauf en un ensemble de mesure nulle}\footnote{J'ai énonce ce théorème dans les Comptes Rendus du 20 mars 1905: \textit{Sur la notion d'écart dans le calcul fonctionnel.} M. \textsc{Lebesgue} a obtenu ce même théorème comme application de sa définition de l'intégrale.}. Si la suite de polynômes converge partout, $f(x)$ est de classe 0 ou 1. Si la suite des polynômes converge partout uniformément, $f(x)$ est de classe 0; c'est-à-dire continue. Il suffit même que la convergence ait lieu partout quasi-uniformément.
}

\section*{Chapitre II.}
\subsection*{Définition de la limite par le voisinage.}

\textbf{25.}
Nous avons déjà remarqué plus haut que l'extrême généralité des classes ($L$) ne permet pas de leur étendre un grand nombre des propriétés des ensembles linéaires. Pour obtenir des propriétés plus nombreuses, il y aurait lieu d'imposer de nouvelles restrictions à la conception des classes ($L$). Il faudrait les choisir de façon à satisfaire aux conditions suivantes: $1^{\circ}$ ces restrictions devraient pouvoir s'énoncer indépendamment de la nature des éléments considérés; $2^{\circ}$ elles devraient être satisfaites par les classes d'éléments qui interviennent le plus fréquemment dans les applications; $3^{\circ}$ elles devraient fournir la généralisation cherchée des théorèmes sur les ensembles linéaires et les fonctions continues.\\

\textbf{26.}
Or nous avons observé ($\mathrm{n}^{\circ}$ 22) que si l'on considère une classe ($L$) quelconque, l'ensemble dérivé d'un ensemble d'éléments de cette classe n'est pas toujours fermé. C'est pourtant une propriété qu'il aurait été assez naturel d'admettre, en la traduisant sous la forme suivante: Lorsque des éléments $A_{1}, A_{2}, \ldots$ d'une classe ($L$) sont chacun limite d'une suite d'éléments (par exemple: $\displaystyle A_{n}=\lim _{p=\infty} A_{n}^{(p)}$) et tendent vers une limite $A$, cet élément $A$ est lui-même limite des derniers éléments (par exemple : $\displaystyle A=\lim _{q=\infty} A_{n_{q}}^{\left(p_{q}\right)}$). L'exemple que nous avons donné (n$^{\circ}$ 22) nous montre que cette propriété n'est pas une conséquence de la définition des classes ($L$). Il prouve aussi qu'elle peut n'être pas vérifiée, même parmi des classes ($L$) qui se présentent d'elles-mêmes dans la Théorie des Fonctions.\\

\textbf{27.}
Cependant la propriété précédente est compatible avec un grand nombre de définitions de la limite (particulièrement les limites dites uniformes). Il y aurait donc lieu, soit d'étudier ce qui se produit quand on impose cette propriété comme condition supplémentaire à la définition de la limite, soit d'introduire une condition supplémentaire qui entrainât cette propriété comme conséquence. Or l'examen des cas déjà connus où cette propriété a lieu nous montre que c'est cette dernière circonstance qui se produit sous la forme suivante:

Considérons une classe $(V)$ d'éléments de nature quelconque, mais tels qu'on sache discerner si deux d'entre eux sont ou non identiques et tels, de plus, qu'à deux quelconques d'entre eux $A, B$, on puisse faire correspondre un nombre $(A, B)=(B, A) \geqslant 0$ qui jouit des deux propriétés suivantes : $1^{\circ}$ La condition nécessaire et suffisante pour que ($A, B$) soit nul est que $A$ et $B$ soient identiques. $2^{\circ}$ Il existe une fonction positive bien déterminée $f(\varepsilon)$ tendant vers zéro avec $\varepsilon$, telle que les inégalités $(A, B) \leqslant \varepsilon$, $(B, C) \leqslant \varepsilon$ entraînent $(A, C) \leqslant f(\varepsilon)$, quels que soient les éléments $A, B, C$. Autrement dit, il suffit que $(A, B)$ et $(B, C)$ soient petits pour qu'il en soit de même de $(A, C)$. Nous appellerons \textit{voisinage} de $A$ et de $B$ le nombre $(A, B)$.

Ceci étant, nous pourrons dire qu'une suite d'éléments de la classe ($V$): $A_{1}, A_{2}, \ldots$ tend vers un élément $A$, si le voisinage $\left(A_{n}, A\right)$ tend vers zéro avec $\displaystyle\cfrac{1}{n}$. Si une suite $A_{1}, A_{2}, \ldots$ a une limite $A$, elle ne peut en avoir qu'une, car si $B$ était limite de la même suite, les nombres $\left(A, A_{n}\right)$ et $\left(B, A_{n}\right)$ seraient infiniment petits avec $\displaystyle\cfrac{1}{n}$, donc aussi $(A, B)$ ($2^{\text {ième }}$ condition). Alors $(A, B)$ serait nul et par suite les éléments $A, B$ ne seraient pas distincts ($1^{\text {ère }}$ condition).

De plus, cette définition de la limite satisfait bien aux conditions I et II que nous avons imposées en général à toute définition de la limite ($\mathrm{n}^{\circ}$ 7) et cela grâce aux conditions $1^{\circ}$ et $2^{\circ}$ imposées à la définition du voisinage.\\

\textbf{28.} 
Néanmoins toute définition de la limite satisfaisant aux conditions I et II, ne peut être déduite de la notion de voisinage. Il nous suffira pour le prouver de démontrer le théorème suivant.

\textsc{\textbf{Théorème.}} --- \textit{L'ensemble dérivé d'un ensemble d'éléments d'une classe ($V$) est un ensemble fermé.}

En effet, revenons aux notations employées plus haut. Puisqu'ici la limite est déduite du voisinage, on pourra faire correspondre à chaque entier $n$ un entier $q_{n}$ tel que $\displaystyle\left(A, A_{q_{n}}\right)<\cfrac{1}{n}$, et un entier $p_{n} \geqslant n$ tel que: $\displaystyle\left(A_{q_{n}}, A_{q_{n}}^{\left(p_{n}\right)}\right)<\cfrac{1}{n}$. On aura donc:
$$
\left(A, A_{q_{n}}^{\left(p_{n}\right)}\right)<f\left(\cfrac{1}{n}\right)
$$
et par suite $A_{q_{n}}^{\left(p_{n}\right)}$ tend vers $A$ quand $n$ tend vers l'infini.

Si maintenant nous revenons à l'exemple de la classe ($C$) donné plus haut, nous voyons qu'il fournit une classe ($L$) où il est impossible de construire une définition quelconque du voisinage telle que la définition de la limite qu'on en déduirait coïncide avec celle qui avait été adoptée. Car, en partant de cette dernière, on obtient un ensemble dérivé non fermé.

C'est donc vraiment se limiter que de considérer en particulier les classes ($V$) parmi les classes $(L)$ et nous pouvons espérer obtenir ainsi de nouvelles généralisations.

Nous nous bornerons donc maintenant à l'étude des classes ($V$), c'est-à-dire de celles des classes ($L$) où la définition de la limite est déduite de celle du voisinage.\\

\textbf{29.} \textsc{\textbf{Théorème.}} --- \textit{L'ensemble $P$ des éléments de condensation\footnote{Voir les définitions données plus haut ($\mathrm{n}^{\circ}$ 8). Nous verrons plus loin ($\mathrm{n}^{\circ}$ 43) un cas très général où un ensemble quelconque est toujours \textit{condensé}, c'est-à-dire qu'une infinité non dénombrable quelconque de ses éléments donne toujours lieu à au moins un élément de condensation.} d'un ensemble condensé $E$ formé d'éléments d'une classe} ($V$) \textit{est un ensemble parfait ou nul \footnote{La démonstration suivante est la généralisation de la démonstration récemment donnée par M. \textsc{Lindelöf} pour le cas où les éléments de $E$ sont des points de l'espace. Voir \textsc{Borel} (\textsc{ii}, pages 5, 6). Je n'ai insisté que sur les points de sa démonstration qui demandent quelques précautions pour être généralisés.}}.

En effet, on peut d'abord montrer que $P$ est un ensemble fermé sans supposer que $E$ soit condensé et même pour une classe ($L$) quelconque. Car si $A$ est un élément quelconque limite d'éléments $A_{1}, A_{2}, \ldots$ de $P$, c'est d'abord un élément limite de $E$ puisque $P$ est contenu dans $E^{\prime}$ qui est fermé d'après le théorème précédent. De plus, si l'on enlève de $E$ un ensemble dénombrable, les éléments $A_{1}, A_{2}, \ldots$ resteront éléments limites de l'ensemble restant $E_{1}$ (sans lui appartenir nécessairement) puisqu'ils sont éléments de condensation de $E$. Donc $A$ est aussi élément limite de $E_{1}^{\prime}$, qui est aussi fermé. Dés lors $A$ est encore élément limite de $E_{1}$, c'est bien un élément de condensation.

Montrons maintenant que tout élément de $P$ appartient à $P^{\prime}$. En effet, soit $A$ un élément de $P$, et $E_{n}$ l'ensemble des éléments $B$ de $E$ tels que $\displaystyle\cfrac{1}{n+1}<(B, A) \leqslant \cfrac{1}{n}$. Il y a une infinité de ces ensembles qui sont non dénombrables, sans quoi il y aurait un entier $q$ tel que l'ensemble des éléments $B$ de $E$ vérifiant $\displaystyle(A, B) \leqslant \cfrac{1}{q+1}$ soit dénombrable et par suite $A$ ne serait pas un élément de condensation. Ainsi, parmi les ensembles $E_{n}$, il y en a une infinité qui sont non dénombrables : $E_{n_{1}}, E_{n_{2}}, \ldots$ pris dans l'ordre des indices croissants. \textit{Comme $E$ est condensé}, l'ensemble non dénombrable $E_{n_{p}}$ donne lieu à au moins un élément de condensation $A_{n_{p}}$. $A_{n_{p}}$ est d'ailleurs distinct de $A$ puisqu'il est limite d'éléments $B$ tels que $(A, B)$ soit supérieur à $\displaystyle\cfrac{1}{n_{p}+1}$. Or on voit facilement que ($A_{n_{p}}, A$) tend vers zéro, donc $A$ appartient à $P^{\prime}$.\\

\textbf{30.} 
\textsc{\textbf{Théorème.}} --- \textit{Soit $E$ un ensemble condensé formé d'éléments d'une classe} ($V$). \textit{L'ensemble $D$ des éléments de $E$ qui ne sont pas des éléments de condensation de $E$ est un ensemble dénombrable\footnote{Même remarque que pour le théorème précédent.}.}\\

\textbf{31.} \textsc{\textbf{Corollaire.}} --- \textit{Tout ensemble fermé et condensé formé d'éléments d'une classe} ($V$) \textit{est la somme d'un ensemble dénombrable et d'un ensemble parfait ou nul sans éléments communs.}\\

\textbf{32.} \textsc{\textbf{Théorème.}} --- \textit{L'ensemble $D$ de ceux des éléments d'un ensemble compact $E$ d'éléments d'une classe} ($V$) \textit{qui n'appartiennent pas à l'ensemble $E^{\prime}$ dérivé de $E$ est dénombrable}\footnote{Pour la démonstration dans le cas où $E$ est un ensemble ponctuel, voir, par exemple, i, page 36. La seconde partie de cette dernière démonstration s'appuie sur ce que des intervalles de longueurs bornées, recouvrant le segment ($0, 1$) et dont les milieux n'appartiennent pas à deux intervalles, sont nécessairement en nombre fini. Elle ne saurait donc se généraliser ici.}.

En effet, si $A$ est un élément de $D$, appelons $\rho_{A}$ la limite inférieure $\geqslant 0$ du voisinage de $A$ avec les éléments de $E^{\prime}$. Le nombre $\rho_{A,}$ est positif, sans quoi $A$ serait un élément limite de $E^{\prime}$ et par suite appartiendrait à $E^{\prime}$.

Je dis que le nombre des éléments de $D$ pour lesquels on a $\displaystyle\rho_{A}>\cfrac{1}{n}$, est fini. En effet, dans le cas contraire, on pourrait en prendre une infinité : $A_{1}, A_{2}, \ldots, A_{p}, \ldots$ tous distincts et tendant vers une limite $B$. Alors, en prenant $p$ assez grand on aurait $\displaystyle\left(A_{p}, B\right)<\cfrac{1}{n}<\rho_{A_{p}}$, ce qui est impossible, puisque $B$, limite d'éléments de $E$, appartiendrait à $E^{\prime}$, contrairement à la définition de $\rho_{A_{p}}$.

Ainsi, il y a un nombre fini d'éléments $A$ de $D: A_{n}^{(1)}, A_{n}^{(2)}, \ldots, A_{n}^{\left(p_{n}\right)}$ tels que $\displaystyle\rho_{A} \geqslant \cfrac{1}{n}$.

Si l'on considère la suite dénombrable:
$$
A_{1}^{(1)}, \ldots, A_{1}^{\left(p_{1}\right)}, A_{2}^{(1)}, \ldots, A_{2}^{\left(p_{2}\right)}, \ldots, A_{n}^{(1)}, \ldots, A_{n}^{\left(p_{n}\right)}, \ldots,
$$
on voit que tous les éléments de $D$ y sont inscrits chacun au moins une fois. Donc $D$ est dénombrable.

En particulier, on voit que si $E$ est fermé, $E$ se décompose en son ensemble dérivé $E^{\prime}$ et un ensemble dénombrable $D$.

\textsc{\textbf{Corollaire I.}} --- \textit{Si l'ensemble dérivé $E^{\prime}$ d'un ensemble compact $E$ formé d'éléments d'une classe} ($V$) \textit{est dénombrable, l'ensemble $E$ est lui-même dénombrable.} \\

\textbf{33.} 
\textsc{\textbf{Corollaire II.}} --- \textit{Un ensemble extrémal quelconque $F$ formé d'éléments d'une classe $(V)$ peut être considéré comme l'ensemble dérivé d'un ensemble d'éléments de la classe $(V)$.} 
Du moins, cette proposition se trouvera exacte quand la classe ($V$) sera telle que l'on puisse toujours y trouver un élément dont le voisinage avec un élément arbitrairement donné soit inférieur à un nombre positif quelconque donné. Cette condition bien naturelle est satisfaite dans tous les exemples concrets que nous étudierons par la suite.

Supposons donc cette condition remplie; on aura $F=D+F^{\prime}, D$ étant un ensemble dénombrable d'éléments:
$$
A_{1}, A_{2}, \ldots, A_{n}, \ldots
$$

A chacun d'eux, $A_{n}$, correspond comme précédemment un nombre positif $\rho_{A_{n}}$. Quel que soit $p$ on pourra par hypothèse trouver un élément de la classe ($V$): $B_{n}^{(p)}$, tel que $\left(A_{n}, B_{n}^{(p)}\right)<\cfrac{1}{n p}$. Nous avons ainsi des éléments $B_{n}^{(p)}$ déterminés pour toute valeur entière de $n$ et de $p$. Appelons $E$ l'ensemble des éléments de $F^{\prime}$ et des éléments
$B_{n}^{(p)}$. Je dis que $F$ est l'ensemble dérivé de $E$. En effet, tout élément de $F$ est évidemment élément limite de $E$. Réciproquement, considérons une suite ${\Sigma}$ d'éléments de $E$ tendant vers une limite $C$. Je dis que $C$ appartient à $F$. En effet, s'il y a dans cette suite une infinité d'éléments $B_{n}^{(p)}$ correspondant à une même valeur de $n$, c'est évident. De même aussi, s'il y a une infinité d'éléments de $F^{\prime}$, car $F^{\prime}$ est fermé et contenu dans $F$. Reste le cas où il n'y aurait dans $\Sigma$ qu'un nombre fini d'éléments de $F^{\prime}$ et un nombre fini d'éléments $B_{n}^{(p)}$ pour chaque valeur de $n$. Alors il y aurait une infinité d'éléments distincts $B_{n}^{(p)}$ correspondant à des valeurs croissantes de $n$ :
$$
B_{n_{1}}^{\left(p_{1}\right)}, \ldots, B_{n_{q}}^{\left(p_{q}\right)}, \ldots
$$

En prenant $q$ assez grand, on aurait : $\left(B_{n_{q}}^{\left(p_{q}\right)}, C\right)<\varepsilon$ et $\left(A_{n_{q}}, B_{n_{q}}^{\left(p_{q}\right)}\right)<\varepsilon$ $\left[ \text{puisque } B_{n_{q}}^{\left(p_{q}\right)} \text{ tend vers } C \text{ et qu'on a:} \left(A_{n_{q}}, B_{n_{q}}^{\left(p_{q}\right)}\right)<\cfrac{1}{n_{q} p_{q}}<\cfrac{1}{n q}\right] $; 
d'où: 
$\left(A_{n_{q}}, C\right)<f(\varepsilon)$.

Comme $f(\varepsilon)$ tend vers zéro avec $\varepsilon$, on voit que $C$ serait limite d'éléments de $D$, c'est-d-dire dans $F^{\prime}$, donc encore dans $F$.\\

\textbf{34.} Appelons sphéroïde de centre $A$ et rayon $\rho$ l'ensemble de tous les éléments $B$ tels que l'on ait: $(A, B)<\rho$. Nous dirons qu'un élément $C$ est \textit{intérieur} à ce sphéroïde, si l'on a : $(A, C)<\rho$.

\textsc{\textbf{Théorème.}} --- \textit{Si un ensemble fermé $F$ appartient à un ensemble compact $E$ formé d'éléments d'une classe $(V)$, on obtiendra $F$ en supprimant de $E$ les éléments intérieurs à chacun des sphéroïdes d'un certain ensemble dénombrable de sphéroïdes}\footnote{La démonstration suivante est une généralisation de celle qui a été donnée pour le cas où $E$ est un ensemble de points du plan, par M. \textsc{Zoretti} (xxiii, page 5).}.

En effet, soit $G$ l'ensemble complémentaire de $F$, c'est-à-dire l'ensemble des éléments de $E$ ne faisant pas partie de $F$. A tout élément $A$ de $G$, nous pouvons faire correspondre un nombre $\rho_{A}$ qui sera la limite inférieure du voisinage de $A$ avec chacun des éléments de $F$. Le nombre $\rho_{A}>0$ ne pourra être nul, sans quoi $A$ appartiendrait à $F$ comme limite d'éléments de $F$.

Nous allons maintenant former une suite dénombrable d'éléments de $G$ :
$$
A_{1}^{(1)}, \ldots, A_{1}^{\left(p_{1}\right)}, A_{2}^{(1)}, \ldots, A_{2}^{\left(p_{2}\right)}, \ldots, A_{n}^{(1)}, \ldots, A_{n}^{\left(p_{n}\right)}, \ldots
$$
telle que $1^{\circ}$ on ait $\rho_{A_{n}^{(1)}} \geqslant \cfrac{1}{n}, \ldots, \rho_{A_{n}^{\left(p_{n}\right)}} \geqslant \cfrac{1}{n}$ quel que soit $n$ ; $2^{\circ}$ si $A$ est un élément de $G$ tel que : $\rho_{A} \geqslant \cfrac{1}{n}$, on ait l'une des inégalités $\left(A, A_{1}^{(1)}\right)<\cfrac{1}{n}, \ldots,\left(A, A_{n}^{\left(p_{n}\right)}\right)<\cfrac{1}{n}$. 
Pour montrer que cela est possible, supposons la suite formée jusqu'à $A_{n-\mathrm{t}}^{\left(p_{n-1}\right)}$ et appelons en général $I_{A_{n}^{(q)}}$ l'ensemble des éléments $B$ de $E$ tels que : $\left(B, A_{n}^{(q)}\right)<\cfrac{1}{n}$. Prenons alors un élément $A$ de $G$ (s'il en existe) tel que $\rho_{A} \geqslant \cfrac{1}{n}$ et qui ne fasse partie d' aucun des ensembles $I_{A_{1}^{(1)}}, \ldots, I_{A_{n-1}^{\left(p_{n-1}\right)}}$. 
Nous pourrons le prendre pour $A_{n}^{(1)}$. Puis, prenons, s'il en existe, un élément $A$ de $G$ tel que $\rho_{A} \geqslant \cfrac{1}{n}$ et qui ne fasse partie d'aucun des ensembles $I_{A_{1}^{(1)}}, \ldots, I_{A_{n-1}^{\left(p_{n-1}\right)}}, I_{A_{n}^{(1)}}$. %%%% TODO Question 
Nous l'appellerons $A_{n}^{(2)}$; et ainsi de suite. 
Nous formerons ainsi de proche en proche une suite $A_{n}^{(1)}, A_{n}^{(2)}, \ldots$ qui peut-être ne contiendra aucun terme, mais qui n'en contiendra sûrement qu'un nombre fini. En effet, d'après leur formation, ils sont tous distincts. 
Si donc il y en avait une infinité, on pourrait en extraire une suite $B_{1}, B_{2}, \ldots$ ayant une limite $B$ et alors pour $q$ assez grand on aurait $\left(B_{q}, B_{q+p}\right)<\cfrac{1}{n}$ quelque soit $p$, c'est-d-dire que $B_{q+p}$ serait intérieur à $I_{B_{q}}$, contrairement à l'hypothèse.

La suite étant ainsi formée comme nous l'avions annoncée, il est alors facile de voir que $F$ est l'ensemble des éléments de $E$ qui ne font partie d'aucun des ensembles
$$
I_{A_{1}^{(1)}}, I_{A_{1}^{(2)}}, \ldots, I_{A_{\mathrm{t}}^{\left(p_{1}\right)}}, I_{A_{2}^{(1)}}, \ldots, I_{A_{n}^{\left(p_{n}\right)}}, I_{A_{n+1}^{(1)}}, \ldots,
$$
ce qui démontre la proposition.\\

\textbf{35.} 
Appelons \textit{ensemble limité} un ensemble tiré d'une classe ($V$) tel que le voisinage de deux éléments quelconques de cet ensemble reste inférieur à un nombre fixe. Dans le cas des ensembles linéaires, nous verrons que cette définition coïncide avec celle d'ensemble compact. Dans le cas général, nous pouvons seulement énoncer la proposition suivante :

\textsc{\textbf{Théorème.}} --- \textit{Tout ensemble compact formé d'éléments d'une classe $(V)$ est limité.}

En effet, dans le cas contraire, on pourrait trouver, quel que soit $n$, deux éléments $A_{n}, B_{n}$ de $E$ tels que $\left(A_{n}, B_{n}\right)>n$, et, puisque $E$ est compact, on peut supposer que $A_{n}, B_{n}$ tendent vers deux limites respectives $A, B$. Or, pour $n$ assez grand, on aura:
$$
\left(A_{n}, A\right)<2(A, B), \quad(A, B)<2(A, B)\,,
$$
d'où:
$$
\left(A_{n}, B\right)<f[2(A, B)]=k\,.
$$
Ainsi, pour $n$ assez grand on aura:
$$
\left(A_{n}, B\right)<k \text { et }\left(B_{n}, B\right)<k\,,
$$
d'où:
$$
\left(A_{n}, B_{n}\right)<f(k)\,,
$$
ce qui conduit à une inégalité impossible $n<f(k)$.\\

\textbf{36.}
\textsc{\textbf{Théorème.}} --- \textit{Soit $E$ un ensemble extrémal formé d'éléments d'une classe $(V)$. S'il existe une suite indéfinie $G$ d'ensembles $I_{1}, I_{2}, \ldots$ telle que tout élément de $E$ soit intérieur au sens étroit à l'un au moins de ces ensembles $I_{n}$, on peut extraire de $G$ un nombre fini de ces ensembles formant une famille $H$ jouissant de la même propriété que $G$\footnote{Ce théorème est une généralisation d'un théorème de M. \textsc{Borel}, énoncé pour les ensembles linéaires (\textsc{i}, page 42), puis étendu par lui aux ensembles de points de l'espace à $n$ dimensions (\textsc{xiv}, page 357). Mais ses démonstrations ne se généralisent pas au cas actuel. Nous démontrerons plus loin ce théorème pour certaines classes ($V$) même dans le cas où $G$ n'est pas dénombrable ($\mathrm{n}^{\circ}$ 42).}.}

En effet, supposons que le théorème soit inexact. Alors il existera au moins un élément de $E$ : $A_{\mathrm{t}}$ qui n'est pas intérieur à $I_{\mathrm{t}}$ au sens étroit. 
Mais $A_{1}$ est intérieur au
sens étroit à un des ensembles $I_{2}, I_{3}, \ldots$; soit $I_{q_{1}}$ le premier d'entre eux ($q_{1}>1$). 
Il y a au moins un élément de $E$, soit $A_{2}$, qui n'est intérieur au sens étroit à aucun des ensembles $I_{1}, I_{2}, \ldots, I_{q_{1}}$. 
Appelons $I_{q_{2}}$ le premier des ensembles $I_{q_{1}+1}, I_{q_{1}+2}, \ldots$ auquel $A_{2}$ est intérieur au sens étroit et ainsi de suite.
Nous formons de la sorte une suite infinie d'éléments $A_{1}, A_{2}, \ldots$ appartenant à $E$, tous distincts et tels que $A_{r+1}$ ne soit intérieur au sens étroit à aucun des ensembles $I_{1}, I_{2}, \ldots, I_{q_{1}}, \ldots, I_{q_{r}}$. 
Cette suite a au moins un élément limite $A$ appartenant à $E$. Soit $\displaystyle A \equiv \lim _{p=\infty} A_{n_{p}}$. 
Or $A$ est intérieur au sens étroit à l'un au moins, $I_{k}$, des ensembles de la suite $G$. 
Il est donc impossible qu'il y ait dans la suite $A_{n_{1}}, A_{n_{2}}, \ldots$ une infinité d'éléments $A_{n_{1}}^{\prime}, A_{n_{2}}^{\prime}, \ldots$ qui ne soient pas intérieurs à $I_{k}$ au sens étroit. Sans quoi, on appellerait $B_{p}$ un élément de $E$ coïncidant avec $A_{n_{p}}^{\prime}$ si celui-ci n'appartient pas à $I_{k}$ ou un élément de $E$ n'appartenant pas à $I_{k}$ et tel que $\left(B_{p}, A_{n_{p}}^{\prime}\right)<\cfrac{1}{p}$ dans l'autre cas. Alors $A$ serait limite d'une suite $B_{1}, B_{2}, \ldots$ d'éléments de $E$ non dans $I_{k}$, ce qui est impossible. 
Ainsi les éléments de la suite $A_{n_{1}}, A_{n_{2}}, \ldots$ sont tous intérieurs à $I_{k}$ au sens étroit à partir d'un certain rang. Cela est manifestement contradictoire avec la façon dont nous avons formé la suite $A_{1}, A_{2}, \ldots$

\subsection*{Les classes ($V$) normales.}

\textbf{37.}
Après avoir étudié les propriétés des ensembles et des opérations portant sur des classes $(L)$, il nous a été utile de nous borner au cas des classes ($V$) pour poursuivre nos généralisations. De même, nous allons maintenant restreindre une fois de plus le champ de nos recherches sans en arriver encore à spécifier la nature des éléments considérés.

Donnons d'abord quelques définitions. Nous dirons qu'une suite d'éléments $A_{1}$, $A_{2}, \ldots$ d'une classe ($V$) satisfait aux conditions de \textsc{Cauchy} lorsqu'à tout nombre $\varepsilon>0$ on peut faire correspondre un entier $n$ tel que l'inégalité $\left(A_{n}, A_{n+p}\right)<\varepsilon$ soit vérifiée quel que soit $p$. Il est évident que si une suite tend vers une limite, elle satisfait aux conditions de \textsc{Cauchy}. D'autre part, si une suite satisfait aux conditions de \textsc{Cauchy} \textit{et fait partie d'un ensemble compact}, elle a un élément limite évidemment unique. Mais si l'on sait seulement que la suite vérifie les conditions de \textsc{Cauchy}, on ne peut affirmer qu'elle tende vers une limite; tout ce qu'on peut dire, c'est que si elle a un élément limite, elle n'en a qu'un.

Nous dirons alors \textit{qu'une classe $(V)$ admet une généralisation du théorème de \textsc{Cauchy} si toute suite d'éléments de cette classe, qui satisfait aux conditions de \textsc{Cauchy}, a un élément limite (nécessairement unique).}

Nous appellerons ensuite classe séparable une classe qui puisse être considérée d'au moins une façon comme l'ensemble dérivé d'un ensemble dénombrable de ses propres éléments.

Enfin, on a intérêt à considérer comme nous l'avons déjà fait ($\mathrm{n}^{\circ}$ 33) parmi les classes ($V$) celles qui sont telles que, près d'un élément donné, il existe des éléments
dont le voisinage avec celui-ci soit aussi petit que l'on veut sans être nul. Autrement dit, tout élément de la classe sera élément limite. Comme d'autre part la réciproque est vraie par définition même de la classe, nous dirons que de telles classes sont parfaites\footnote{Une classe séparable est nécessairement parfaite, mais la réciproque n'est pas évidemment vraie. Il y a donc lieu de séparer les deux hypothèses d'autant plus que certains théorèmes s'appliquent aux classes parfaites sans les supposer séparables.
}.

Ceci étant, nous nous bornerons maintenant à l'étude des classes ($V$) \textsc{normales}, \textit{c'est-à-dire parfaites, séparables et admettant une généralisation du théorème de \textsc{Cauchy}}. Cette limitation n'a du reste rien d'artificiel, elle provient directement de la comparaison des classes ($V$) avec les ensembles linéaires et nous verrons plus loin que toutes les classes particulières que nous examinerons rentrent dans cette catégorie générale des classes ($V$) normales. Ce dernier fait pourrait même amener à se demander si toute classe ($V$) n'est pas nécessairement normale. Il n'en est rien comme le montrent les exemples suivants:\\

{\small
\textbf{38.} 
Prenons une classe d'éléments représentés par les points d'une droite et appelons voisinage de deux d'entre eux la longueur de l'arc de cercle que limitent les deux points correspondants dans une transformation par inversion. Nous avons ainsi une classe parfaite ($V$). Cependant, si l'on prend une suite d'éléments correspondants à des points s'éloignant à l'infini, il est évident que l'on aura une suite de \textsc{Cauchy} sans éléments limites. On peut donner un exemple dans lequel le voisinage ne soit pas défini d'une façon aussi artificielle. 
Il suffit de prendre la classe des nombres en se plaçant au point de vue des arithméticiens qui se défendent la considération des nombres irrationnels. 
En prenant pour voisinage de deux nombres rationnels, la valeur absolue de leur différence, on obtient encore une classe parfaite ($V$) pour laquelle il existe une infinité de suites vérifiant les conditions de \textsc{Cauchy} sans avoir d'éléments limites.

Passons maintenant aux classes séparables. On peut qualifier ainsi les ensembles linéaires en considérant la droite indéfinie comme l'ensemble dérivé de l'ensemble des points d'abscisses rationnelles. 
Mais il n'en est pas de même pour toute classe parfaite ($V$).

Prenons par exemple la classe des fonctions (continues ou discontinues) d'une variable $x$ dans l'intervalle $(0, 1)$. En appelant voisinage de deux éléments $f(x), g(x)$, la limite supérieure (finie ou non) de $|f(x)-g(x)|$ dans l'intervalle $(0, 1)$, on voit qu'on obtient une classe ($V$) parfaite. Cette classe n'est pas séparable. En effet, si elle l'était, on pourrait former une fois pour toutes une suite de fonctions $f_{1}(x), f_{2}(x), \ldots$ telle que tout élément de la classe soit la limite uniforme d'une suite $f_{n_{1}}(x), f_{n_{2}}(x), \ldots$ extraite de la précédente. Alors les éléments de la classe étant définis par des conditions dénombrables, la puissance de la classe serait au plus égale à celle du continu (\textsc{i}, page 126). 
Or on sait que c'est le contraire qui a lieu (\textsc{i}, page 125). 
On peut remarquer que les exemples précédents nous prouvent que la puissance d'un ensemble \textit{parfait} tiré d'une classe ($V$) n'est pas nécessairement la puissance du continu comme cela a lieu pour les ensembles linéaires, mais qu'elle peut lui être inférieure (premier exemple) ou supérieure (deuxième exemple).
}\\

\textbf{39.} 
Ces remarques faites, limitons-nous maintenant à l'étude des classe ($V$) normales.

Tout d'abord, pour arriver à nous rendre compte de la structure de telles classes, nous généraliserons une question proposée par M. \textsc{Hadamard} (\textsc{xii}). La question proprement dite sera étudiée plus loin (voir n$^{\circ}$ 58). Nous l'étendrons au cas général actuel de la façon suivante:

Considérons une classe ($V$). Supposons qu'on ait pu former des ensembles partiels $k_{\varepsilon}$ contenant chacun au moins un élément et tels: $1^{\circ}$ que tout élément de la classe appartienne à l'un des ensembles $k_{\varepsilon}, 2^{\mathrm{o}}$ que deux éléments quelconques d'un même ensemble $k_{\varepsilon}$ aient un voisinage inférieur à $\varepsilon$. Considérant les $k_{\varepsilon}$ comme autant d'individus, on peut dire avec M. \textsc{Hadamard} que l'ensemble $\mathfrak{K}_{\varepsilon}$, qui a ces $k_{\varepsilon}$ comme éléments, «numère» la classe considérée. Nous nous proposons de rechercher la puissance de $\mathfrak{K}_{\varepsilon}$.

Nous allons trouver ici une nouvelle analogie avec les ensembles linéaires. Si l'on prend la classe des points d'une droite, le problème consiste à trouver la puissance de l'ensemble des intervalles de longueurs $<\varepsilon$ et qui recouvrent la droite indéfinie. Or il est évident qu'on peut les choisir de façon que cet ensemble soit dénombrable quoique infini.\\

\textbf{40.} 
\textit{De même, étant donnée une classe $(V)$ séparable, on peut, quel que soit $\varepsilon$, choisir les ensembles $k_{\varepsilon}$ de façon que $\mathfrak{K}_{\varepsilon}$ soit dénombrable.}

En effet, soient $\omega$ et $\eta$ deux nombres tels que $f(\omega)<\varepsilon$ et $f(\eta)<\omega$. %%% TODO Question 
Puisque la classe est séparable, on peut en extraire une suite d'éléments $A_{1}, A_{2}, \ldots$ dont l'ensemble dérivé soit la classe toute entière. Appelons alors $K_{\varepsilon}^{(p)}$ l'ensemble des éléments $A$ tels que : $\left(A, A_{p}\right)<\omega$. La suite $K_{\varepsilon}^{(1)}, K_{\varepsilon}^{(2)}, \ldots$ sera dénombrable; de plus, pour deux éléments quelconques $A, B$ de $K_{\varepsilon}^{(p)}$, on aura: $(A, B)<\varepsilon$; enfin tout élément $A$ de la classe appartiendra pour une valeur donnée de $\varepsilon$ à l'un au moins des $K_{\varepsilon}^{(p)}$. L'ensemble des $K_{\varepsilon}^{(p)}$ constitue donc l'ensemble $\mathfrak{K}_{\varepsilon}$ cherché. On peut même ajouter que tout élément $A$ est intérieur au sens étroit à l'un au moins des ensembles $K_{\varepsilon}^{(1)}, K_{\varepsilon}^{(2)}, \ldots$. Il suffit de prendre dans $A_{1}, A_{2}, \ldots$ un élément $A_{n_{1}}$ tel que $\left(A, A_{n_{1}}\right)<\eta$; alors $A$ est intérieur au sens étroit à $K_{\varepsilon}^{\left(n_{1}\right)}$.\\

\textbf{41.} 
La même méthode prouve qu'étant donné un \textit{ensemble} $E$ appartenant à une classe séparable ($V$), on peut former une infinité dénombrable $\mathfrak{K}_{\varepsilon}$ d'ensembles $K_{\varepsilon}$ d'éléments de $E$ tels que tout élément de $E$ soit intérieur au sens étroit à l'un au moins des $K_{\varepsilon}$ et que le voisinage de deux éléments quelconques de $K_{\varepsilon}$ reste inférieur à $\varepsilon$. On peut se demander s'il existe des ensembles $E$ tels que l'ensemble $\mathfrak{K}_{\varepsilon}$ soit non seulement dénombrable, mais fini.

\textsc{\textbf{Théorème.}} --- \textit{Pour que l'ensemble $\mathfrak{K}_{\varepsilon}$ $[$correspondant à un ensemble $E$ tiré d'une classe $(V)$ \textsc{normale}$]$ puisse être choisi, quel que soit $\varepsilon$, de façon à ne comprendre qu'un nombre fini d'éléments, il faut et il suffit que $E$ soit compact.}

La condition est nécessaire. En effet, dans le cas contraire, on pourrait extraire de $E$ une suite infinie $S$ d'éléments distincts $B_{1}, B_{2}, \ldots$ sans éléments limites. Si $\mathfrak{K}_{\varepsilon}$ est fini, il y aura nécessairement un ensemble partiel $K_{\varepsilon}$ auquel appartiennent une infinité d'éléments de la suite $S$. On voit alors qu'on pourra former de proche en proche une infinité de suites $S_{n}$ d'éléments de $S$, telle que $S_{n+1}$ soit contenu dans $S_{n}$ et que l'écart de deux éléments de $S_{n}$ soit inférieur à $\cfrac{1}{n}$. Si donc j'appelle $B_{1}^{(p)}, B_{2}^{(p)}, \ldots$ les éléments de la suite $S_{n}$ pris dans le même ordre que dans $S$, on voit que la suite $B_{1}^{(1)}$, $B_{2}^{(2)}, \ldots, B_{p}^{(p)}, \ldots$ sera une suite d'éléments de $S$ distincts et tels que l'on ait $\left(B_{p}^{(p)}, B_{n+p}^{(n+p)}\right)<\cfrac{1}{p}$ quel que soit $n$. Puisque $E$ est tiré d'une classe $(V)$ normale, il faudrait donc que la suite $S$ eut un élément limite.

Réciproquement, supposons $E$ compact. Alors l'ensemble $F \equiv E+E^{\prime}$ est extrémal. Pour une valeur donnée de $\varepsilon$, nous savons qu'on peut former une suite d'ensembles partiels $K_{\varepsilon}^{(1)}, K_{\varepsilon}^{(2)}, \ldots$ telle que leur ensemble réponde aux conditions d'un $\mathfrak{K}_{\varepsilon}$ relativement à $F$. En particulier, tout élément de $F$ est intérieur au sens étroit à l'un des ensembles $K_{\varepsilon}^{(1)}, K_{\varepsilon}^{(2)}, \ldots$. Donc, on peut extraire de cette suite $K_{\varepsilon}^{(1)}, K_{\varepsilon}^{(2)}, \ldots$ un nombre fini de termes $K_{\varepsilon}^{\left(q_{1}\right)}, \ldots, K_{\varepsilon}^{\left(q_{r}\right)}$ jouissant de la même propriété (voir $\mathrm{n}^{\circ}$ 36). 
Si nous appelons maintenant $H_{\varepsilon}^{\left(q_{k}\right)}$ l'ensemble des éléments de $E$ qui appartiennent à $K_{\varepsilon}^{\left(q_{k}\right)}$ (lequel est dans $F$), on voit qu'on aura un nombre fini d'ensembles $H_{\varepsilon}^{\left(q_{1}\right)}, \ldots, H_{\varepsilon}^{\left(q_{r}\right)}$ formés avec des éléments de $E$ et tels: 1$^{\circ}$ que tout élément de $E$ soit intérieur au sens étroit à au moins l'un d'eux, 2$^{\circ}$ que deux éléments quelconques de l'un d'eux aient un voisinage $<\varepsilon$.

Il nous est maintenant facile de généraliser le théorème du $\mathrm{n}^{\circ}$ 36.\\

\textbf{42.} 
\textsc{\textbf{Théorème.}} --- \textit{Soit $E$ un ensemble d'éléments d'une classe normale $(V)$. Pour que de toute famille $H$ \textsc{dénombrable ou non}\footnote{Dans le cas où $E$ est un ensemble linéaire, on obtient la généralisation du théorème de M. \textsc{Borel} (voir la note du n$^{\circ}$ 36) étendu par M. \textsc{Lebesgue} au cas où la famille $H$ est non dénombrable. Sa démonstration (\textsc{iv}, page 105) ne se généralise pas au cas actuel.} d'ensembles I tels que tout élément de $E$ soit intérieur au sens étroit à au moins l'un d'eux, on puisse extraire un nombre fini d'ensembles I formant une famille $G$ jouissant de la même propriété que $H$, il faut et il suffit que $E$ soit extrémal.}

Nous avons démontré ($\mathrm{n}^{\circ}$ 36) que la condition est suffisante dans le cas où $H$ est dénombrable.

Pour le cas général, remarquons que, si $E$ est extrémal, on peut former, quel que soit $\varepsilon$, des ensembles $K_{\varepsilon}$ en nombre fini satisfaisant aux conditions indiquées plus haut. Si le théorème n'est pas vrai pour $E$, il y a au moins un de ces ensembles tels que ses éléments ne soient pas intérieurs au sens étroit à un nombre fini d'ensembles $I$. Pour $\varepsilon=\cfrac{1}{n}$ appelons celui-là $K^{(n)}$ et soit $A_{n}$ l'un de ses éléments. Puisque $E$ est extrémal, on peut extraire de la suite $A_{1}, A_{2}, \ldots$ une suite $A_{n_{1}}, A_{n_{2}}, \ldots$ qui tend vers un élément $A$ de $E$. $A$ est intérieur au sens étroit à un intervalle $I: I_{0}$ et on prouve facilement que pour $p$ assez grand tout élément de $K^{(n_p)}$ est aussi intérieur au sens étroit à $I_{0}$, ce qui amène bien à une contradiction.

La condition est aussi nécessaire. En effet, supposons que $E$ ne soit pas fermé, il existera une suite d'éléments $B_{1}, B_{2}, \ldots$ de $E$, qui tendent vers un élément $B$ n'appartenant pas à $E$. Or, considérons les ensembles $I_{n}$ formés chacun des éléments $A$ de $E$ tels que $(A, B)>\cfrac{1}{n}$. Tout élément de $E$ est intérieur au sens étroit à l'un au moins des $I_{n}$. Mais si l'on considère un nombre fini de ces ensembles $I_{n}$, il y aura certainement des termes de la suite $B_{1}, B_{2}, \ldots$ qui ne leur appartiennent pas.

De même, supposons que $E$ ne soit pas compact; il existera une suite $S$ d'éléments de $E: B_{1}, B_{2}, \ldots$ sans éléments limites. Si nous considérons un élément $A$ quelconque de $E$, nous pourrons définir un nombre $\rho_{A}>0$ tel que $\left(A, B_{n}\right) \geqslant \rho_{A}$, quel que soit l'élément $B_{n}$ distinct de $A$ et pris dans la suite $S$; alors $A$ sera intérieur au sens étroit à l'ensemble $I_{A}$ des éléments $C$ de $E$ tels que $(C, A)<\rho_{A}$. Il en résulte que tout élément $B$ de $E$ est intérieur au sens étroit à l'un au moins des intervalles $I_{A}$, à savoir $I_{B}$. Si de la famille $H$ des intervalles $I_{A}$, on en extrait un nombre fini formant une famille $G$, il sera impossible que $G$ contienne $E$, car il y a dans tout intervalle $I_{A}$ un élément au plus de la suite $S$.\\

\textbf{43.} 
\textsc{\textbf{Théorème.}} --- \textit{Tout ensemble non dénombrable $E$ formé d'éléments d'une classe $(V)$ normale est condensé.}

Soit $E_{1}$ une infinité non dénombrable d'éléments de $E$, il s'agit de démontrer que $E_{1}$ donne lieu à au moins un élément de condensation. En effet, quel que soit $\varepsilon$ on peut, comme nous l'avons vu, trouver une suite dénombrable d'ensembles $K_{\varepsilon}^{(1)}, K_{\varepsilon}^{(2)}, \ldots, K_{\varepsilon}^{(n)}, \ldots$, telle que tout élément de $E_{1}$ se trouve dans l'un d'eux et que le voisinage de deux éléments de l'un d'eux soit $<\varepsilon$. Il y a donc au moins un de ces ensembles qui contient une infinité non dénombrable d'éléments de $E_{1}$. 
En prenant successivement $\varepsilon=1$, $\cfrac{1}{2}, \ldots \cfrac{1}{n}, \ldots$, nous pourrons ainsi former une suite d'ensembles $H^{(1)}, H^{(2)}, \ldots$ telle que $H^{(n)}$ contienne une infinité non dénombrable d'éléments de $E_{1}$, soit contenu dans $H^{(n-1)}$, et que deux quelconques des éléments de $H^{(n)}$ aient un voisinage inférieur à $\cfrac{1}{n}$. 
Alors, si on prend deux éléments quelconques $A_{n}, A_{n}^{\prime}$ dans $H^{(n)}$, chacune des suites $A_{1}, A_{2}, \ldots ; A_{1}^{\prime}, A_{2}^{\prime}, \ldots$ a une limite $A$ qui est la même. 
Donc $E_{1}$ donne lieu à un élément limite $A$ et c'est un élément de condensation, car, si on enlève de $E_{1}$ une infinité dénombrable d'éléments, il restera encore des éléments dans chacun des $H^{(n)}$ et $A$ sera encore élément limite de l'ensemble restant de $E_{1}$.\\

\textbf{44.} 
\textsc{\textbf{Remarque.}} --- En combinant le théorème précédent avec celui du n$^{\circ}$ 31 on obtient l'énoncé suivant:

\textit{
Tout ensemble fermé $F$ formé d'éléments d'une classe $(V)$ normale est la somme d'un ensemble dénombrable et d'un ensemble parfait ou nul sans éléments communs.}\\

\textbf{45.} 
\textsc{\textbf{Théorème.}} --- \textit{Soit $E$ un ensemble quelconque formé d'éléments d'une classe séparable $(V)$; il existe un ensemble dénombrable d'éléments de $E$ tel que tout élément de $E$ appartienne, soit à cet ensemble $D$, soit à son dérivé $D^{\prime}$. Lorsque $E$ est fermé, on a: $E \equiv D+D^{\prime}$. Lorsque $E$ est parfait, $E \equiv D^{\prime}$.}

En effet, quel que soit $n$, on peut former une infinité dénombrable d'ensembles $H_{n}^{(1)}, H_{n}^{(2)}, \ldots, H_{n}^{(p)}, \ldots$ formés d'éléments de $E$ tels que dans chacun d'eux le voisinage reste inférieur à $\cfrac{1}{n}$ et que tout élément de $E$ soit dans l'un des ensembles de cette suite. Dans chacun de ces ensembles $H_{n}^{(p)}$ il y a au moins un élément $A_{n}^{(p)}$. Quand on donne à $n$ et $p$. des valeurs entières quelconques, on obtient un ensemble dénombrable $D$ d'éléments $A_{n}^{(p)}$ appartenant à $E$. Or il est manifeste que tout élément de $E$ appartient à $D$ ou à $D^{\prime}$.

L'inverse n'est pas en général exact; mais si $E$ est fermé tout élément de $D+D^{\prime}$ appartiendra à $E$; donc dans ce cas $E \equiv D+D^{\prime}$. De plus $E^{\prime} \equiv D^{\prime}+D^{\prime \prime} \equiv D^{\prime}$. Si même $E$ est parfait, on aura $E \equiv E^{\prime}$ d'où $E \equiv D^{\prime}$.

Observons d'ailleurs que, réciproquement, si $E, D$ sont deux ensembles formés d'éléments d'une classe $(V)$, tels que l'on ait: $E \equiv D+D^{\prime}$, l'ensemble $E$ est nécessairement fermé. Si $E \equiv D^{\prime}$ ($D$ étant une partie de $E$), $E$ est parfait.

\subsection*{La continuité définie au moyen du voisinage.}

\textbf{46.}
\textsc{\textbf{Théorème.}} --- \textit{Considérons une opération $U$ définie dans un ensemble $E$ formé d'éléments d'une classe $(V)$. La condition nécessaire et suffisante pour que $U$ soit une opération continue dans $E$ est que, si $A$ est un élément quelconque commun à $E$ et à $E^{\prime}$, on puisse faire correspondre à tout nombre $\varepsilon>0$ un nombre $\eta_{A}$ tel que l'inégalité $(A, B)<\eta_{A}$ entraîne $|U(A)-U(B)|<\varepsilon$ pour tout élément $B$ de $E$.}

1$^{\circ}$ En effet, d'après la définition que nous avons donnée de la continuité de $U$, si $U$ est continue en $A$ et si $A_{1}, A_{2}, \ldots, A_{n}, \ldots$ tendent vers $A,\, U\left(A_{n}\right)$ tend vers $U(A)$. Soit maintenant $\varepsilon$ un nombre positif quelconque; si on ne pouvait déterminer un nombre $n_{A}$ tel que l'inégalité $(A,\, B)<\eta_{A}$ entraîne $|U(A)-U(B)|<\varepsilon$, on pourrait déterminer, quel que soit $n$, un élément $B_{n}$ de $E$ tel que:
$$
\left(A, B_{n}\right)<\cfrac{1}{n}, \quad\left|U(A)-U\left(B_{n}\right)\right| \geqslant \varepsilon .
$$

Lorsque $n$ croît indéfiniment, la première inégalité montre que $B_{n}$ tend vers $B$ et, d'après l'hypothèse, $U\left(B_{n}\right)$ tendra vers $U(A)$, ce qui amène une contradiction avec la seconde inégalité.

$2^{\circ}$ Si, quel que soit $\varepsilon$, on peut déterminer $\eta_{A}$ tel que $(A, B)<\eta_{A}$ entraîne $|U(A)-U(B)|<\varepsilon$, on voit qu'on pourra prendre $p$ assez grand pour que si la suite $B_{1}, B_{2}, \ldots$ tend vers $B$, l'inégalité $n>p$ entraîne: $\left|U(A)-U\left(B_{n}\right)\right|<\varepsilon$. Il suffira de prendre $p$ assez grand pour que $n>p$ entraîne $\left(A, B_{n}\right)<\eta_{A}$.

Cela prouve que $U\left(B_{n}\right)$ tend vers $U(A)$.\\

\textbf{47.} 
Ce théorème nous fournit une seconde définition de la continuité d'une opération. Cette définition est celle qui est généralement adoptée pour les exemples concrets habituels. Elle est d'ailleurs moins générale que la première, puisqu'elle n'a de sens que lorsqu'on peut définir un voisinage.

Mais l'introduction du voisinage est absolument nécessaire si l'on veut étendre la notion de continuité uniforme.

Nous dirons qu'une opération $U$ est uniformément continue dans un ensemble $E$ formé d'éléments d'une classe $(V)$ si, étant donné un nombre positif s , on peut choisir un nombre positif $\eta$ tel que, pour deux éléments quelconques de $E: A, B$, l'inégalité:
$$
(A, B)<\eta \quad \text { entraîne } \quad|U(A)-U(B)|<\varepsilon .
$$

Il résulte évidemment de cette définition que toute opération uniformément continue dans un ensemble $E$ est continue dans $E$. La réciproque est vraie dans un cas très général.

\textsc{\textbf{Théorème.}} --- \textit{Toute opération continue dans un ensemble \textsc{extrémal} $E$ formé d'éléments d'une classe $(V)$ est uniformément continue dans $E$.}

En effet, dans le cas contraire, on pourrait trouver un nombre $\varepsilon>0$ tel que, quel que soit $n$, il y ait deux éléments $A_{n}, B_{n}$ de $E$ vérifiant:
$$
\left(A_{n}, B_{n}\right)<\cfrac{1}{n}, \quad\left|U\left(A_{n}\right)-U\left(B_{n}\right)\right| \geqslant \varepsilon .
$$

De la suite $A_{1}, A_{2}, \ldots$ on pourrait extraire une suite $A_{p_{1}}, A_{p_{2}}, \ldots$ ayant pour limite un élément $A$ de $E$. Alors $B_{p_{n}}$ aurait la même limite $A$, puisque ($A_{p_{n}}, A$) et $\left(A_{p_{n}}, B_{p_{n}}\right)$ étant infiniment petits avec $\cfrac{1}{n}$ il en est de même de $\left(A, B_{p_{n}}\right)$. Or on a:
$$
\left|U\left(A_{p_{n}}\right)-U\left(B_{p_{n}}\right)\right| \leqslant\left|U\left(A_{p_{n}}\right)-U(A)\right|+\left|U(A)-U\left(B_{p_{n}}\right)\right| .
$$

Les deux quantités du second membre tendent vers zéro avec $\cfrac{1}{n}$. Il est donc impossible que le premier membre reste $\geqslant \varepsilon$.\\

\textbf{48.}
\textbf{\textit{Les opérations également continues.}} --- Lorsque l'on considère des opérations continues dans un ensemble $E$ formé d'éléments d'une classe $(V)$, on peut énoncer les conditions qui définissent leur égale continuité ($\mathrm{n}^{\circ}$ 15) d'une façon qui fait intervenir le voisinage et qui est parfois plus commode.

Soit $\mathfrak{F}$ famille d'opérations continues dans un ensemble quelconque $E$ formé d'éléments d'une classe $(V)$. Si cette famille est telle que, à tout nombre $\varepsilon>0$, on puisse faire correspondre un nombre $\eta>0$ de façon que l'on ait:
$$
|U(A)-U(B)|<\varepsilon
$$
pour toute opération $U$ de $\mathfrak{F}$ et pour tout couple d'éléments $A, B$ de $E$ vérifiant $(A, B)<\eta$, les opérations de $\mathfrak{F}$ sont également continues dans $E$. Cela résulte immédiatement de la définition du n$^{\circ}$ 15; on voit en même temps que chacune des opérations de sera $\mathfrak{F}$ \textit{uniformément} continue.

Inversement, cette condition sera vérifiée par toute famille $\mathfrak{F}$ d'opérations également continues dans un ensemble \textit{extrémal} $E$ formé d'éléments d'une classe $(V)$. En effet, dans le cas contraire, on pourrait trouver un nombre $\varepsilon>0$, tel que, quel que soit $n$, il existe deux éléments $A_{n}, B_{n}$ de $E$ et une opération $U_{n}$ de $\mathfrak{F}$ pour lesquels:
$$
\left(A_{n}, B_{n}\right)<\cfrac{1}{n}, \quad\left|U_{n}\left(A_{n}\right)-U_{n}\left(B_{n}\right)\right| \geqslant \varepsilon .
$$

On peut même supposer que la suite $A_{1}, A_{2}, \ldots, A_{n}, \ldots$ a une limite $A$ dans $E$, puisque $E$ étant extrémal il suffirait dans le cas contraire de remplacer $A_{1}, A_{2}, \ldots$ par une suite convenablement extraite de la précédente. Alors $\left(A, A_{n}\right)$ et $\left(A_{n}, B_{n}\right)$ seront infiniment petits avec $\cfrac{1}{n}$, donc aussi $\left(A, B_{n}\right)$. Il en résulte que la suite $B_{1}, B_{2}, \ldots$ tend aussi vers $A$. Mais, puisque les opérations de $\mathfrak{F}$ sont également continues, on pourra déterminer deux nombres fixes $p, p^{\prime}$ tels que l'on ait:
$$
\begin{array}{ll}
\left|U_{q}\left(A_{n}\right)-U_{q}(A)\right|<\cfrac{\varepsilon}{2} & \text { pour } n>p \,,\\
\left|U_{q}\left(B_{n}\right)-U_{q}(A)\right|<\cfrac{\varepsilon}{2} & \text { pour } n>p^{\prime}\,,
\end{array}
$$
et ceci quel que soit l'entier $q$. Dés lors on aura, pour $n>p+p^{\prime}$,
$$
\left|U_{n}\left(A_{n}\right)-U_{n}\left(B_{n}\right)\right| \leqslant\left|U_{n}\left(A_{n}\right)-U_{n}(A)\right|+\left|U_{n}(A)-U_{n}\left(B_{n}\right)\right|<\cfrac{\varepsilon}{2}+\cfrac{\varepsilon}{2}=\varepsilon,
$$
d'où la contradiction annoncée.

Les conditions que je viens d'indiquer sont celles qui servent à M. \textsc{Arzelà} pour définir l'égale continuité dans les cas qu'il a considérés. On voit que nos résultats sont un peu plus étendus, même en considérant les mêmes éléments que lui, puisque notre définition du $n^{\circ}$ if comprend des cas où il n'y a pas continuité égale au sens de M. \textsc{Arzelà} et qui se présentent lorsque $E$ n'est pas extrémal (voir un exemple au n$^{\circ}$ 54).

Dans le cas où $E$ est formé des éléments d'une classe séparable, la condition imposée à $E$ dans le théorème général ($\mathrm{n}^{\circ}$ 19), que l'on ait $E \equiv D+D^{\prime}, D$ étant dénombrable, se trouve remplie d'elle-même. Ce théorème devient donc le suivant:

\textsc{\textbf{Théorème.}} --- \textit{Pour que des opérations continues dans un même ensemble extrémal E, formé d'éléments d'une classe $(V)$ séparable, forment une famille compacte $\mathfrak{F}$, il faut et il suffit que les opérations de $\mathfrak{F}$ soient, en tout élément de $E$, également continues et bornées.
}\\

\textbf{49.} 
\textbf{\textit{Introduction de l'écart.}} --- Lorsque nous appliquerons les résultats généraux de la \textsc{Première Partie} à des exemples concrets, nous reconnaîtrons d'abord que, dans chaque cas, on peut faire correspondre à tout couple d'éléments $A, B$ un nombre $(A, B) \geqslant 0$, que nous appellerons \textit{l'écart des deux éléments} et qui jouit des deux propriétés suivantes: \textit{a)} L'écart ($A, B$) n'est nul que si $A$ et $B$ sont identiques. \textit{b)} Si $A, B, C$, sont trois éléments quelconques, on a toujours $(A, B) \leqslant(A, C)+(C, B)$.

Lorsqu'on peut définir l'écart de deux éléments quelconques d'une certaine classe, nous dirons que celle-ci est une classe ($E$).

Il est facile de voir que le nombre ainsi défini satisfait aux conditions imposées à la définition du voisinage. En effet, la condition 1$^{\circ}$ du n$^{\circ}$ 27, sera remplie d'elle-même et la condition 2$^{\circ}$ sera remplie, en prenant par exemple $f(\varepsilon)=2 \varepsilon$, si l'on tient compte de la condition \textit{b)} actuelle.

Ainsi, \textit{l'écart est un voisinage} qui jouit d'une propriété particulière, ou, si l'on veut, toute classe ($E$) est une classe $(V)$. Dans la plupart des démonstrations des théorèmes connus, la propriété  \textit{b)} de l'écart intervient dans les raisonnements. Cependant la théorie développée dans ce Chapitre montre qu'elle n'est pas indispensable et qu'il suffit de se servir du voisinage sans avoir besoin pour cela de compliquer notablement le raisonnement.\\

\textbf{50.} 
Une exception doit être faite cependant pour le théorème que nous allons établir maintenant; l'hypothèse qu'on opère sur une classe $(E)$ intervient en effet d'une manière essentielle dans la démonstration. Malgré cela, il est pourtant vraisemblable que l'énoncé reste exact pour toutes les classes $(V)$.

Ce théorème est la réciproque du théorème que nous avons donné au début (n$^{\circ}$ 11) concernant le maximum d'une opération continue. J'attire l'attention sur le mode de démonstration et aussi sur la réciproque elle-même qui me paraît donner dans certains cas une forme précise à un principe général énoncé d'une façon un peu vague par M. \textsc{Hilbert} (\textsc{xx}, page 137):

« Tout problème du Calcul des variations possède une solution, pourvu que certaines hypothèses restrictives convenablement choisies relatives à la nature des conditions aux limites données soient remplies, et nécessairement aussi pourvu que ce que l'on entend par le mot \textit{solution} éprouve une généralisation conforme au sens, à la nature des choses ».\\

\textbf{51.} 
\textsc{\textbf{Théorème.}} --- \textit{La condition nécessaire et suffisante pour que toute opération continue dans un ensemble $E$ d'éléments d'une classe $(E)$, $1^{\circ}$ soit bornée dans cet ensemble, $2^{\circ}$ y atteigne sa limite supérieure, est que cet ensemble $E$ soit extrémal.}

Nous avons déjà prouvé que la condition est suffisante.

Nous montrerons maintenant que si l'ensemble $E$ n'était pas extrémal, on pourrait former au moins deux opérations continues dans $E$ : l'une non bornée, l'autre bornée mais n'atteignant pas sa limite supérieure. Observons qu'il suffit d'obtenir la première $U$, car alors on pourra prendre pour la seconde: $V \equiv \cfrac{U^{2}}{1+U^{2}}$ qui n'atteindra jamais sa limite supérieure: i.

1$^{\circ}$ Supposons d'abord que $E$ ne soit pas fermé. Il y a donc un élément $A$, limite d'éléments de $E$ et n'appartenant pas à $E$. Alors il suffira de prendre pour valeur de $U(B)$ en chaque élément $B$ de $E$ :
$$
U(B)=\cfrac{1}{(A, B)}\,.
$$

Cette opération est évidemment non bornée. Elle est bien définie en tout élément $B$ de $E$; de plus elle est continue, car si $B$ et $C$ sont deux éléments de $E$, on a:
$$
|U(B)-U(C)|=\left|\cfrac{(A, B)-(A, C)}{(A, B)(A, C)}\right| .
$$

Or, en prenant $B$ fixe et $\varepsilon$ aussi petit que l'on veut et en particulier plus petit que $(A, B)$, comme on a:
$$
|(A, C)-(A, B)|<(B, C),
$$
l'inégalité: $(B, C)<\varepsilon$ entraînera:
$$
|(A, B)-(A, C)|<\varepsilon, \quad(A, B) \cdot(A, C)>(A, B)[(A, B)-\varepsilon] .
$$

Donc, si $\omega$ est un nombre $>0$ aussi petit que l'on veut, il suffira de choisir $\varepsilon$ de façon que:
$$
\varepsilon<(A, B) \quad \text { et } \quad \cfrac{\varepsilon}{(A, B)[(A, B)-\varepsilon]}<\omega\,,
$$
pour que l'inégalité:
$$
(B, C)<\varepsilon\, \text { entraîne }\, |U(B)-U(C)|<\omega .
$$

$2^{\circ}$ Considérons de même le cas où $E$ serait non compact. Alors on pourrait trouver dans $E$ une suite infinie $S$ d'éléments de $E$ distincts
$$
A_{1}, A_{2}, \ldots, A_{n}, \ldots
$$
tels que la suite $S$ n'ait aucun élément limite. Pour former une opération $U$ continue et non bornée dans cet ensemble $E$, nous ferons d'abord quelques remarques sur la suite $S$.

Soit $\varepsilon_{p}$ la limite inférieure des écarts de $A_{p}$ avec tous les autres éléments de la suite $S$. Le nombre $\varepsilon_{p} \geqslant 0$ ne peut être nul, sans quoi on pourrait extraire de $S$ une suite tendant vers $A_{\mathrm{p}}$.

Nous décomposerons alors $E$ en ensembles partiels de la manière suivante. Appelons $E_{p}$ l'ensemble des éléments $B$ de $E$ tels que: $\left(B, A_{p}\right) \leqslant \alpha_{p}$, en nommant $\alpha_{p}$ le plus petit des deux nombres $\cfrac{1}{p}$ et $\cfrac{\varepsilon_{p}}{3}$. Soient alors $B$ un élément de $E_{p}$, et $C$ un élément de $E_{q}$; on aura:
\begin{equation*}
\left(A_{p}, A_{q}\right) \leqslant\left(A_{p}, B\right)+\left(C, A_{q}\right)+(B, C) . \tag{I}
\end{equation*}

Or, quels que soient $p$ et $q$ on aura, d'après la définition même de $\varepsilon_{p}$ et $\varepsilon_{q}$:
$$
\left(A_{p}, A_{q}\right) \geqslant \varepsilon_{p} \quad \text { et } \quad\left(A_{p}, A_{q}\right) \geqslant \varepsilon_{q},
$$
d'où:
$$
\left(A_{p}, A_{q}\right) \geqslant \cfrac{\varepsilon_{p}+\varepsilon_{q}}{2} .
$$
D'autre part, d'après la définition de $E_{p}$ et $E_{q}$ :
$$
\left(A_{p}, B\right) \leqslant \cfrac{\varepsilon_{p}}{3}, \quad\left(A_{q}, C\right) \leqslant \cfrac{\varepsilon_{q}}{3} ;
$$
l'inégalité devient donc:
$$
\cfrac{\varepsilon_{p}+\varepsilon_{q}}{2} \leq(B, C)+\cfrac{\varepsilon_{p}+\varepsilon_{q}}{3} \text {. }
$$
D'où:
$$
(B, C) \geqslant \cfrac{\varepsilon_{p}+\varepsilon_{q}}{6}
$$

Ainsi, l'écart de deux éléments quelconques, l'un dans $E_{p}$, l'autre dans $E_{q}$, reste supérieur à un nombre positif fixe. Cela prouve que: $1^{\circ}$ $E_{p}$ et $E_{q}$ n'ont aucun élément commun; $2^{\circ}$ aucun élément limite de $E_{p}$ n'appartient à $E_{q}$, ni inversement. Enfin, si l'on considère une suite d'éléments $B_{1},\, B_{2}, \ldots$ appartenant respectivement à des ensembles $E_{p_{1}},\, E_{p_{2}}, \ldots$ tous distincts, il est impossible qu'une telle suite ait une limite. En effet, dans ce cas on pourrait d'abord, en ne considérant au besoin qu'une suite extraite de la suite donnée, supposer que les indices $p_{1},\, p_{2}, \ldots$ vont en croissant. Or, on aurait, en appelant $C$ la limite de cette suite d'éléments,
$$
\left(C, A_{p_{n}}\right) \leqslant\left(C, B_{n}\right)+\left(B_{n}, A_{p_{n}}\right)\,,
$$
et puisque par hypothèse $\left(B_{n}, A_{p_{n}}\right) \leqslant \cfrac{1}{p_{n}}$, on voit que les deux termes du second membre tendraient vers zéro avec $\cfrac{1}{n}$. Or ceci est impossible puisqu'alors il y aurait une suite $A_{p_{1}},\, A_{p_{2}}, \ldots$ extraite de $S$ et tendant vers une limite $C$.

Ceci étant, nous formerons l'opération cherchée $U$ de la manière suivante. Nous prendrons:
$$
U(B)=\left[\alpha_{p}-\left(B, A_{p}\right)\right] \cfrac{p}{\alpha_{p}}\,,
$$
lorsque $B$ est un élément quelconque de $E_{p}$, et nous prendrons $U(B)=0$ quand $B$ n'est dans aucun des ensembles $E_{1}, E_{2}, \ldots$ c'est-à-dire est dans l'ensemble $G \equiv E-E_{1}-E_{2}-\cdots$. On voit d'abord que $U$ sera une opération bien déterminée en tout élément de $E$. Elle n'est pas bornée, car on a:
$$
U\left(A_{p}\right)=p .
$$

Elle est pourtant continue dans $E$. Il suffit de montrer que si des éléments de $E$ distincts : $C_{1}, C_{2}, \ldots$ tendent vers un élément $C$ de $E$, on a:
$$
U(C)=\lim _{n=\infty} U\left(C_{n}\right) .
$$

En effet, observons d'abord qu'il n'y a pas, d'après ce qui précède, une infinité d'éléments de la suite $C_{1}, C_{2}, \ldots$ appartenant à des ensembles $E_{p}$ distincts. Alors:

$1^{\circ}$ Ou bien $C$ est dans $G$, c'est-à-dire que l'on a, quel que soit $p$ :
$$
\left(C, A_{p}\right)>\alpha_{p} .
$$
Or :
$$
\left(C_{n}, A_{p}\right) \geqslant\left(C, A_{p}\right)-\left(C, C_{n}\right)=\alpha_{p}+\left[\left(C, A_{p}\right)-\alpha_{p}-\left(C, C_{n}\right)\right] ;
$$
d'autre part, on aura, pour $n$ assez grand:
$$
\left(C, C_{n}\right)<\left(C, A_{p}\right)-\alpha_{p},
$$
d'où, en combinant ces deux inégalités :
$$
\left(C_{n}, A_{p}\right)>\alpha_{p} .
$$

Donc, à partir d'un certain rang $C_{n}$ est dans $G$. Alors on a:
$$
U\left(C_{n}\right)=0, \quad U(C)=0,
$$
d'où:
$$
U(C)=\lim _{n=\infty} U\left(C_{n}\right) ;
$$

$2^{\circ}$ Ou bien $C$ est dans $E_{p}$ et on a: $\left(C, A_{p}\right) \leqslant \alpha_{p}$. Alors deux cas se présentent:

\textit{a)} $\left(C, A_{p}\right)<\alpha_{p}$; on voit comme précédemment qu'à partir d'un certain rang $C_{n}$ est constamment dans $E_{p}$. Alors:
$$
\left|U(C)-U\left(C_{n}\right)\right|=\left|\left(C_{n}, A_{p}\right)-\left(C, A_{p}\right)\right| \cfrac{p}{\alpha_{p}} \leqslant\left(C, C_{n}\right) \cfrac{p}{\alpha_{p}} \,.
$$
Donc:
$$
U(C)=\lim _{n=\infty} U\left(C_{n}\right) \,.
$$

\textit{b)} $\left(C, A_{p}\right)=\alpha_{p}$. Alors, à partir d'un certain rang il n'y a plus dans la suite $C_{1}$, $C_{2}, \ldots$ que des éléments de $G$ : $C_{n_{1}}, C_{n_{2}}, \ldots$ et des éléments de $E_{p}: C_{q_{1}}, C_{q_{2}}, \ldots$. On voit comme précédemment que:
$$
U(C)=\lim _{r=\infty} U\left(C_{q_{r}}\right) \,.
$$
D'autre part, on aura:
$$
U(C)=0, \quad U\left(C_{n_{r}}\right)=0,
$$
d'où:
$$
U(C)=\lim _{r=\infty} U\left(C_{n_{r}}\right) .
$$
D'où, en combinant:
$$
U(C)=\lim _{n=\infty} U\left(C_{n}\right) .
$$
Ainsi $U$ est bien une opération non bornée, continue en tout élément de $G$.

\newpage
\section*{DEUXIÈME PARTIE.}
\section*{APPLICATIONS DE LA THÉORIE GÉNÉRALE.}

\textbf{52.}
La méthode que nous aurons à employer pour appliquer la théorie générale aux cas particuliers obtenus en spécifiant la nature des éléments, s'indique d'elle-même. Dans tous les exemples qui suivront, nous commencerons par définir la classe d'éléments sur laquelle nous aurons à opérer; en particulier nous donnerons une règle permettant de discerner les éléments distincts, ce qui n'est pas toujours aussi simple qu'on pourrait le croire (voir $\mathrm{n}^{\text {os }} 76-77$). Puis nous montrerons qu'on peut considérer la définition ordinaire de la limite de ces éléments comme rentrant dans la définition que nous avons donnée à l'aide de l'écart (cas particulier du voisinage, $\mathrm{n}^{\circ}$ 49). Nous prouverons enfin que la classe $(E)$, ainsi obtenue, est normale ($\mathrm{n}^{\circ}$ 37). \textit{Ceci fait, il n'y aura plus qu'à répéter les théorèmes généraux de la \textsc{Première Partie} énoncés dans le langage qui correspond à la classe considérée.} Enfin, nous donnerons dans chaque cas une condition nécessaire et suffisante pour qu'un ensemble soit compact ($\mathrm{n}^{\circ}$ 9). Cela revient à remplacer la définition générale de l'ensemble compact par une définition d'une apparence moins abstraite, mais particulière à chaque cas.

\section*{Chapitre III.}
\subsection*{Les ensembles linéaires et les fonctions d'une variable.}

\textbf{53.}
Prenons comme éléments les points d'une droite (ou les nombres qui représentent leurs abscisses). On sait discerner les éléments de cette classe qui sont distincts. Si l'on appelle écart de deux d'entre eux leur distance, on voit que cette définition répond bien aux conditions \textit{a)}, \textit{b)}, imposées à la notion d'écart, $\mathrm{n}^{\circ}$ 49. De plus, la définition ordinaire de la limite d'une suite de points coïncide avec celle qu'on déduit de cette définition de l'écart.

La classe $(E)$ ainsi définie est normale. En effet, le théorème de \textsc{Cauchy} (n$^{\circ}$ 37) a été démontré précisément dans ce cas. D'autre part, on sait que l'ensemble des points d'une droite peut être considéré comme l'ensemble dérivé de l'ensemble dénombrable des points d'abscisses rationnelles.

On sait d'ailleurs que tout ensemble linéaire limité et comprenant une infinité de points, donne lieu à au moins un point limite. Inversement, nous avons démontré ($\mathrm{n}^{\circ}$ 35) que tout ensemble compact tiré d'une classe $(V)$ est limité. Par suite, dans le cas des ensembles linéaires, la notion d'ensemble compact se confond avec celle d'ensemble limité.

\textit{Si maintenant nous appliquons nos théorèmes généraux, nous retrouvons la plupart des théorèmes classiques de la théorie des ensembles linéaires et des fonctions continues d'une variable.} (Voir par exemple I, II).\\

\textbf{54.} 
Nous devons même remarquer que nous obtenons ainsi un peu plus. En effet, dans la théorie classique, on est naturellement amené à se borner aux ensembles de points d'un même intervalle et on oublie que les ensembles illimités ont quelquefois des propriétés différentes. Au contraire, nous avons vu dans la théorie générale que les propriétés particulières des ensembles compacts intervenaient constamment dans les démonstrations et d'une façon apparente.

Ainsi, par exemple, considérons des fonctions $f_{1}(x), f_{2}(x), \ldots$ continues \textit{pour toute valeur} de $x$ et qui convergent quel que soit $x$ vers $f(x)$. A quelle condition $f(x)$ est-elle continue? M. \textsc{Arzelà} ($\mathrm{n}^{\circ}$ 14) ne s'est pas occupé de ce cas; si l'on généralise son résultat sans précautions, on serait tenté de dire : pour que $f(x)$ soit continue, il faut et il suffit que, étant donnés deux nombres positifs $\varepsilon$ et $N$, on puisse en trouver un troisième $N^{\prime} \geqslant N$, tel que, pour toute valeur de $x$, il existe un entier $n_{x}$ vérifiant les inégalités
$$
N \leqslant n_{x} \leqslant N^{\prime}, \quad\left|f_{n_{x}}(x)-f(x)\right|<\varepsilon\,.
$$

Or, ce serait une erreur; il suffit pour le voir de prendre $f_{n}(x)=e^{-\frac{n}{1+x^{2}}}$. D'ailleurs la difficulté se lève comme dans le cas général. Pour que $f(x)$ soit continue, il faut et il suffit que la convergence soit quasi-uniforme ($\mathrm{n}^{\circ}$ 14) \textit{dans tout intervalle limité}.

De même, on pourrait être tenté de généraliser un autre résultat de M. \textsc{Arzelà} (n$^{\circ}$ 15) en énonçant ainsi la condition nécessaire et suffisante pour que des fonctions $f(x)$ continues quelque soit $x$ soient telles que, d'une infinité quelconque d'entre elles, on puisse extraire une suite convergente : il faut et il suffit que, $1^{\circ}$ ces fonctions soient bornées dans leur ensemble, $2^{\circ}$ à tout nombre $\varepsilon>0$ on puisse faire correspondre un nombre $\eta$ tel que l'inégalité $\left|x^{\prime}-x^{\prime \prime}\right|<\eta$ entraîne pour toutes les fonctions $f(x)$ :
$$
\left|f\left(x^{\prime}\right)-f\left(x^{\prime \prime}\right)\right|<\varepsilon .
$$

Or aucune de ces deux conditions n'est nécessaire, comme le montre l'exemple des fonctions $f_{n}(x)=x^{2}+\cfrac{1}{n}$, où $n$ prend toutes les valeurs entières positives. Au contraire, de nos théorèmes généraux nous pouvons conclure que la condition nécessaire et suffisante est que les fonctions doivent être bornées et également continues en tout point $x$ pris isolément (voir $\mathrm{n}^{\circ}$ 15). De plus, si ces conditions sont remplies, la convergence sera uniforme dans tout segment limité.\\

\textbf{55.} 
\textsc{\textbf{Remarque.}} --- La plupart des théorèmes classiques sur les ensembles linéaires et les fonctions d'une variable s'étendent immédiatement aux ensembles de points de l'espace à $2,3, \ldots, n, \ldots$ dimensions et aux fonctions de $2,3, \ldots, n, \ldots$ variables. C'est même pour la plupart d'entre eux la seule généralisation qu'on en avait- faite. L'analogie qu'on avait ainsi observée est beaucoup plus profonde si l'on se place à notre point de vue général.

Pour obtenir ces théorèmes, il suffit de procéder comme plus haut en appelant écart de deux éléments $\left(x_{1}, x_{2}, \ldots, x_{n}\right)$ et $(x_{1}^{\prime}, x_{2}^{\prime}, \ldots, x_{n}^{\prime})$ la quantité :
$$
\sqrt{\left(x_{1}-x_{1}^{\prime}\right)^{2}+\cdots+\left(x_{n}-x_{n}^{\prime}\right)^{2}} \,.
$$

\section*{Chapitre IV.}
\subsection*{Les ensembles de fonctions continues et les fonctionnelles.}

\textbf{56.}
Prenons comme éléments variables les fonctions de $x$ uniformément continues dans un intervalle déterminé $J$. Nous considérerons bien entendu comme distinctes deux fonctions dont la différence n'est pas partout nulle dans $J$.

Il y a ici deux définitions classiques de la limite, nous n'envisagerons que la limite dite uniforme\footnote{On dit qu'une fonction $f_n(x)$ tend uniformément vers $f(x)$ dans $J$, si a tout nombre $\varepsilon>0$ on
peut faire correspondre un entier $p$ tel que l’inégalité $n>p$ entraîne: $|f_n(x)-f(x)|<\varepsilon$ \textit{pour route valeur} de $x$ de l'intervalle $J$ (voir n$^\circ$ 13).}. Nous pouvons considérer cette définition comme une conséquence de la définition suivante de l'écart de deux fonctions $f(x), g(x)$ uniformément continues dans $J$: \textit{Cet écart $(f, g)$ est le maximum de $|f(x)-g(x)|$ dans $J$}. Cette définition bien naturelle semble avoir été employée pour la première fois d'une manière systématique par \textsc{Weierstrass}. Elle satisfait bien aux conditions générales \textit{a)}, \textit{b)} du $\mathrm{n}^{\circ}$ 49. La classe $(E)$ ainsi définie est normale. En effet, on sait d'abord qu'elle admet une généralisation du théorème de \textsc{Cauchy} relatif à la convergence d'une suite. D'autre part, on peut former, une fois pour toutes, une suite $S$ de fonctions uniformément continues dans $J$ :
$$
f_{1}(x), f_{2}(x), \ldots
$$
telle que toute fonction continue dans $J$ en soit la limite uniforme. Par exemple, on peut prendre pour former la suite $S$, l'ensemble évidemment dénombrable des fonctions continues qui prennent des valeurs rationnelles en chacun des points de division de $J$ en $q$ parties égales ($q$ étant arbitraire) et qui sont linéaires dans chacune de ces divisions. 
Alors, étant donnée une fonction $f(x)$ continue dans $J$, si l'on prend dans cet ensemble la fonction $f_{n_{q}}(x)$ qui prend en chaque point de division une valeur égale à la valeur approchée par défaut de $f(x)$ à $\cfrac{1}{q}$ près, on voit facilement que la suite $f_{n_{1}}(x), f_{n_{2}}(x), \ldots f_{n_{q}}(x), \ldots$ extraite de $S$ converge uniformément vers $f(x)$\footnote{On pourrait aussi procéder comme au n$^{\circ}$ 72 en utilisant le développement d'une fonction continue en série de polynômes (\textsc{ii}, page 50).}.

Cette remarque peut s'énoncer de la façon suivante, en posant
$$
u_{1}(x)=f_{1}(x), \ldots, u_{q}(x)=f_{q}(x)-f_{q-1}(x), \ldots:
$$

\textit{
On peut former, une fois pour toutes, une série de fonctions uniformément continues dans $J$:
$$
u_{1}(x)+u_{2}(x)+\cdots+u_{q}(x)+\cdots
$$
telle qu'en groupant convenablement ses termes on puisse la faire tendre uniformément vers n'importe quelle fonction continue dans $J$.}\\

\textbf{57.} 
D'après notre définition de la limite, le théorème d'\textsc{Arzelà} sur les fonctions continues (qui se déduit dans le Chapitre précédent de nos théorèmes généraux) nous permet d'affirmer que la condition nécessaire et suffisante pour qu'un ensemble de fonctions uniformément continues dans $J$ soit compact est que ces fonctions soient en chaque point de $J$ bornées et également continues. Nous n'avons plus maintenant aucune difficulté à appliquer nos théorèmes généraux aux ensembles de fonctions continues dans $J$ \textit{en nous souvenant que la limite dont il s'agit dans ce qui suit est la limite \textsc{uniforme}.}

\textsc{\textbf{Théorème.}} --- \textit{Étant donné un ensemble quelconque $E$ de fonctions uniformément continues dans $J$, on peut extraire de $E$ une suite dénombrable d'éléments telle que tout élément de $E$ appartienne à cette suite ou soit un de ses éléments limites} (n$^{\circ}$ 45). On sait aussi que l'ensemble dérivé de $E$ est fermé\footnote{Nous savons ($\mathrm{n}^{\circ}$ 22) qu'il n'en serait plus ainsi, si l'on avait pris la définition de la limite dans son sens ordinaire, c'est-à-dire sans la supposer nécessairement uniforme.}.

\textsc{\textbf{Théorème.}} --- \textit{Si ce même ensemble $E$ est non dénombrable, il donne lieu à au moins un élément de condensation} ($\mathrm{n}^{\circ}$ 43). Remarquons que la définition générale des éléments de condensation peut se traduire ici de la façon suivante : Un élément $f(x)$ est un élément de condensation de $E$ si, quel que soit $\varepsilon>0$, il y a une infinité non dénombrable d'éléments $\varphi(x)$ de $E$ tels que $f(x)-\varepsilon<\varphi(x)<f(x)+\varepsilon$.

\textsc{\textbf{Théorème.}} --- \textit{Soit $F$ un ensemble fermé de fonctions uniformément continues dans un intervalle $J$. $1^{\circ}$ On peut toujours décomposer cet ensemble en un ensemble dénombrable et un ensemble parfait ou nul} ($\mathrm{n}^{\circ}$ 44). \textit{$2^{\circ}$ Si $F$ fait partie d'un ensemble $B$ de fonctions qui sont en chaque point de $J$ également continues et bornées, on pourra extraire de $B$ une suite d'éléments $f_{1}(x), f_{2}(x), \ldots$ et former une suite de nombres positifs $\varepsilon_{1}, \varepsilon_{2}, \ldots$ telles que l'on obtienne $F$ en supprimant de $B$ les fonctions $f(x)$ qui vérifient \textsc{l'une} des inégalités suivantes:}
$$f_{1}(x)-\varepsilon<f(x)<f_{1}(x)+\varepsilon, \ldots, f_{n}(x)-\varepsilon<f(x)<f_{n}(x)+\varepsilon, \ldots \quad \left(\mathrm{n}^{\mathrm{o}} \;34\right).$$

\textsc{\textbf{Théorème.}} --- \textit{Soit $B$ un ensemble \textsc{fermé} de fonctions également continues et bornées en tout point d'un intervalle $J$. S'il existe une famille $H$ d'ensembles $I$ de fonctions de $B$, telle que toute fonction de $B$ est intérieure au sens étroit à l'un au moins de ces ensembles, on peut extraire de $H$ un nombre fini d'ensembles $I$ formant une famille $G$ jouissant de la même propriété que $H$. La réciproque est vraie} ($\mathrm{n}^{\circ}$ 42).\\

\textbf{58.} 
En particularisant la question que nous avons résolue au n$^{\circ}$ 39, on obtient le problème posé par M. \textsc{Hadamard} en ces termes: « Soit $E$ l'ensemble des fonctions continues entre 0 et 1, ayant des valeurs déterminées aux extrémités, ou remplissant des conditions analogues. Divisons $E$ en ensembles partiels $k_{\varepsilon}$ tels que deux fonctions quelconques appartenant à $E$ aient un écart moindre que $\varepsilon$. Considérant les $k_{\varepsilon}$ comme autant d'individus, on peut dire que l'ensemble $\mathfrak{K}_\varepsilon$, qui a ces $k_{\varepsilon}$ comme éléments, \textit{numère} l'ensemble $E$. C'est cet ensemble $\mathfrak{K}_\varepsilon$ dont il conviendrait d'étudier les propriétés et en particulier la puissance ».

La théorie générale appliquée ici nous permet de donner à ce problème une solution complète en ce qui concerne la puissance, et même il nous est indifférent de supposer ou non que les valeurs des fonctions soient ou non données aux extrémités. La réponse est la suivante: \textit{Quel que soit un ensemble $E$ de fonctions uniformément continues dans un intervalle $J$, on peut toujours choisir sa décomposition en ensembles $k_{\varepsilon}$ de façon que $\mathfrak{K}_\varepsilon$ soit dénombrable} ($\mathrm{n}^{\circ}$ 40). \textit{Pour que $\mathfrak{K}_\varepsilon$ non seulement soit dénombrable mais se compose d'un nombre fini de termes quel que soit $\varepsilon$, il faut et il suffit que les fonctions appartenant à $E$ soient en chaque point de $J$ bornées et également continues} ($\mathrm{n}^{\circ}$ 41). Dans les deux cas, on pourra choisir les $k_{\varepsilon}$ de façon que chaque élément de $E$ soit intérieur au sens étroit à au moins l'un d'eux. De plus, nous connaissons un moyen effectif de déterminer les $k_{\varepsilon}$ dans le cas général et cela indépendamment de $E$.\\

\textbf{59.} 
Les opérations portant sur des fonctions continues sont spécialement appelées des \textit{fonctionnelles} par M. \textsc{Hadamard} (\textsc{xi}). Un exemple important de fonctionnelle continue est la fonctionnelle linéaire:
$$
U(f)=\int_{a}^{b} m(x) f(x) d x
$$
où $m(x)$ est une fonction bornée intégrable dans l'intervalle $(a, b)$.

Nous pouvons appliquer encore ici nos théorèmes généraux sur les opérations.

\textsc{\textbf{Théorème.}} --- Soit $U$ une fonctionnelle continue dans un ensemble fermé $B$ de fonctions de $x$ bornées et également continues en tout point d'un intervalle $J$. Cette fonctionnelle : $1^{\circ}$ est bornée dans $B$; 2$^{\circ}$ y atteint au moins une fois sa limite supérieure ($\mathrm{n}^{\circ}$ 11). \textit{Réciproquement, si cette circonstance a lieu pour toute fonctionnelle continue dans $B$, $B$ est un ensemble fermé de fonctions également continues et bornées en tout point de $J$} ($\mathrm{n}^{\circ}$ 51).

\textsc{\textbf{Théorème.}} --- Pour qu'une suite de fonctionnelles $U_{1}, U_{2}, \ldots$, continues dans un champ quelconque $E$ de fonctions de $x$ uniformément continues dans $J$, converge vers une fonctionnelle continue dans $E$, il faut et il suffit que la convergence soit quasi-uniforme dans tout ensemble fermé formé de fonctions également continues et bornées appartenant à $E$ ($\mathrm{n}^{\circ}$ 14).

\textsc{\textbf{Théorème.}} --- Considérons une famille $\mathfrak{K}_\varepsilon$ de fonctionnelles continues dans un ensemble fermé de fonctions également continues et bornées en tout point d'un intervalle $J$. Pour que de toute infinité de fonctionnelles de $\mathfrak{K}_\varepsilon$, on puisse extraire une suite qui converge uniformément, il faut et il suffit que les fonctionnelles de $\mathfrak{K}_\varepsilon$ soient bornées et également continues en tout élément de l'ensemble de fonctions ($\mathrm{n}^{\circ}$ 48).

\section*{Chapitre V.}
\subsection*{Les ensembles et les fonctions de points de l'espace à une infinité dénombrable de dimensions.}

\textbf{60.}
Un grand nombre des éléments qui interviennent en mathématiques sont déterminés chacun complètement par une suite infinie de nombres réels ou complexes: Par exemple, une série de \textsc{Taylor} est déterminée par la suite de ses coefficients sous la forme:
\begin{equation*}
f(x)=a_{0}+a_{1} x+\cdots+a_{n}(x)+\cdots \tag{\textsc{i}}
\end{equation*}

Une fonction continue de $x$ entre $0$ et $1$ est déterminée par la suite des valeurs qu'elle prend aux points d'abscisses rationnelles, par la formule d'interpolation de M. \textsc{Borel} (\textsc{ii}, page 80):
$$
\varphi(x)=\lim _{q=\infty} \sum_{p=0}^{p=q} \varphi\left(\cfrac{p}{q}\right) M_{p, q}(x) \,.
$$

De même, un nombre irrationnel est défini par une suite de nombres rationnels; et ainsi de suite.

On peut donc considérer les nombres de la suite qui définit chacun de ces éléments comme les coordonnées de cet élément envisagé comme un point d'un espace $(E_{\omega})$ à une infinité dénombrable de dimensions. Il y a plusieurs avantages à opérer ainsi. D'abord l'avantage qui se présente toujours quand on emploie le langage géométrique si propice à l'intuition par les analogies qu'il fait naître. Ensuite cela permet d'obtenir des propriétés générales applicables à toutes ces catégories d'éléments: celles qui résultent non de leur nature propre, mais de leur détermination par un ensemble dénombrable de nombres. Il reste d'ailleurs bien entendu qu'à toute suite infinie de nombres ne correspond pas nécessairement un de ces éléments. Par exemple, l'expression (\textsc{i}) ne définit $f(x)$ que si la suite $a_{0}, a_{1}, \ldots, a_{n}, \ldots$ satisfait à certaines conditions.\\

\textbf{61.} 
Nous allons donc maintenant faire abstraction de l'origine de la suite de nombres qui définit un de ces éléments et considérer simplement cette suite:
$$
x_{1}, x_{2}, \ldots, x_{n}, \ldots
$$
comme définissant un point déterminé $x$ de l'espace.

Nous dirons que deux points $x, x^{\prime}$ de $(E_{\omega})$ coïncident, lorsque leurs coordonnées sont respectivement égales, et dans ce cas seulement.

Pour pouvoir appliquer dans le cas présent les théorèmes généraux obtenus précédemment, il nous suffira de montrer que \textit{la classe des points de $(E_{\omega})$ définit une classe $(E)$ normale.
}\\

\textbf{62.} 
\textit{\textbf{Écart de deux points de}} $\left(E_{\omega}\right)$. --- On pourrait définir de bien des manières l'écart de deux points:
$$
\begin{array}{cll}
x: & x_{1}, & x_{2}, \ldots, x_{n}, \ldots \\
x^{\prime}: & x_{1}^{\prime}, & x_{2}^{\prime}, \ldots, x_{n}^{\prime}, \ldots
\end{array}
$$

Mais pour généraliser utilement le cas de l'espace à un nombre fini de dimensions, il faut s'arranger pour que, si l'écart ($x, x^{\prime}$) tend vers zéro, chacune des quantités $x_{1}-x_{\mathrm{t}}^{\prime},\, x_{2}-x_{2}^{\prime},\, \ldots, x_{n}-x_{n}^{\prime}, \ldots$ tende vers zéro.

Une question importante se pose, à savoir s'il ne serait pas utile de choisir cette définition de façon que cette suite infinie de différences tende \textit{uniformément} vers zéro. Nous verrons plus loin ($\mathrm{n}^{\mathrm{o}}$ 68) qu'il est préférable de ne pas s'imposer cette condition qui semble assez naturelle. Quoiqu'il en soit, nous adopterons la définition suivante de l'écart, dont le choix sera justifié par la suite.

Nous appellerons écart des deux points $x, x^{\prime}$, le nombre bien défini:
$$
\left(x, x^{\prime}\right)=\cfrac{\left|x_{1}-x_{1}^{\prime}\right|}{1+\left|x_{1}-x_{1}^{\prime}\right|}+\cfrac{1}{2!}\, \cfrac{\left|x_{2}-x_{2}^{\prime}\right|}{1+\left|x_{2}-x_{2}^{\prime}\right|}+\cdots+\cfrac{1}{n!}\, \cfrac{\left|x_{n}-x_{n}^{\prime}\right|}{1+\left|x_{n}-x_{n}^{\prime}\right|}+\cdots
$$

Le second membre est évidemment convergent quels que soient $x_{1}, x_{1}^{\prime} ; x_{2}, x_{2}^{\prime} ; \ldots$ On voit qu'il est toujours $>0$ lorsque $x$ et $x^{\prime}$ sont distincts. De plus, on a, quel que soit $n$:
$$
\cfrac{\left|x_{n}^{\prime}-x_{n}^{\prime \prime}\right|}{1+\left|x_{n}^{\prime}-x_{n}^{\prime \prime}\right|} \leqslant \cfrac{\left|x_{n}-x_{n}^{\prime}\right|}{1+\left|x_{n}-x_{n}^{\prime}\right|}+\cfrac{\left|x_{n}-x_{n}^{\prime \prime}\right|}{1+\left|x_{n}-x_{n}^{\prime \prime}\right|}\,,
$$
comme il est facile de le vérifier.

Donc on a pour trois points quelconques $x, x^{\prime}, x^{\prime \prime}$ :
$$
\left(x^{\prime}, x^{\prime \prime}\right) \leqslant\left(x, x^{\prime}\right)+\left(x, x^{\prime \prime}\right)\,.
$$

Ainsi le nombre que nous venons de définir satisfait bien aux deux conditions générales que nous avions imposées à la définition de l'écart ($\mathrm{n}^{\mathrm{o}}$ 49).\\

\textbf{63.} 
\textit{\textbf{Limite d'un point de}} $\left(E_{\omega}\right)$. --- De la définition de l'écart résulte la définition de la limite d'un point de l'espace $(E_{\omega})$.

On dit qu'un point $x^{(n)}$ de l'espace $(E_{\omega})$ tend vers le point $x$ de $(E_{\omega})$, quand $n$ croît indéfiniment, si l'écart $\left(x^{(n)}, x\right)$ tend vers zéro avec $\cfrac{1}{n}$. Mais on peut donner une définition équivalente faisant intervenir directement les coordonnées, au moyen du théorème suivant:

\textsc{\textbf{Théorème.}} --- \textit{La condition nécessaire et \textsc{suffisante} pour qu'un point de $(E_{\omega})$}
$$x^{(n)}:  x_{1}^{(n)}, \, x_{2}^{(n)}, \ldots, x_{p}^{(n)}, \ldots$$
\textit{tende vers un point:}
$$x: x_{1}, \, x_{2}, \ldots, x_{p}, \ldots,$$
\textit{est que, quel que soit $p,\, x_{p}^{(n)}$ tende vers $x_{p}$ quand $n$ croit indéfiniment.}

En effet, supposons d'abord que cette dernière condition soit réalisée. Je vais montrer que ($x,\, x^{(n)}$) tend vers zéro. Pour cela observons qu'on a:
\begin{equation*}
\left(x, x^{(n)}\right) \leqslant \cfrac{\left|x_{1}-x_{1}^{(n)}\right|}{1+\left|x_{1}-x_{1}^{(n)}\right|}+\cdots+\cfrac{1}{p!}\, \cfrac{\left|x_{p}-x_{p}^{(n)}\right|}{1+\left|x_{p}-x_{p}^{(n)}\right|}+r_{p}, \tag{2}
\end{equation*}
en appelant $r_{p}$ l'expression indépendante de $n$:
$$
r_{p}=\cfrac{1}{(p+1)!}+\cfrac{1}{(p+2)!}+\cdots
$$

Cette dernière quantité tend vers zéro avec $\cfrac{1}{p}$; on peut donc fixer un nombre $p$ indépendant de $n$, tel que l'on ait $r_{p}<\cfrac{\varepsilon}{2}$. Le nombre $p$ étant ainsi \textit{fixé}, il est manifeste que la somme des $p$ termes qui le précèdent dans l'inégalité (2) tend vers zéro quand $n$ croît indéfiniment. On peut donc trouver un nombre $q$ tel que leur somme soit inférieure à $\cfrac{\varepsilon}{2}$ pour $n>q$. En résumé, nous obtenons un nombre $q$ tel que l'on ait:
$$
\left(x^{(n)}, x\right)<\varepsilon, \quad \text { pour } n>q ;
$$
ce qui démontre que la condition supposée était bien suffisante.

Démontrons qu'elle est nécessaire. L'expression de ($x, x^{(n)}$) montre que l'on a pour toute valeur de $p$ :
$$
\cfrac{\left|x_{p}-x_{p}^{(n)}\right|}{1+\left|x_{p}-x_{p}^{(n)}\right|}<p!\left(x, x^{(n)}\right) .
$$

Donc le premier membre tend vers zéro lorsque, $p$ restant fixe, $n$ croit indéfiniment. Ceci ne peut arriver que si $x_{p}^{(n)}$ tend vers $x_{p}$ pour toute valeur fixe de $p$.\\

\textbf{64.} 
Cette proposition permet de montrer que la classe $(E_{\omega})$ admet une généralisation du théorème de \textsc{Cauchy} :

\textsc{\textbf{Théorème.}} --- 
\textit{La condition nécessaire et suffisante pour qu'une suite infinie de points de l'espace $(E_{\omega})$:}
$$
x^{(1)}, \quad x^{(2)}, \ldots, x^{(n)}, \ldots
$$
\textit{ait une limite, est que, quel que soit le nombre $\varepsilon>0$, on puisse déterminer un nombre $n$ tel que l'on ait:
$$
\left(x^{(n+p)}, x^{(n)}\right)<\varepsilon,
$$
quel que soit l'entier $p$.}

La condition est évidemment nécessaire.

Inversement, supposons la condition réalisée. On aura:
$$
\cfrac{\left|x_{q}^{(n)}-x_{q}^{(n+p)}\right|}{1+\left|x_{q}^{(n)}-x_{q}^{(n+p)}\right|}<\varepsilon q!
$$
D'où:
$$
\left|x_{q}^{(n)}-x_{q}^{(n+p)}\right|<\cfrac{\varepsilon q!}{1-\varepsilon q!}\,,
$$
en supposant $\varepsilon<\cfrac{1}{q!}$. Ayant une fois fixé $q$, on pourra prendre $\varepsilon$ de façon que
$$
\varepsilon<\cfrac{1}{q!} \quad \text { et } \quad \cfrac{\varepsilon q!}{1-\varepsilon q!}<\omega\,,
$$
$\omega$ étant donné à l'avance; alors $\varepsilon$ déterminera $n$ et on aura:
$$
\left|x_{q}^{(n)}-x_{q}^{(n+p)}\right|<\omega,
$$
quel que soit $p$. D'après un théorème bien connu de \textsc{Cauchy}, il en résulte que la suite des nombres:
$$
x_{q}^{(1)}, \quad x_{q}^{(2)}, \ldots, x_{q}^{(n)}, \ldots
$$
a une limite $x_{q}$ lorsque $n$ croît indéfiniment. Et ceci a lieu quel que soit $q$. D'après le théorème précédent, cela prouve que la suite $x^{(1)}, \ldots, x^{(n)}, \ldots$ a une limite déterminée $x: x_1, \ldots, x_{q}, \ldots$

\subsection*{Les ensembles de points de l'espace $(E_{\omega})$.}

\textbf{65.}
Du fait que l'on peut définir l'écart de deux points de l'espace $(E_{\omega})$ à une infinité dénombrable de dimensions, il résulte que les points de cet espace forment une classe $(E)$. Nous compléterons de plus l'assimilation à la théorie générale par le théorème suivant:

\textsc{\textbf{Théorème.}} --- \textit{Les points de l'espace $(E_{\omega})$ forment une classe $(E)$ normale.}

Nous savons déjà qu'ils forment une classe $(E)$ admettant une généralisation du théorème de \textsc{Cauchy} sur les suites convergentes. Cette classe $(E)$ est évidemment parfaite. Il suffit de montrer qu'on peut la considérer comme l'ensemble dérivé d'une suite dénombrable de ses éléments. Pour cela remarquons d'abord que l'ensemble des nombres rationnels de signe quelconque est un ensemble dénombrable qu'on peut mettre sous la forme d'une suite:
$$
c_{1}, \, c_{2}, \ldots, c_{n}, \ldots
$$

Considérons alors l'ensemble $D$ des points de l'espace $(E_{\omega})$ qui ont des coordonnées de la forme:
$$
x_{1}=c_{n_{1}}, \quad x_{2}=c_{n_{2}}, \ldots, x_{p}=c_{n_{p}}, \quad x_{p+1}=0, \quad x_{p+2}=0, \ldots,
$$
où $p, n_{1}, n_{2}, \ldots, n_{p}$ sont des entiers positifs quelconques. Cet ensemble est évidemment dénombrable et on voit facilement que tout point de $(E_{\omega})$ est limite d'une suite d'éléments de $D$.\\

\textbf{66.} 
\textit{\textbf{Les ensembles compacts.}} --- La notion d'ensemble compact prend une signification géométrique très simple dans le cas d'un ensemble de points de $(E_{\omega})$. Pour l'indiquer, nous dirons d'abord qu'\textit{un ensemble de points de $(E_{\omega})$ est contenu dans un domaine fini}, si l'on peut trouver une suite de nombres $\geqslant 0: M_{1}, M_{2}, \ldots$ tels que l'on ait pour tout point ($x_{1}, \ldots, x_{n}, \ldots$) de l'ensemble:
$$
\left|x_{1}\right| \leqslant M_{1}, \quad\left|x_{2}\right| \leqslant M_{2}, \ldots,\left|x_{n}\right| \leqslant M_{n}, \ldots
$$

\textsc{\textbf{Théorème.}} --- \textit{La condition nécessaire et suffisante pour qu'un ensemble $E$ de points de l'espace $(E_{\omega})$ soit compact est que cet ensemble soit contenu dans un domaine fini.}

En effet, supposons l'ensemble $E$ compact; s'il n'était pas dans un domaine fini, on pourrait trouver $n$ tel que l'ensemble des coordonnées de rang $n$ des points de $E$ ne soit pas borné. Autrement dit, il faudrait que, quel que soit $p$, on puisse trouver un point $x^{(p)}$ de $E$ tel que, en appelant $x_{n}^{(p)}$ sa coordonnée de rang $n$, on ait:
$$
\left|x_{n}^{(p)}\right|>p .
$$

Or ceci est impossible si $E$ est compact; car, de la suite des points de $E: x^{(1)}$, $x^{(2)}, \ldots$ on pourrait extraire une suite $x^{\left(p_{1}\right)}, x^{\left(p_{2}\right)}, \ldots$ ayant une limite $x$. Et alors les nombres $x_{n}^{\left(p_{1}\right)}, x_{n}^{\left(p_{2}\right)}, \ldots$ qui croissent indéfiniment comme $p_{1}, p_{2}, \ldots$ auraient une limite finie $x_{n}$.

Inversement, supposons que $E$ soit dans un domaine fini. Alors, ou bien il n'y a qu'un nombre fini d'éléments et dans ce cas $E$ est compact par définition, ou bien il y a un nombre infini d'éléments distincts. Considérons un ensemble infini $E_{1}$ contenu dans $E$. L'ensemble de ses coordonnées de rang i est borné par hypothèse. Donc: ou bien il y en a une infinité qui sont égales à un même nombre $x_{1}$, ou bien on peut en trouver une infinité qui sont distinctes et tendent vers un nombre déterminé $x_{1}$. Dans les deux cas, on pourra extraire de $E_{1}$ une suite de points de $\left(E_{\omega}\right)$:
$$
x^{(1)}, \quad x^{(2)}, \ldots, x^{(n)}, \ldots,
$$
telle que la suite $x_{1}^{(1)}, x_{1}^{(2)}, \ldots, x_{1}^{(n)}, \ldots$ ait une limite déterminée $x_{1}$. De cette première suite, on pourra extraire une autre suite de points rangés dans le même ordre:
$$
x^{(1,2)}, \quad x^{(2,2)}, \ldots, x^{(n, 2)}, \ldots,
$$
telle que les coordonnées du deuxième rang aient une limite déterminée $x_{2}$, les coordonnées du premier rang continuant à tendre vers $x_{1}$. Et ainsi de suite. On arrivera à former une suite de points de $E_{1}$:
$$
x^{(1, p)}, \quad x^{(2, p)}, \ldots, x^{(n, p)}, \ldots
$$
contenue dans les suites précédemment formées et telle que les coordonnées de rang au plus égal à $p$ aient respectivement des limites déterminées : $x_{1}, x_{2}, \ldots, x_{p}$.

Alors, considérons la suite de points de $E_{1}$ distincts:
\begin{equation*}
x^{(1)}, \quad x^{(2,2)}, \ldots, x^{(n, n)}, \ldots \tag{Σ}
\end{equation*}
A partir du rang $p$, et ceci quel que soit $p$, cette suite est formée d'éléments de la suite $x^{(1, p)}, x^{(2, p)}, \ldots, x^{(n, p)}, \ldots$ pris dans le même ordre. Donc ses coordonnées de rang $p$ tendent, quel que soit $p$, vers un nombre déterminé $x_{p}$. Autrement dit, la suite (Σ) est une suite d'éléments de $E_{1}$ qui sont distincts et ont une limite déterminée: le point de coordonnées
$$
x_{1}, \quad x_{2}, \ldots, x_{p}, \ldots
$$

La proposition est ainsi démontrée\footnote{M. \textsc{Montel} est depuis longtemps en possession de la condition suffisante qui lui a servi pour établir certaines propositions énoncées dans une Note des Comptes Rendus (\textsc{xxv})}.

\subsection*{Applications des théorèmes généraux.}

\textbf{67.}
 Il n'y a plus maintenant aucune difficulté à appliquer aux ensembles de points de l'espace $(E_{\omega})$ les théorèmes énoncés pour les ensembles tirés d'une classe $(E)$ normale.

\textsc{\textbf{Théorème.}} --- \textit{Considérons un ensemble quelconque $E$ de points de l'espace $(E_{\omega})$ à une infinité dénombrable de dimensions: $1^{\circ}$ on peut extraire de $E$ un ensemble dénombrable de points, $D$, tel que tout point de $E$ appartienne, soit à $D$, soit à son dérivé $D^{\prime}$; $2^{\circ}$ l'ensemble $E^{\prime}$ dérivé de $E$ est fermé ; $3^{\circ}$ l'ensemble $E$ est dénombrable ou sinon donne lieu à au moins un point de condensation.}

\textsc{\textbf{Théorème.}} --- \textit{Si un ensemble $E$ de points de l'espace $\left(E_{\omega}\right)$ est dans un domaine fini, l'ensemble de ceux de ses points qui ne sont pas des points limites de $E$ est dénombrable.}

\textsc{\textbf{Théorème.}} --- \textit{Soit $E$ un ensemble de points de l'espace $(E_{\omega})$ qui est fermé et contenu dans un domaine fini $D: 1^{\circ}$ il existe un ensemble dénombrable $G$ de sphéroïdes tels qu'on obtienne $E$ en enlevant de $D$ les points intérieurs à chacun de ces sphéroïdes; $2^{\circ} E$ peut être décomposé en un ensemble dénombrable de points et un ensemble parfait ou nul sans points communs avec le précédent; $3^{\circ}$ il existe au moins un ensemble $K$ de points de $(E_{\omega})$ dont l'ensemble dérivé coïncide avec $E$.}

\textsc{\textbf{Théorème.}} --- \textit{Pour qu'un ensemble $E$ de points de l'espace $(E_{\omega})$ soit fermé et contenu dans un domaine fini, il faut et il suffit que de toute famille $G$ d'ensembles I de points de $E$ telle que tout point de $E$ soit intérieur au sens étroit à l'un au moins des ensembles $I$, on puisse extraire un nombre fini de ces ensembles I formant une famille $H$ jouissant de la même propriété que $G$.}

\textsc{\textbf{Théorème.}} --- \textit{Tout ensemble parfait de points de $(E_{\omega})$ possède la puissance du continu.}

On peut encore ici résoudre une question analogue à celle qui a été posée par M. \textsc{Hadamard} pour les ensembles de fonctions continues ($\mathrm{n}^{\mathrm{o}}$ 39).

Soit $E$ un ensemble de points de l'espace $(E_{\omega})$; décomposons $E$ en ensembles partiels $k_{\varepsilon}$ tels que deux points quelconques de l'un d'eux aient un écart moindre que $\varepsilon$, et soit $\mathfrak{K}_\varepsilon$ l'ensemble des $k_{\varepsilon}$. 
\textit{Quels que soient $E$ et $\varepsilon$, on peut toujours opérer cette décomposition de façon que $\mathfrak{K}_\varepsilon$ soit dénombrable. Pour que, quel que soit $\varepsilon$, on puisse décomposer $E$ en un nombre fini d'ensembles $k_{\varepsilon}$, il faut et il suffit que $E$ soit contenu dans un domaine fini.}\\

\textbf{68.} 
\textsc{\textbf{Remarque.}} --- C'est ici le lieu d'observer qu'on aurait pu être amené à choisir une autre définition de la limite d'une suite de points de l'espace $(E_{\omega})$. Il semble au premier abord qu'il aurait été plus naturel, en même temps que plus adéquat aux applications, d'adopter la définition suivante: Une suite de points $x^{(1)}, x^{(2)}, \ldots, x^{(n)}, \ldots$ tend vers un point $x$ lorsque, étant donné un nombre $\varepsilon>0$, on peut trouver un entier $q$ tel que l'on ait:
$$
\left|x_{p}^{(n)}-x_{p}\right|<\varepsilon, \quad \text { pour } \quad n>q,
$$
quel que soit le rang $p$ des coordonnées considérées de $x^{(n)}$ et de $x$.

Il y aurait certainement lieu d'étudier une théorie des ensembles et de la continuité dans l'espace $\left(E_{\omega}\right)$ fondée sur cette définition qui peut présenter parfois des avantages (\textsc{xviii}). Cependant, elle se prête moins bien aux applications de nos théorèmes généraux. En effet, on voit que pour déduire cette définition d'une définition convenable de l'écart, on est amené à appeler écart de deux points $x, x^{\prime}$ la limite supérieure de $\left|x_{p}-x_{p}^{\prime}\right|$ quand $p$ prend toutes les valeurs entières possibles. Cette définition semble beaucoup plus simple que celle que nous avons adoptée; elle a pourtant l'inconvénient de ne pas s'appliquer à deux éléments quelconques. Plus exactement, elle pourrait donner une valeur infinie à l'écart de deux points dont les coordonnées sont finies (mais non bornées).

Un autre inconvénient de cette méthode est qu'on ne voit plus nettement quelle est la signification géométrique qu'il faut attacher à la notion d'ensemble compact. En effet, il est facile de former un exemple d'un ensemble de points de $(E_{\omega})$ qui est contenu dans un domaine fini et qui n'a pourtant aucun élément limite au sens de la deuxième définition. On pourrait peut-être espérer qu'il y a un élément limite lorsqu'on impose à l'ensemble d'être, non plus seulement infini, mais non dénombrable. Ou bien encore en restreignant la définition que nous avons donnée d'un domaine fini et en disant que le domaine sera fini si toutes les coordonnées sont en valeur absolue inférieures à un \textit{même} nombre fixe. Aucune de ces restrictions ne peut pourtant restituer sa validité au théorème en question. Il suffit en effet de considérer l'ensemble de tous les points distincts dont les coordonnées sont toujours égales à 0 ou 1. Cet ensemble a la puissance du continu (il n'est donc pas dénombrable) et toutes les coordonnées de ses points sont bornées dans leur ensemble; il n'a pourtant aucun point limite au sens de la deuxième définition. Il en a au contraire au sens de la première.

\subsection*{Les fonctions d'une suite infinie de variables indépendantes.}

\textbf{69.}
Conformément à nos définitions générales, nous dirons qu'une fonction d'une suite infinie de variables $x_{1}, x_{2}, \ldots, x_{n}, \ldots$:
$$
f\left(x_{1}, x_{2}, \ldots, x_{n}, \ldots\right)
$$
est continue, si $f\left(x_{1}^{(p)}, x_{2}^{(p)}, \ldots, x_{n}^{(p)}, \ldots\right)$ a pour limite $f\left(x_{1}, x_{2}, \ldots, x_{n}, \ldots\right)$ lorsque $x_{1}^{(p)}, x_{2}^{(p)}, \ldots, x_{n}^{(p)}, \ldots$ tendent simultanément, mais indépendamment, vers $x_{1}, x_{2}, \ldots$, $x_{n}, \ldots$ quand $p$ croît indéfiniment. Nous pouvons encore ici appliquer nos théorèmes généraux:

\textsc{\textbf{Théorème.}} --- \textit{Si une fonction d'un point de l'espace $(E_{\omega})$à une infinité dénombrable de dimensions est continue dans un ensemble limité et fermé de points de cet espace, cette fonction: $1^{0}$ est bornée; $2^{0}$ atteint en au moins un point de $E$ sa limite supérieure. Réciproquement, si cette propriété a lieu pour toutes les fonctions continues dans un ensemble $E$, cet ensemble est limité et fermé.}

\textsc{\textbf{Théorème.}} --- \textit{Toute fonction continue dans un ensemble extrémal de points de l'espace $(E_{\omega})$ est uniformément continue dans cet ensemble.}

\textsc{\textbf{Théorème.}} --- \textit{La condition nécessaire et suffisante pour qu'une série de fonctions continues en tout point d'un ensemble extrémal de points de l'espace $(E_{\omega})$ converge vers une fonction continue, est que la convergence de cette série soit quasi-uniforme.}

\textsc{\textbf{Théorème.}} --- \textit{Soit $\mathfrak{K}_\varepsilon$ une famille de fonctions continues dans un ensemble limité et fermé de points de l'espace $(E_{\omega})$. Pour que, de toute infinité de fonctions de $\mathfrak{K}_\varepsilon$, on puisse extraire une suite qui converge uniformément, il faut et il suffit que les fonctions de $\mathfrak{K}_\varepsilon$ soient également continues et bornées en tout point de l'ensemble.}

\section*{Chapitre VI.}
\subsection*{Fonctions holomorphes à l'intérieur d'une même aire.}

\textbf{70.}
Considérons dans le plan complexe des $z$, une aire quelconque $\mathfrak{A}$ à contour simple ou multiple. Nous allons étudier les ensembles dont les éléments sont des fonctions holomorphes en tout point \textit{intérieur} à $\mathfrak{A}$. Pour éviter des restrictions dans les énoncés que nous allons obtenir, nous ne nous préoccuperons pas de ce qui se passe sur le contour de $\mathfrak{A}$. Autrement dit, nous considérerons comme identiques deux fonctions holomorphes à l'intérieur de $\mathfrak{A}$ qui ont même valeur en tout point intérieur à $\mathfrak{A}$.

Pour appliquer nos théorèmes généraux, nous montrerons qu'on peut définir un écart. Supposons qu'on ait déterminé une suite d'aires limitées $\mathfrak{A}_{1},\, \mathfrak{A}_{2},\ldots \mathfrak{A}_{n}, \ldots$ chacune intérieure aux suivantes et à $\mathfrak{A}$, de façon que toute aire $\mathfrak{A}'$ intérieure à $\mathfrak{A}$ se trouve aussi intérieure aux aires de cette suite à partir d'un certain rang\footnote{Par exemple, si $\mathfrak{A}$ est limitée par un contour convexe simple, on prendrait pour $\mathfrak{A}_n$ l'homothétique de $\mathfrak{A}$ dans le rapport $\cfrac{n}{n+1}$ relativement à un point fixe pris indépendamment de $n$ à l'intérieur de $\mathfrak{A}$.}. Pour définir l'écart de deux fonctions $f$ et $g$ holomorphes à l'intérieur de $\mathfrak{A}$, nous appelons $u_{n}$ le maximum fini de $|f(z)-g(z)|$ quand $z$ varie dans $\mathfrak{A}_n$ ou sur son contour. La série
$$
\cfrac{u_{1}}{1+u_{1}}+\cfrac{1}{2!}\, \cfrac{u_{2}}{1+u_{2}}+\cdots+\cfrac{1}{n!}\, \cfrac{u_{n}}{1+u_{n}}+\cdots
$$
est certainement convergente; sa somme sera par définition l'écart $(f, g)$ de $f$ et de $g$ dans $\mathfrak{A}$. On voit que si $|f(z)-g(z)|$ a une limite supérieure finie $u$ quand $z$ varie de façon quelconque à l'intérieur de $\mathfrak{A}$ se l'écart sera inférieur à $\cfrac{e u}{1+u}$. Mais l'écart aura une valeur finie $<e$ même dans le cas contraire.

En se servant des remarques faites pour les points de l'espace $\left(E_{\omega}\right)$ au $\mathrm{n}^{\mathrm{o}}$ 62, on voit encore que la définition que nous venons de donner satisfait bien aux conditions imposées à celle de l'écart ($\mathrm{n}^{\mathrm{o}}$ 49).

Conformément à la théorie générale, nous dirons donc que, étant données deux fonctions holomorphes à l'intérieur de $\mathfrak{A}: f(z)$ et $f_{n}(z)$, la fonction $f(z)$ est la limite de $f_{n}(z)$ si leur écart tend vers zéro avec $\cfrac{1}{n}$.

Pour se rendre compte de la signification de cette définition, il suffit de remarquer que \textit{la condition nécessaire et suffisante pour que l'écart ($f, f_{n}$) tende vers zéro est que $f_{n}(z)$ tende uniformément vers $f(z)$ dans toute aire $\mathfrak{A}'$ intérieure à $\mathfrak{A}$.}

En effet, si cette condition est remplie, le maximum $u_{p}^{(n)}$ de $\left|f(z)-f_{n}(z)\right|$ dans $\mathfrak{A}$ tend vers zéro avec $\cfrac{1}{n}$, quel que soit l'entier fixe $p$. D'après un raisonnement employé plus haut ($\mathrm{n}^{\mathrm{o}}$ 63), cela suffit pour que l'écart

$$
\left(f, f_{n}\right)=\cfrac{u_{1}^{(n)}}{1+u_{1}^{(n)}}+\cdots+\cfrac{1}{p!}\, \cfrac{u_{p}^{(n)}}{1+u_{p}^{(n)}}+\cdots
$$
ait aussi pour limite zéro. Inversement, si l'écart tend vers zéro, il en est de même de $u_{p}^{(n)}$ quel que soit l'entier fixe $p$, d'après l'inégalité:
$$
\cfrac{u_{p}^{(n)}}{1+u_{p}^{(n)}}<p!\left(f, f_{n}\right)\,.
$$
Donc $f_{n}(z)$ tend uniformément vers $f(z)$ dans chaque aire $\mathfrak{A}_p$ et par suite dans toute aire $\mathfrak{A}'$ intérieure à $\mathfrak{A}$. Mais il n'est pas certain que la convergence de $f_{n}(z)$ vers $f(z)$ soit uniforme \textit{dans} $\mathfrak{A}$. On en verrait un exemple en prenant pour $\mathfrak{A}$ le cercle $|z| \leqslant 1$ et en posant $f_{n}(z) \equiv z^{n}, f(z) \equiv 0$. Il nous semble pourtant préférable d'adopter notre définition plutôt que celle d'après laquelle on considérerait seulement $f(z)$ comme limite de $f_{n}(z)$ quand $f_{n}(z)$ tend vers $f(z)$ uniformément \textit{dans toute l'aire} $\mathfrak{A}$. Car on serait amené à ne pas toujours considérer une fonction telle que $\cfrac{1}{1-z}$, comme limite de son développement de \textsc{Taylor} dans son cercle de convergence.\\

\textbf{71.} 
Ainsi donc, nous allons établir notre théorie des ensembles de fonctions holomorphes à l'intérieur de $\mathfrak{A}$ en considérant une fonction comme limite d'une autre, lorsque la valeur de la seconde tend vers la première uniformément à l'intérieur de toute aire intérieure à $\mathfrak{A}$.

Pour pouvoir appliquer nos théorèmes généraux de la \textsc{Première Partie}, nous démontrerons que \textit{la classe des fonctions holomorphes à l'intérieur d'une même aire $\mathfrak{A}$ est une classe $(E)$ normale.}

Nous savons qu'on peut la considérer comme une classe $(E)$. Montrons qu'elle admet une généralisation du théorème de \textsc{Cauchy}.

\textsc{\textbf{Théorème.}} --- \textit{Pour qu'une suite de fonctions:}
$$
f_{1}(z), \quad f_{2}(z), \ldots, f_{n}(z), \ldots
$$
\textit{holomorphes à l’intérieur d'une aire $\mathfrak{A}$ soit uniformément convergente dans toute aire $\mathfrak{A}'$ complètement intérieure à $\mathfrak{A}$, il faut et il suffit qu'à tout nombre $\varepsilon>0$, on puisse faire correspondre un entier $n$ tel que l'on ait, quel que soit $p$:}
$$
\left(f_{n}, f_{n+p}\right)<\varepsilon\,.
$$

Il n'y a aucune difficulté à montrer que la condition est nécessaire. Pour montrer qu'elle est suffisante, appelons $u_{q}^{(n, r)}$ le module maximum de $\left|f_{n}(z)-f_{r}(z)\right|$ dans $\mathfrak{A}_{q}$. Donnons-nous maintenant une aire $\mathfrak{A}'$ intérieure à $\mathfrak{A}$. On pourra prendre $q$ assez grand pour que $\mathfrak{A}'$ soit aussi complètement intérieure à $\mathfrak{A}_{q}$. Ayant ainsi fixé le nombre $q$, choisissons un nombre $\varepsilon>0$, inférieur à $\cfrac{\omega}{q!(1+\omega)}$.

Par hypothèse on pourra trouver un entier $n$ tel que l'on ait:
$$
\left(f_{n+p}, f_{n}\right)<\varepsilon,
$$
quel que soit $p$. Or,
$$
\cfrac{1}{q!}\, \cfrac{u_{q}^{(n, n+p)}}{1+u_{q}^{(n, n+p)}}<\left(f_{n}, f_{n+p}\right) .
$$
Donc
$$
\cfrac{1}{q!}\, \cfrac{u_{q}^{(n, n+p)}}{1+u_{q}^{(n, n+p)}}<\cfrac{1}{q!}\, \cfrac{\omega}{1+\omega}\,,
$$
ou
$$
u_{q}^{(n, n+p)}<\omega\,.
$$
Autrement dit, étant donné $\omega>0$, on peut trouver un entier $n$, tel que l'on ait en tout point de $\mathfrak{A}_{q}$:
$$
\left|f_{n}(z)-f_{n+p}(z)\right|<\omega,
$$
quel que soit l'entier $p$. Par conséquent la suite $f_{1}(z), f_{2}(z), \ldots$ est bien uniformément convergente dans $\mathfrak{A}'$.\\

\textbf{72.} 
Démontrons maintenant que les fonctions holomorphes à l'intérieur d'une même aire $\mathfrak{A}$ forment une classe séparable.

\textsc{\textbf{Théorème.}} --- \textit{On peut déterminer, une fois pour toutes, une suite $S$ de polynômes $P_{1}(z), P_{2}(z), \ldots, P_{n}(z), \ldots$ telle que toute fonction holomorphe à l'intérieur de $\mathfrak{A}$ soit limite d'au moins une suite extraite de $S$, et cela uniformément dans toute aire limitée $\mathfrak{A}'$ intérieure à $\mathfrak{A}$.}

Nous nous appuierons sur ce théorème bien connu que toute fonction $f(z)$ holomorphe à l'intérieur de $\mathfrak{A}$ est la somme d'une série de polynômes (avec convergence uniforme dans toute aire $\mathfrak{A}'$ intérieure à $\mathfrak{A}$). Alors, quel que soit $n$ on peut déterminer un polynôme $Q_{n}(z)$ tel que l'on ait \textit{dans toute l'aire} $\mathfrak{A}_n$, contour compris
$$
\left|f(z)-Q_{n}(z)\right|<\cfrac{1}{2 n}\,.
$$

Mais en remplaçant les parties réelles et imaginaires des coefficients de $Q_{n}(z)$ par leurs valeurs rationnelles approchées à moins de $\cfrac{1}{q}$ près, on pourra toujours former (en prenant $q$ assez grand) un polynôme $R_{n}(z)$ à coefficients rationnels tels que l'on ait dans l'aire limitée $\mathfrak{A}_n$ et sur son contour
$$
\left|Q_{n}(z)-R_{n}(z)\right|<\cfrac{1}{2 n}\,.
$$

Donc on aura $\left|f(z)-R_{n}(z)\right|<\cfrac{1}{n}$ dans $\mathfrak{A}_n$ et par suite $R_{n}(z)$ tend uniformément vers $f(z)$ dans toute aire limitée $\mathfrak{A}'$ intérieure à $\mathfrak{A}$. D'ailleurs, la suite $R_{1}(z), R_{2}(z), \ldots$ est extraite de l'ensemble $E$ des polynômes de la forme:
$$
\cfrac{a_{0}+a_{1} z+a_{2} z^{2}+\cdots+a_{k} z^{k}}{q}+i \cfrac{b_{0}+b_{1} z+b_{2} z^{2}+\cdots+b_{k} z^{k}}{q},
$$
où $q$ et $k$ sont deux entiers positifs; $a_{0}, a_{1}, \ldots a_{k}, b_{0}, b_{1}, \ldots b_{k}$ des entiers positifs négatifs ou nuls. Il suffit évidemment de démontrer que l'ensemble ${E}$ est dénombrable. D'ailleurs cet ensemble est la somme des ensembles $E_{q, k}$ de ceux de ces polynômes qui correspondent à des valeurs fixes de $q$ et de $k$. Il suffit donc de démontrer (\textsc{ii}, page 2) que chacun des ensembles $E_{q, k}$ est dénombrable. Or cela résulte de ce que les polynômes de $E_{q, k}$ pour lesquels $\left|a_{0}\right|+\left|a_{\mathrm{t}}\right|+\cdots+\left|a_{k}\right|+\left|b_{0}\right|+\cdots+\left|b_{k}\right|=r$ sont en nombre fini pour ch que valeur de $r$ et qu'on obtient $E_{q, k}$ prenant successivement $r=1,2, \ldots$.\\

\textbf{73.}
\textsc{\textbf{Théorème.}} --- \textit{La condition nécessaire et suffisante pour qu'un ensemble de  fonctions holomorphes à l'intérieur de $\mathfrak{A}$ soit un ensemble compact est que les fonctions de cet ensemble soient en module bornées dans leur ensemble dans toute aire limitée $\mathfrak{A}'$ intérieure à $\mathfrak{A}$.}

La condition est nécessaire d'après un raisonnement entièrement analogue à celui du $\mathrm{n^o}$ 18, en considérant l'aire limitée $\mathfrak{A}'$ comme un ensemble extrémal de points du plan.

Pour démontrer que la condition est suffisante, il suffit de démontrer que si l'on considère une infinité $I$ de fonctions holomorphes à l'intérieur de $\mathfrak{A}$ et bornées dans toute aire $\mathfrak{A}'$ intérieure à $\mathfrak{A}$, on peut extraire de $I$ une suite qui converge uniformément dans chacune de ces aires $\mathfrak{A}'$ \footnote{Ce théorème a été démontré par M. \textsc{Arzelà} (\textsc{x}, page 6) lorsqu'on ajoute à notre hypothèse les conditions: $1^{\circ}$ que les fonctions de $I$ sont bornées, non seulement dans les $\mathfrak{A}'$, mais dans tout $\mathfrak{A}$ (ce qui est moins général); $2^{\circ}$ que les dérivées de ces fonctions sont aussi bornées dans $\mathfrak{A}$, ce qui est inutile. M. \textsc{Montel} a énoncé sans démonstration (\textsc{xxv}) que si des fonctions sont régulières dans $\mathfrak{A}$, \textit{continues sur le contour} et bornées dans leur ensemble dans $\mathfrak{A}$,  on peut en extraire une suite qui converge uniformément dans $\mathfrak{A}$.}.

Or on peut extraire de $\mathfrak{A}$ une suite $S$ de points \textit{intérieurs} à $\mathfrak{A}$: $\alpha_{1}, \alpha_{2}, \ldots, \alpha_{n}, \ldots$, telle que tout point intérieur à $\mathfrak{A}$ appartienne à la suite $S$ ou à son ensemble dérivé ($\mathrm{n^o}$ 45). Soit $r_{n}$ la limite inférieure de la distance de $\alpha_{n}$ aux points non intérieurs à $\mathfrak{A}$. Appelons $\boldsymbol{\Gamma}_{n}$ un cercle de centre $\alpha_{n}$ et de rayon $\rho_{n}=r_{n}\left(\cfrac{n}{n+1}\right)$. Tout point intérieur à $\mathfrak{A}$ est intérieur à l'un au moins des cercles $\boldsymbol{\Gamma}_{n}$; et inversement, tout point de $\boldsymbol{\Gamma}_{n}$, ou de son contour, est \textit{intérieur} à $\mathfrak{A}$. Dans chacun des cercles $\boldsymbol{\Gamma}_{n}$ une quelconque des fonctions $f(z)$ de $I$ est développable en une série de \textsc{Taylor} qui converge uniformément dans $\boldsymbol{\Gamma}_{n}$, contour compris:
$$
f(z)=a_{0, n}+a_{1, n}\left(z-\alpha_{n}\right)+\cdots+a_{p, n}\left(z-\alpha_{n}\right)^{p}+\cdots
$$

Alors, à chaque fonction $f(z)$, on peut faire correspondre un point $A$ de l'espace $(E_{\omega})$ à une infinité dénombrable de dimensions, à savoir le point ayant pour coordonnées l'ensemble dénombrable de nombres:
\begin{equation*}
a_{0,1}, a_{1,1}, a_{2,1}, \ldots ; a_{0,2}, a_{1,2}, a_{2,2}, \ldots ; a_{0, n}, a_{1, n}, \ldots . \footnote{Ces nombres ne sont pas rangés de façon à suivre l'ordre d'un seul indice comme au Chapitre V. Mais il suffit de savoir qu'on pourrait le faire.} \tag{1}
\end{equation*}

Par suite, à l'ensemble $I$ de fonctions $f(z)$ correspond un ensemble $G$ de points $A$ de $(E_{\omega})$. Cet ensemble est limité, car on a, quel que soit le point $A$,
$$
\left|a_{p, n}\right|<\cfrac{M_{n}}{\left(\rho_{n}^{\prime}\right)^{p}}\,,
$$
en appelant $M_{n}$ un nombre supérieur au module de toute fonction $f(z)$ de $I$ en tout point d'un cercle $C_{n}^{\prime}$ de centre $\alpha_{n}$ et de rayon $\rho_{n}^{\prime}>\rho_{n}$ et $<r_{n}$. Dés lors, l'ensemble $G$ est compact ($\mathrm{n^o}$ 66) et on peut prendre une suite de ses points $A_{1}, A_{2}, \ldots$ ayant une limite $B$. En appelant 
$$
a_{0,1}^{(q)}, \, a_{1,1}^{(q)}, \ldots, a_{p, n}^{(q)}, \ldots
$$
les coordonnées de $A_{q}$ et
$$
b_{0,1}, \, b_{1,1}, \ldots, b_{p, n}, \ldots
$$
celles de $B$, on aura:
$$
b_{p, n}=\lim _{q=\infty} a_{p, n}^{(q)},
$$
quels que soient $p, n$. Il en résulte en particulier que l'on a:
$$
\left|b_{p, n}\right| \leqslant \cfrac{M_{n}}{\left(\rho_{n}^{\prime}\right)^{p}} ;
$$
par suite, pour chaque valeur de $n$ la série:
$$
b_{0, n}+b_{1, n}\left(z-\alpha_{n}\right)+\cdots+b_{p, n}\left(z-\alpha_{n}\right)^{p}+\cdots
$$
converge vers une fonction $\varphi_{n}(z)$ holomorphe à l'intérieur de $C_{n}^{\prime}$. Soient d'autre part $f_{1}(z), f_{2}(z), \ldots$ les fonctions de $I$ qui correspondent à $A_{1}, A_{2}, \ldots$ Je vais démontrer que cette suite de fonctions a une limite. En effet, on a dans tout cercle $\boldsymbol{\Gamma}_{n}$:
$$
\begin{gathered}
\left|f_{q}(z)-\varphi_{n}(z)\right|<\left|a_{0, n}^{(q)}-b_{0, n}\right|+\cdots+\left|a_{p, n}^{(q)}-b_{p, n}\right|\left(\rho_{n}\right)^{p} \\
+2 M_{n}\left[\left(\cfrac{\rho_{n}}{\rho_{n}^{\prime}}\right)^{p}+\left(\cfrac{\rho_{n}}{\rho_{n}^{\prime}}\right)^{p+1}+\cdots\right] .
\end{gathered}
$$
En prenant $p$ assez grand, le dernier terme sera $<\cfrac{\varepsilon}{2}$; $p$ étant ainsi choisi et fixé, la somme des $p+1$ premiers termes tend vers zéro avec $\cfrac{1}{q}$, on peut donc trouver $h$ tel que cette somme reste inférieure à $\cfrac{\varepsilon}{2}$ pour $q>h$. En résumé, $f_{q}(z)$ tend uniformément vers $\varphi_{n}(z)$ dans $\boldsymbol{\Gamma}_{n}$ contour compris.

Comme tout point intérieur à $\mathfrak{A}$ est intérieur à au moins un cercle $\boldsymbol{\Gamma}_{n}$, on voit d'abord que l'on a bien extrait de $I$ une suite $f_{1}, f_{2}, \ldots$ convergente en tout point intérieur à $\mathfrak{A}$. De plus, la limite $f(z)$ est une fonction holomorphe en tout point intérieur à $\mathfrak{A}$ puisqu'elle coïncide avec $\varphi_{n}(z)$ dans $\boldsymbol{\Gamma}_{n}$ quel que soit $n$. Enfin, la convergence est uniforme dans toute aire limitée $\mathfrak{A}'$ intérieure à $\mathfrak{A}$. 
En effet, les points de cette aire sel $\mathfrak{A}'$ (contour compris) forment un ensemble limité et fermé dont chaque point est intérieur à l'un au moins des cercles $\boldsymbol{\Gamma}_{n}$; on peut donc extraire un nombre fini de ces cercles jouissant de la même propriété (voir $\mathrm{n^o}$ 36). La fonction $f_{q}(z)$ convergeant uniformément dans un nombre \textit{fini} de cercles $\boldsymbol{\Gamma}_{n}$ convergera aussi uniformément dans l'aire $\mathfrak{A}'$ qu'ils recouvrent.

Il serait d'ailleurs inexact d'affirmer qu'on peut choisir la suite $f_{1}(z), f_{2}(z), \ldots$ de façon qu'elle converge uniformément \textit{dans toute l'aire} $\mathfrak{A}$ (voir la note précédente). Cela serait inexact même si l'on supposait que les fonctions de $I$ sont à la fois holomorphes et bornées dans leur ensemble dans $\mathfrak{A}$ \textit{contour compris}. Il suffit pour s'en rendre compte de prendre encore pour $\mathfrak{A}$ le cercle $|z| \leqslant 1$ et pour $I$ les fonctions $z^{n}$.\\

\textbf{74.} 
\textit{\textbf{Application des théorèmes généraux.}} --- Nous savons que les fonctions holomorphes à l'intérieur d'une même aire $\mathfrak{A}$ forment une classe $(E)$ normale. Nous pouvons donc leur appliquer les résultats généraux de la \textsc{Première Partie} en ayant soin de conserver à la définition de la limite d'une suite de fonctions holomorphes dans $\mathfrak{A}$ le sens que nous avons précisé plus haut ($\mathrm{n}^{\mathrm{o}}$ 71).

\textsc{\textbf{Théorème.}} --- \textit{Soit $E$ un ensemble quelconque de fonctions holomorphes à l'intérieur d'une même aire $\mathfrak{A}$ à contour simple ou multiple: $1^{\circ}$ l'ensemble des éléments limites de $E$ est fermé; $2^{\circ}$ ou bien $E$ est dénombrable, ou bien $E$ donne lieu à au moins un élément de condensation $(\mathrm{n}^{\mathrm{o}}\;8)$; $3^{\circ}$ on peut extraire de $E$ une suite dénombrable $S$ de fonctions telles que toute fonction de $E$ appartienne à $S$ ou soit limite d'au moins une suite extraite de $S$.}

\textsc{\textbf{Théorème.}} --- \textit{Si les fonctions de l'ensemble $E$ précédent sont en module bornées dans leur ensemble dans toute aire limitée $\mathfrak{A}'$ intérieure à $\mathfrak{A}$, l'ensemble des fonctions de $E$ qui ne sont pas limites de fonctions de $E$ est dénombrable.}

\textsc{\textbf{Théorème.}} --- \textit{Soit $F$ un ensemble fermé de fonctions holomorphes et bornées en module dans leur ensemble dans toute aire limitée $\mathfrak{A}'$ intérieure à $\mathfrak{A}$: $1^\circ$ il existe au moins un ensemble $H$ de fonctions holomorphes à l'intérieur de $\mathfrak{A}$ dont l'ensemble des éléments limites coïncide avec $F$; $2^{\circ}$ on peut décomposer $F$ en un ensemble dénombrable et un ensemble parfait ou nul.}

\textsc{\textbf{Théorème.}} --- \textit{Tout ensemble parfait de fonctions holomorphes à l'intérieur de $\mathfrak{A}$ possède la puissance du continu.}

On peut aussi répondre à une question analogue à celle de M. \textsc{Hadamard} ($\mathrm{n}^{\mathrm{os}}$ 39, 58) et donner une généralisation du théorème de M. \textsc{Borel} ($\mathrm{n}^{\mathrm{o}}$ 42) pour des ensembles de fonctions holomorphes.\\

\textbf{75.} 
De même, considérons des opérations fonctionnelles ($\mathrm{n}^{\mathrm{o}}$ 4) dont la variable soit une fonction holomorphe (voir \textsc{xvi, xxvi}).

\textsc{\textbf{Théorème.}} --- \textit{Soit $F$ l'ensemble précédemment considéré de fonctions holomorphes. Toute opération réelle continue portant sur des fonctions holomorphes de $F: 1^{\circ}$ est uniformément continue dans $F$; $2^{\circ}$ est bornée et atteint sa limite supérieure pour au moins une fonction de $F$.}

\textit{Réciproquement, si toute opération réelle continue dans un ensemble $E$ de fonctions holomorphes à l'intérieur d'une même aire $\mathfrak{A}$ atteint sa limite supérieure pour au moins une fonction de $E$, l'ensemble $E$ est fermé et compact.}

\textsc{\textbf{Théorème.}} --- \textit{Considérons une série d'opérations continues dans un ensemble fermé $F$ de fonctions holomorphes et bornées dans toute aire limitée $\mathfrak{A}'$ intérieure à $\mathfrak{A}$ Pour que la somme de cette série soit une opération continue dans $F$, il faut et il suffit que la convergence soit quasi-uniforme.}

\textsc{\textbf{Théorème.}} --- \textit{Soit $\mathfrak{F}$ une famille d'opérations continues dans le même ensemble $F$ de fonctions holomorphes. Pour que de toute infinité d'opérations de $\mathfrak{F}$, on puisse extraire une suite qui converge uniformément, il faut et il suffit que les opérations de $\mathfrak{F}$ soient également continues et bornées en tout élément de $F$.}

\section*{Chapitre VII.}
\subsection*{Ensembles de courbes continues et fonctions de lignes.}

\textbf{76.}
\textit{\textbf{Définition de l'arc de courbe.}} --- Soient $f, g, h$, trois fonctions de $t$ continues dans un même intervalle $I: a \leqslant t \leqslant b$ et qui ne sont à la fois constantes dans aucun intervalle compris dans $I$ ou qui sont à la fois constantes dans \textit{tout} l'intervalle $I$. Les formules:
\begin{equation*}
x=f(t), \quad y=g(t), \quad z=h(t) \qquad\qquad (a\leqslant t \leqslant b) \tag{1}
\end{equation*}
définissent dans l'espace à trois dimensions un ensemble $E$ de points $(x, y, z)$. Dans le second cas cet ensemble $E$ ne comprend qu'un seul point; dans le premier, il est non dénombrable et alors aussi parfait, limité et bien enchaîné. Si l'on tient compte de l'ordre dans lequel se présentent les points de $E$ quand on fait croître $t$, on obtient une suite ordonnée (\textsc{iii}, p. 27) qu'on appelle \textit{arc de courbe}. Il y a donc entre l'ensemble $E$ et l'arc de courbe $\gamma$, auquel il donne naissance, la même différence qu'il $y$ a entre une combinaison et un arrangement. Autrement dit, considérons un système de trois fonctions $F(u), G(u), H(u)$ satisfaisant aux mêmes conditions que $f, g, h$; les formules:
\begin{equation*}
x=F(u), \quad y=G(u), \quad z=H(u) \qquad\qquad A \leqslant u \leqslant B \tag{2}
\end{equation*}
définissent un arc de courbe $\boldsymbol{\Gamma}$ qu'on ne devra envisager comme coïncidant avec $\gamma$ que si non seulement $\gamma$ et $\boldsymbol{\Gamma}$ sont formés par le même ensemble de points, mais si encore on rencontre ces points dans le même ordre quand on fait croître, soit $t$, soit $u$, dans (1) ou (2). Cette dernière condition est indépendante de la première; il suffit pour le voir de choisir, comme cela est facile, les formules (1) et (2) de façon à représenter deux arcs de courbes en forme de huit: \textit{QRSQTPQ} et \textit{QSRQTPQ} formés des mêmes points non parcourus dans le même ordre.

Remarquons que, comme dans l'exemple précédent, un même point géométrique peut être rencontré deux fois sur un arc de courbe, c'est-à-dire peut correspondre à deux valeurs de $t$ différentes. Nous considérerons cependant ces deux valeurs de $t$ comme correspondant à deux points de $\gamma$ distincts (points multiples). Cette convention faite, nous pourrons dire que, pour que deux courbes $\gamma$ et $\boldsymbol{\Gamma}$ coïncident, il faut et il suffit qu'on puisse établir entre leur points une correspondance univoque et réciproque telle que deux points correspondants coïncident et que leur ordre soit conservé\footnote{Remarquons que cette définition satisfait bien à ces conditions fondamentales que: $1^{\circ}$ si $\gamma$ est identique à $\boldsymbol{\Gamma}$, $\boldsymbol{\Gamma}$ est identique à $\gamma$; $2^{\circ}$ si deux courbes sont identiques à une même troisième, elles coïncident.}.\\

\textbf{77.} 
En général, on se contente de dire que deux courbes (1) et (2) coïncident, s'il est possible de trouver une fonction $u=\varphi(t)$ continue et constamment croissante, allant de $A$ à $B$ quand $t$ croît de $a$ à $b$, et telle que l'on ait
\begin{equation*}
f(t) \equiv F[\varphi(t)], \quad g(t) \equiv G[\psi(t)], \quad h(t)=H[\varphi(t)] \qquad\qquad(a \leqslant t \leqslant b) . \tag{3}
\end{equation*}
Cette définition a l'inconvénient de ne pas avoir un rapport direct avec la notion intuitive que nous avons de l'identité de deux courbes, notion qui me semble clairement exprimée dans la définition que j'ai donnée plus haut. Remarquons d'ailleurs que, si la condition (3) est remplie, les courbes coïncideront bien au premier sens que j'ai indiqué. Mais la réciproque est moins évidente. Pour la démontrer, observons que si l'on peut établir entre (1) et (2) cette correspondance dans laquelle l'ordre est conservé, on pourra évidemment obtenir des identités telles que (3) dans lesquelles $\varphi(t)$ est une fonction bien déterminée pour chaque valeur de $t$ et qui va sans jamais décroître de $A$ à $B$ quand $t$ croit de $a$ à $b$. Il reste à montrer que $\psi(t)$ est une fonction continue croissante. Or s'il en était autrement: ou bien $\varphi(t)$ serait constante dans un certain intervalle, et alors $f(t), g(t), h(t)$ seraient à la fois constantes dans cet intervalle, ou bien $\varphi(t)$ passerait brusquement de valeurs $<\varphi\left(t_{0}\right)-k$, à des valeurs supérieures à $\varphi\left(t_{0}\right)+k$ quand $t$ passe par $t_{0}$ et alors l'ordre ne serait pas conservé.

Ainsi, la définition géométrique que nous avons donnée coïncide complètement avec la définition ordinaire. Celle-ci permet en particulier de supposer toujours que l'intervalle de variation du paramètre est l'intervalle $(0,1)$; il suffit de faire la transformation $u=\cfrac{t-a}{b-a}$. Nous admettrons toujours par la suite qu'on a effectué celle-ci.\\

\textbf{78.} 
\textit{\textbf{Définition de l'écart.}} --- Maintenant que nous savons discerner les courbes distinctes, nous pouvons considérer l'ensemble de toutes ces courbes comme formant une classe d'éléments à laquelle nous essayerons d'appliquer nos théorèmes généraux. Dans ce but, nous démontrerons qu'on peut donner pour cette classe une définition de l'écart.

Considérons en effet deux représentations quelconques:
\begin{equation*}
    x=f(t),  y=g(t),  z=h(t) \qquad\qquad\qquad\; (0 \leqslant t \leqslant 1), \tag{4}
\end{equation*}
\begin{equation*}
x=F(u),  y=G(u),  z=H(u) \qquad \qquad \quad (0\leqslant u \leqslant 1),\tag{5}
\end{equation*}
de deux courbes $\gamma$ et $\boldsymbol{\Gamma}$ et formons l'expression
$$
\delta(t)=\sqrt{[f(t)-F(t)]^{2}+[g(t)-G(t)]^{2}+[h(t)-H(t)]^{2}} \quad\quad(0 \leqslant t \leqslant 1) ;
$$
c'est une fonction continue de $t$ qui a un maximum $d \geqslant 0$. Nous appellerons \textit{écart des deux courbes} la limite inférieure $e \geqslant 0$ de l'ensemble des valeurs de $d$ obtenues en prenant pour (4) et (5) toutes les représentations possibles de $\gamma$ et de $\boldsymbol{\Gamma}$. On peut simplifier le calcul de l'écart en remarquant qu'il suffit de prendre pour $e$ la limite inférieure des valeurs de $d$ obtenues en prenant pour $\gamma$ une représentation quelconque déterminée (4) et en faisant varier seulement la représentation de $\boldsymbol{\Gamma}$. En effet, une représentation simultanée quelconque de $\gamma$ et de $\boldsymbol{\Gamma}$ pourra s'écrire, d'après ce qui précède,
$$
\begin{array}{llll}
x=f[\varphi(t)], & y=g[\varphi(t)], & z=h[\varphi(t)] \qquad\qquad & (0 \leqslant t \leqslant 1), \\
x=F[\psi(u)], & y=G[\psi(u)], & z=H[\psi(u)] \qquad\qquad & (0 \leqslant u \leqslant 1),
\end{array}
$$
où $\varphi(t)$ et $\psi(u)$ sont deux fonctions continues croissantes. Alors, pour une telle représentation la valeur de $\delta$ sera
$$
\delta_{1}(t)=\sqrt{\{f[\varphi(t)]-F[\psi(t)]\}^{2}+\{g[\varphi(t)]-G[\psi(t)]\}^{2}+\{h[\varphi(t)]-H[\psi(t)]\}^{2}}
$$
et si $\varphi_{1}(u)$ est la fonction inverse de $\varphi(t)$, on aura, en posant $\theta(u)=\psi\left[\varphi_{1}(u)\right]$,
$$
\delta_{1}\left[\varphi_{1}(u)\right]=\sqrt{\left\{f(u)-F[\theta(u)]\}^{2}+\{g(u)-G[\theta(u)]\right\}^{2}+\{h(u)-H[\theta(u)]\}^{2}} .
$$

Mais le maximum de $\delta_{1}(t)$ est évidemment le même que celui de $\delta_{1}\left[\varphi_{1}(u)\right]$ qui passe par les mêmes valeurs. Or ce dernier est bien obtenu en conservant la même représentation de $\gamma$ et en faisant varier celle de ${\boldsymbol{\Gamma}}$.\\

\textbf{79.} 
Ceci étant, il est facile de démontrer que \textit{la définition que nous venons de donner satisfait bien aux conditions générales a), b) de l'écart }($\mathrm{n^o}$ 49). En effet, il est d'abord évident que si $\gamma$ et $\boldsymbol{\Gamma}$ coïncident, l'une des valeurs de $d$ est nulle et par suite $(\gamma, \boldsymbol{\Gamma})=0$. Réciproquement, si cette condition est vérifiée: ou bien l'une des valeurs de $d$ est nulle, et alors $\gamma$ et $\boldsymbol{\Gamma}$ coïncident sûrement; ou bien, quelque soit $n$, on peut déterminer une fonction $\varphi_{n}(t)$ continue et allant en croissant de 0 à 1, telle que l'on ait, pour toute valeur de $t$ entre $0$ et $1$,
\begin{equation*}
\sqrt{\left\{f(t)-F\left[\varphi_{n}(t)\right]\right\}^{2}+\left\{g(t)-G\left[\varphi_{n}(t)\right]\right\}^{2}+\left\{h(t)-H\left[\varphi_{n}(t)\right]\right\}^{2}}<\cfrac{1}{n} . \tag{6}
\end{equation*}
On aura donc
$$
f(t)=\lim _{n=\infty} F\left[\varphi_{n}(t)\right], \, g(t)=\lim _{n=\infty} G\left[\varphi_{n}(t)\right], \, h(t)=\lim _{n=\infty} H\left[\varphi_{n}(t)\right] ; \, (0 \leqslant t \leqslant 1),
$$
avec convergence uniforme. Pour démontrer le théorème, il suffit de prouver que l'on peut extraire de la suite $\varphi_{1}(t), \varphi_{2}(t), \ldots$ une suite qui converge uniformément vers une fonction $\varphi(t)$ (nécessairement continue et croissante de 0 à 1). 
Pour cela, nous montrerons que les fonctions $\varphi_{n}(t)$ sont également continues et bornées ($\mathrm{n^o}$ 57). 
Elles sont évidemment bornées: $0 \leqslant \varphi_{n}(t) \leqslant 1$. Si elles n'étaient pas également continues, on pourrait déterminer un nombre $\varepsilon>0$ tel que, quel que soit $n$, il y ait une fonction $\varphi_{p_{n}}$ et deux nombres $t_{n}, t_{n}^{\prime}$ de l'intervalle $(0,1)$ vérifiant les inégalités
\begin{equation*}
\left|\varphi_{p_{n}}\left(t_{n}\right)-\varphi_{p_{n}}\left(t_{n}^{\prime}\right)\right|>\varepsilon, \quad 0<\left|t_{n}-t_{n}^{\prime}\right|<\cfrac{1}{n} . \tag{7}
\end{equation*}
Et comme les nombres $t_{n}, \varphi_{p_{n}}\left(t_{n}\right), \varphi_{p_{n}}\left(t_{n}^{\prime}\right)$ sont bornés dans leur ensemble, on peut supposer les avoir choisis de façon qu'ils convergent (quand $n$ croît indéfiniment) vers des limites respectives que nous appellerons $\tau_{0}, u_{0}, u_{0}^{\prime}$. Alors les inégalités (7) montrent que $t_{n}^{\prime}$ tend aussi vers $\tau_{0}$ et que l'on a $\left|u_{0}-u_{0}^{\prime}\right| \geqslant \varepsilon$. Ceci étant, soit $\lambda$ un nombre quelconque compris entre $u_{0}$ et $u_{0^{\prime}}$; pour $n$ assez grand $\varphi_{p_{n}}\left(t_{n}\right)$ et $\varphi_{p_{n}}\left(t_{n}^{\prime}\right)$, qui tendent vers $u_{0}$ et $u_{0}^{\prime}$, comprendront entre eux le nombre $\lambda$. La fonction continue $\varphi_{p_{n}}(t)$ prendra donc au moins une fois la valeur $\lambda$ pour une valeur $\tau_{n}$ de $t$ comprise entre $t_{n}$ et $t_{n}^{\prime}$. On aura donc, d'après (6),
$$
\left|f\left(\tau_{n}\right)-F(\lambda)\right|<\cfrac{1}{p_{n}}, \quad\left|g\left(\tau_{n}\right)-G(\lambda)\right|<\cfrac{1}{p_{n}}, \quad\left|h\left(\tau_{n}\right)-H(\lambda)\right|<\cfrac{1}{p_{n}} \,.
$$
Comme $\tau_{n}$ tend évidemment vers $\tau_{0}$, il en résulte que l'on a

$$
f\left(\tau_{0}\right)=F(\lambda), \quad g\left(\tau_{0}\right)=G(\lambda), \quad h\left(\tau_{0}\right)=H(\lambda),
$$
quelle que soit la valeur de $\lambda$ comprise entre $u_{0}$ et $u_{0}^{\prime}$. Nous arrivons ainsi à la contradiction annoncée puisque $F(u), G(u), H(u)$ ne sont à la fois constants dans aucun intervalle. Il faudrait faire exception pour le cas où $\boldsymbol{\Gamma}$ se réduirait à un point, mais alors la réciproque est évidente.\\

\textbf{80.} 
Pour démontrer que la condition b) du $\mathrm{n}^{\circ}$ 49 est satisfaite, considérons trois courbes $\gamma, \boldsymbol{\Gamma}$ et $C$, ayant pour représentations (4), (5) et
$$
x=a(v), \quad y=b(v), \quad z=c(v) \qquad\qquad(0 \leqslant v \leqslant 1).
$$
Pour obtenir leurs écarts respectifs, il suffit de prendre les maxima des quantités
$$
\begin{aligned}
\delta(t) & =\sqrt{\{f[\varphi(t)]-F[\psi(t)]\}^{2}+\{g[\varphi(t)]-G[\psi(t)]\}^{2}+\{h[\varphi(t)]-H(\psi(t)]\}^{2}}\,, \\
\delta_{1}(t) & =\sqrt{\{a(t)-f[\psi(t)]\}^{2}+\{b(t)-g[\varphi(t)]\}^{2}+\{c(t)-h[\varphi(t)]\}^{2}}\,, \\
\delta_{2}(t) & =\sqrt{\{a(t)-F[\psi(t)]\}^{2}+\{b(t)-G[\psi(t)]\}^{2}+\{c(t)-H(\psi(t)]\}^{2}}\,,
\end{aligned}
$$
quand $t$ croît de $0$ à $1$, puis de faire varier la forme de $\varphi(t)$ et $\psi(t)$, fonctions continues croissantes de $t$. On a évidemment
$$
\delta(t) \leqslant \delta_{1}(t)+\delta_{2}(t) ;
$$
on en déduit facilement pour les maxima correspondants $d, d_{1}, d_{2}$ :
$$
d \leqslant d_{1}+d_{2}
$$
et en faisant varier indépendamment $\varphi$ et $\psi$ :
$$
(\gamma, \boldsymbol{\Gamma}) \leqslant(C, \gamma)+(C, \boldsymbol{\Gamma}) .
$$

\textbf{81.}
\textit{\textbf{Limite d'une suite de courbes.}} --- La définition de l'écart a pour conséquence ($\mathrm{n}^{\text {os}}$ 49, 27) une définition de la limite: \textit{La courbe $\gamma_{n}$ tend vers $\gamma$ lorsque l'écart ($\gamma_{n}, \gamma$) tend vers zéro avec $\cfrac{1}{n}$}. Cette définition peut s'exprimer analytiquement de la façon suivante:

La condition nécessaire et suffisante pour qu'une courbe $\gamma_{n}$ ait pour limite une courbe $\gamma$, lorsque $n$ croit indéfiniment, est qu'il existe une représentation de $\gamma_{n}$:
\begin{equation*}
x=f_{n}(t), \quad y=g_{n}(t), \quad z=h_{n}(t) \qquad\qquad(0 \leqslant t \leqslant 1), \tag{8}
\end{equation*}
et une représentation de $\gamma$:
\begin{equation*}
x=f(t), \quad y=g(t), \quad z=h(t) \qquad\qquad (0 \leqslant t \leqslant 1) \tag{4}
\end{equation*}
telles que $f_{n}, g_{n}, h_{n}$ convergent uniformément vers $f, g, h$.

En effet, si cette condition est vérifiée, il est évident que ($\gamma_{n}, \gamma$) tend vers zéro. Réciproquement, choisissons une représentation déterminée (4) de $\gamma$; on pourra, quel que soit $n$, choisir une représentation (8) de $\gamma_{n}$, telle que l'on ait
$$
\sqrt{\left[f(t)-f_{n}(t)\right]^{2}+\left[g(t)-g_{n}(t)\right]^{2}+\left[h(t)-h_{n}(t)\right]^{2}}<\left(\gamma_{n}, \gamma\right)+\cfrac{1}{n} \,.
$$

Alors, si $\left(\gamma_{n}, \gamma\right)$ tend vers zéro, on voit que $f_{n}, g_{n}, h_{n}$ convergent uniformément vers $f, g, h$.

Nous sommes ainsi ramené à la définition ordinaire de la limite d'une courbe. Il en résulte en particulier que si $\gamma_{n}$ tend vers $\gamma$, elle se trouve toute entière contenue, pour $n$ assez grand, dans le volume engendré par une sphère de rayon $\varepsilon$ dont le centre parcourt $\gamma$.\\

\textbf{82.} 
La définition que nous avons donnée de l'écart semble assez arbitraire; tâchons de montrer pourquoi elle est préférable à d'autres qui pourraient paraître plus naturelles.

On a eu depuis longtemps l'idée de définir un nombre déterminé par deux courbes $C_{1}$ et $C_{2}$ de telle façon que ce nombre soit nul quand les deux courbes coïncident et soit très petit quand les deux courbes sont infiniment voisines.

M. \textsc{Arzelà} considère ainsi ce qu'il appelle \textit{la plus courte distance des deux courbes} (\textsc{v}, page 343), savoir la limite inférieure $\lambda$ de la distance de deux points, l'un quelconque sur $C_{1}$, l'autre quelconque sur $C_{2}$. Un tel nombre satisfait bien aux deux conditions précédentes. Mais il ne satisfait pas aux conditions réciproques: il n'est pas nécessaire pour que $\lambda$ soit nul que les deux courbes coïncident, il suffit qu'elles se coupent. Les deux courbes peuvent être très différentes de formes et le nombre $\lambda$ aussi petit que l'on veut et même nul. Aussi, la considération du nombre $\lambda$ ne suffit-elle pas à M. \textsc{Arzelà} pour définir la limite d'une courbe.

Avant M. \textsc{Arzelà}, \textsc{Weierstrass} avait introduit une quantité qu'il appelait \textit{voisinage de deux courbes}. La définition qu'il en donnait échappe à l'objection précédente, en ce sens que le voisinage est toujours petit lorsque les deux courbes sont voisines et dans ce cas seulement. Mais il n'est défini que pour des courbes voisines. \textsc{Weierstrass} appelait voisinage de deux courbes voisines tout nombre $\geqslant 0$ inférieur au maximum de la distance de deux points correspondants à une même abscisse ou à des abscisses très voisines. Sa définition, parfaitement suffisante pour le but qu'il se proposait\footnote{Celui d'apporter plus de rigueur dans le Calcul des variations.}, manquait de précision à notre point de vue. De plus, il ne pouvait songer à l'utiliser dans la théorie des ensembles qui était encore à ses débuts. Au contraire, M. \textsc{Arzelà} semble avoir été le premier qui ait aperçu l'importance de la définition d'un nombre bien déterminé tel que sa \textit{plus courte distance} et défini pour deux courbes quelconques.

Au lieu des définitions précédentes dont nous avons reconnu l'insuffisance, on aurait pu songer aussi à introduire un nombre $\mu_{1, 2}$ qui serait la limite supérieure de la distance minimum d'un point de $C_{1}$ à tous les points de $C_{2}$; ou bien encore, on aurait pu introduire le nombre $\rho_{1,2}$ représentant la limite inférieure du maximum de la distance d'un point de $C_{1}$ à tous les points de $C_{2}$. Ces nombres satisfont en partie aux conditions que nous exigeons de l'écart, mais pas à toutes.

D'abord, ils sont bien définis, quand même $C_{1}$ et $C_{2}$ ne seraient pas très voisins. De plus, si $C_{1}$ coïncide avec $C_{2}$, on a $\mu_{1,2}=0$. Mais il peut arriver que $\mu_{1,2}$ soit nul sans que $C_{1}$ coïncide avec $C_{2}$; il suffit, en effet, que l'ensemble de leurs points soit le même. Inversement, il peut arriver que $C_{1}$ coïncide avec $C_{2}$ sans que $\rho_{1,2}$ soit nul, car dans ce dernier cas $C_{2}$ serait réduit à un point. Ces nombres $\mu_{1,2}, \rho_{1,2}$, ne sauraient donc définir un écart des deux courbes. Mais comme ils sont d'un calcul plus facile que l'écart $e$, ils peuvent être parfois utiles pour donner une idée de la valeur de $e$. On voit, en effet, bien facilement, que l'on a toujours $\lambda \leqslant \mu_{1,2} \leqslant e$ et $\lambda \leqslant \mu_{2,1} \leqslant e$.

Ces inégalités sont utiles dans certaines questions (voir par exemple $\mathrm{n^o}$~85).\\

\textbf{83.} 
\textit{\textbf{Limite d'une courbe.}} --- Le théorème que nous avons donné au $\mathrm{n^o}$~81 sur la limite d'une suite de courbes peut s'exprimer de la façon suivante. Pour que $\gamma_{n}$ ait $\gamma$ pour limite, il faut et il suffit que, pour chaque valeur de $n$, on puisse établir entre $\gamma_{n}$ et $\gamma$ une correspondance univoque et réciproque dans laquelle l'ordre soit conservé et cela de façon que si $M_{n}$ de $\gamma_{n}$ correspond à $M$ de $\gamma, M_{n}$ tende vers $M$, mais uniformément. En supposant cette condition remplie pour une certaine correspondance, on peut se demander si elle serait aussi remplie pour toute autre correspondance univoque et conservant l'ordre. Autrement dit, soit
\begin{equation*}
x=\varphi_{n}(t), \quad y=\psi_{n}(t), \quad z=\chi_{n}(t) \qquad\qquad (0 \leqslant t \leqslant 1) \tag{$8'$}
\end{equation*}
une représentation quelconque de $\gamma_{n}$. A une même valeur de $t$ correspondent d'après (8), (8'), (4) deux points $M_{n}, M_{n}^{\prime}$ de $\gamma_{n}$ et un point $M$ de $\gamma$. Il s'agit de savoir ce que devient $M_{n}^{\prime}$ à la limite.

Il est facile de voir que lorsque $M$ restant fixe, $n$ croit indéfiniment: $1^{\circ}$ le point correspondant $M_{n}^{\prime}$ a au moins un point limite; $2^{\circ}$ tout point limite de $M_{n}^{\prime}$ est un point de $\gamma$ (qui peut être distinct de $M$). Mais la réciproque n'est pas vraie. Autrement dit, quand on fait prendre à $M$ toutes les positions possibles sur $\gamma$, l'ensemble des points limites des points correspondants $M_{n}^{\prime}$ est situé sur $\gamma$, mais ne remplit toujours la courbe $\gamma$. Si, par exemple, on prend
$$
\varphi_{n}(t) \equiv f_{n}\left[\alpha_{n}(t)\right], \quad \psi_{n}(t) \equiv g_{n}\left[\alpha_{n}(t)\right], \quad \chi_{n}(t) \equiv h_{n}\left[\alpha_{n}(t)\right]
$$
avec
$$
\alpha_{n}(t)=t e^{n(t-1)},
$$
les formules ($8'$) donneront bien une représentation de $\gamma_{n}$ puisque $\alpha_{n}(t)$ est une fonction continue qui croit constamment de $0$ à $1$. Cependant, on voit que pour $t \neq 1: \varphi_{n}(t),\, \psi_{n}(t),\, \chi_{n}(t)$ tendent vers $f(0), g(0), h(0)$, et pour $t=1,\, \varphi_{n}(1),\, \psi_{n}(1),\, \chi_{n}(1)$ tendent vers $f(1), g(1), h(1)$. Donc les points $M_{n}^{\prime}$ tendent tous vers l'une ou l'autre des extrémités de $\gamma$.

Cela montre en particulier, que si l'on considère un ensemble $E$ de courbes et si l'on prend pour chacune d'elles une représentation paramétrique quelconque, il n'est pas certain, lorsqu'une suite de courbes de $E$ a une limite, que les représentations analytiques correspondantes aient une limite.\\

\textbf{84.} 
\textit{\textbf{L'ensemble des courbes forme une classe $(E)$ normale.}} --- Pour arriver à l'application de nos théorèmes généraux, il ne nous reste plus qu'à prouver que la classe des courbes qui, d'après ce qui précède, est déjà une classe $(E)$, est aussi une classe $(E)$ normale.

I. Je dis qu'elle est séparable. En effet, nous avons vu ($\mathrm{n^o}$ 56) qu'on peut former, une fois pour toutes, une suite $S$ de fonctions continues
$$
A_{1}(t), A_{2}(t), \ldots, A_{n}(t), \ldots,
$$
telle que toute fonction continue soit un des éléments limites de cette suite. Alors, si l'on considère une représentation (4) d'une courbe $\gamma$, on pourra trouver trois fonctions de cette suite $A_{p_{n}}(t), A_{q_{n}}(t), A_{r_{n}}(t)$, telles que l'on ait
$$\left|f(t)-A_{p_{n}}(t)\right|<\cfrac{1}{n}, \quad\left|g(t)-A_{q_{n}}(t)\right|<\cfrac{1}{n}, \quad\left|h(t)-A_{r_{n}}(t)\right|<\cfrac{1}{n} \qquad(0 \leqslant t \leqslant 1)$$ 
et on pourra toujours choisir ces fonctions non constantes à la fois dans un même intervalle. Cela prouve que l'on peut considérer $\gamma$ comme courbe limite d'une suite de courbes extraite de l'ensemble $D$ des courbes
$$
x=A_{p}(t), \quad y=A_{q}(t), \quad z=A_{r}(t) \qquad\qquad(0 \leqslant t \leqslant 1),
$$
où $A_{p}, A_{q}, A_{r}$ sont trois fonctions continues extraites de la suite $S$ et non constantes à la fois dans un même intervalle. Or l'ensemble $D$ est évidemment dénombrable. Nous arrivons donc à cette conclusion qui (outre l'intérêt qu'elle présente par la suite) est bien curieuse en elle-même:

\textsc{\textbf{Théorème.}} --- \textit{On peut tracer une fois pour toutes dans l'espace à trois dimensions une suite dénombrable de courbes continues}\footnote{On peut même supposer, d'après le mode de construction de la suite $S$, que ces lignes continues sont toutes des courbes unicursales, ou sont toutes des lignes polygonales chacune d'un nombre fini de côtés.}:
$$
\gamma_{1}, \gamma_{2}, \ldots, \gamma_{n}, \ldots,
$$
\textit{telle que toute courbe de l'espace soit limite d'au moins une suite convenablement extraite de la première.}

II. Montrons maintenant que le théorème de \textsc{Cauchy} sur la convergence d'une suite peut s'étendre au cas d'une suite de courbes:

\textsc{\textbf{Théorème.}} --- \textit{La condition nécessaire et suffisante pour qu'une suite de courbes $C_{1}$, $C_{2}, \ldots$ tende vers une courbe limite est que, quel que soit $\varepsilon>0$, on puisse trouver un entier $n$ vérifiant l'inégalité $\left(C_{n}, C_{n+p}\right)<\varepsilon$ quel que soit l'entier $p$.}

La condition est évidemment nécessaire. Pour démontrer qu'elle est suffisante, il suffit de montrer que, si elle est vérifiée, l'ensemble est compact. En effet, si l'on peut extraire de la suite de \textsc{Cauchy} $C_{1}, C_{2}, \ldots$ une suite $C_{n_{1}}, C_{n_{2}}, \ldots$ (d'indices croissants), qui tend vers une courbe $C$, alors la suite donnée convergera aussi vers $C$.

Pour former la suite $C_{n_{1}}, C_{n_{2}}, \ldots$, observons que, d'après l'hypothèse, on peut toujours choisir $n_{q}$ assez grand pour que l'on ait, quel que soit l'entier $p$,
$$
\left(C_{n_{q}}, C_{n_{q+p}}\right)<\cfrac{1}{q^{2}}\,.
$$

Nous savons qu'étant donnée la représentation
$$
x=f_{q}(t), \quad y=g_{q}(t), \quad z=h_{q}(t) \qquad\quad\qquad\qquad(0 \leqslant t \leqslant 1)
$$
de $C_{n_{q}}$, nous pourrons toujours choisir celle de $C_{n_{q+1}}$
$$
x=f_{q+1}(t), \quad y=g_{q+1}(t), \quad z=h_{q+1}(t) \qquad\qquad (0 \leqslant t \leqslant 1),
$$
de façon que l'on ait
$$
\sqrt{\left[f_{q}(t)-f_{q+1}(t)\right]^{2}+\left[g_{q}(t)-g_{q+1}(t)\right]^{2}+\left[h_{q}(t)-h_{q+1}(t)\right]^{2}}<\left(C_{n_{q}}, C_{n_{q+1}}\right)+\varepsilon,
$$
$\varepsilon$ étant aussi petit que l'on veut. Prenons en particulier $\varepsilon=\cfrac{1}{q^{2}}$. On voit alors qu'on pourra choisir successivement les représentations de $C_{n_{1}}, C_{n_{2}}, \ldots$ de façon que l'on ait, quel que soit $q$,
$$
\left|f_{q}(t)-f_{q+1}(t)\right|<\cfrac{2}{q^{2}}, \quad\left|g_{q}(t)-g_{q+1}(t)\right|<\cfrac{2}{q^{2}}, \quad\left|h_{q}(t)-h_{q+1}(t)\right|<\cfrac{2}{q^{2}} \,.
$$

Alors, étant donné $\omega>0$, si l'on choisit un nombre $q_{\mathrm{t}}$ tel que l'on ait
$$
\cfrac{2}{q_{1}^{2}}+\cfrac{2}{\left(q_{1}+1\right)^{2}}+\cdots<\omega
$$
(comme cela est toujours possible), on voit facilement que l'on aura, quel que soit l'entier $p$,
$$
\left|f_{q_{1}}(t)-f_{q_{1}+p}(t)\right|<\omega, \quad\left|g_{q_{1}}(t)-g_{q_{1}+p}(t)\right|<\omega, \quad\left|h_{q_{1}}(t)-h_{q_{1}+p}(t)\right|<\omega \,.
$$
Cela montre que les fonctions $f_{q}(t), g_{q}(t), h_{q}(t)$ convergent uniformément vers trois fonctions continues $f(t), g(t), h(t)$, lorsque $q$ croît indéfiniment. Si ces trois fonctions sont constantes de 0 à 1, alors $C_{n_{1}}, C_{n_{2}}, \ldots, C_{n_{q}}, \ldots$, tendent vers un point. Si ces trois fonctions ne sont pas constantes dans l'intervalle $(0,1)$, il faudrait, pour montrer que $C_{n_{1}}, C_{n_{2}}, \ldots$ tendent vers une courbe limite, prouver que $f(t), g(t), h(t)$ ne sont à la fois constantes dans aucun intervalle. Ou plutôt, il faudrait prouver qu'on peut choisir les représentations de $C_{n_{1}}, C_{n_{2}}, \ldots, C_{n_{q}}, \ldots$ de façon qu'elles convergent vers des fonctions continues qui ne soient à la fois constantes dans aucun intervalle.

Pour cela, nous nous appuierons sur ce que, si $f, g, h$ ne sont pas constantes de 0 à 1, on peut former une fonction $a(t)$ allant sans jamais décroître de 0 à 1 et qui n'est constante que dans les intervalles où $f, g, h$ sont à la fois constantes\footnote{Voir la \textsc{Note I} à la fin du Mémoire.}.

Alors, si l'on pose $u=a(t)$, à toute valeur de $u$ correspond un seul système de valeurs de $f(t), g(t), h(t)$, soit $F(u), G(u), H(u)$. Il y a donc trois fonctions $F, G$, $H$ déterminées pour chaque valeur de $u$ et telles que l'on ait
$$
f(t) \equiv F[a(t)], \quad g(t) \equiv G[a(t)], \quad h(t) \equiv H[a(t)] \qquad(0 \leqslant t \leqslant 1) .
$$
Montrons d'abord que les formules
$$
x=F(u), \quad y=G(u), \quad z=H(u) \qquad\qquad\qquad\qquad(0 \leqslant u \leqslant 1)
$$
définissent une courbe. D'après l'hypothèse faite sur $a(t), F, G, H$ ne peuvent être à la fois constantes dans un même intervalle. Je dis qu'elles sont continues; autrement dit, s'il existe une suite de valeurs de $u: u_{1}, u_{2}, \ldots, u_{n}, \ldots$ qui convergent vers une limite $u_{0}$, on aura par exemple
$$
F\left(u_{0}\right)=\lim _{n=\infty} F\left(u_{n}\right) .
$$
En effet, dans l'ensemble borné des nombres $F\left(u_{1}\right), F\left(u_{2}\right), \ldots$, on peut former une suite $F\left(u_{1}^{\prime}\right), F\left(u_{2}^{\prime}\right), \ldots$ qui converge vers une limite déterminée $\alpha_{0}$; il suffit de démontrer que, quelle que soit la façon dont on forme cette suite, on a toujours $\alpha_{0}=F\left(u_{0}\right)$. Or, à chacun des nombres $u_{n}^{\prime}$, l'égalité $u=a(t)$ fait correspondre au moins un nombre $t_{n}^{\prime}$ tel que $u_{n}^{\prime}=a\left(t_{n}^{\prime}\right)$. Les nombres $t_{1}^{\prime}, t_{2}^{\prime}, \ldots$ étant bornés, on peut extraire de leur suite une suite $t_{p_{1}}^{\prime}, t_{p_{2}}^{\prime}, \ldots$ ayant une limite $t_{0}$; et puisque $a(t)$ est continue, on aura:
$$
a\left(t_{0}\right)=\lim _{n=\infty} a\left(t_{p_{n}}^{\prime}\right)=\lim _{n=\infty} u_{p_{n}}^{\prime}=u_0 .
$$

Mais $f(t)$ est aussi continue, donc
$$
F\left(u_{0}\right)=F\left[a\left(t_{0}\right)\right]=f\left(t_{0}\right)=\lim _{n=\infty} f\left(t_{p_{n}}^{\prime}\right)=\lim _{n=\infty} F\left(u_{p_{n}}^{\prime}\right)=\alpha_{0} .
$$

Ainsi $F(u)$ est bien continue; de même pour $G, H$.

Ceci étant, posons $a_{n}(t)=\left(1-\cfrac{1}{n}\right) a(t)+\cfrac{t}{n}$. Pour chaque valeur de $n, a_{n}(t)$ est une fonction continue et croissante de $t$. [Lorsque $n$ croit indéfiniment, cette fonction tend uniformément vers $a(t)]$. Donc la fonction inverse $t=b_{n}(u)$ est aussi une fonction continue et croissante. Par suite, si l'on pose
$$
F_{n}(u)=f_{n}\left[b_{n}(u)\right], \quad G_{n}(u)=g_{n}\left[b_{n}(u)\right], \quad H_{n}(u)=h_{n}\left[b_{n}(u)\right],
$$
la courbe $C_{n}$ est aussi représentée par les formules
$$
x=F_{n}(u), \quad y=G_{n}(u), \quad z=H_{n}(u) \qquad\qquad (0 \leqslant u \leqslant 1)\,.
$$

Il suffit maintenant de prouver que $F_{n}(u), G_{n}(u), H_{n}(u)$ tendent uniformément vers $F(u), G(u), H(u)$. Or, on a
$$
\left|F\left[a_{n}(t)\right]-f_{n}(t)\right| \leqslant\left|F\left[a_{n}(t)\right]-F[a(t)]\right|+\left|f(t)-f_{n}(t)\right|\,.
$$

Les deux termes du second membre tendent uniformément vers zéro; il en est donc de même du premier. Mais si l'on pose $u=a_{n}(t)$, celui-ci devient $\left|F(u)-F_{n}(u)\right|$ et son maximum, pour une valeur donnée de $n$, est resté le même. Dès lors, le maximum du premier nembre tend vers zéro. Il en sera de même pour $\left|G(u)-G_{n}(u)\right|$ et pour $\left|H(u)-H_{n}(u)\right|$.\\

\textbf{85.} 
\textit{\textbf{Ensembles compacts de courbes.}} --- Nous avons vu ($\mathrm{n^o}$~35) que tout ensemble compact formé d'éléments d'une classe $(V)$ est limité. Nous pouvons mettre ici cet énoncé sous une forme plus géométrique, en introduisant la notion de domaine fini; nous appellerons ainsi un ensemble de points tel que la distance de deux quelconques d'entre eux reste inférieure à un nombre fixe. Alors, on voit facilement que la condition nécessaire et suffisante pour qu'un ensemble de courbes soit limité (c'est-à-dire pour que l'écart de deux quelconques des courbes de cet ensemble reste inférieur à un nombre fixe) est que toutes les courbes de cet ensemble soient contenues dans un même domaine fini. Il suffit pour le démontrer de s'appuyer sur ce que l'écart de deux courbes quelconques est au plus égal à la limite supérieure de la distance d'un point quelconque de l'une à un point quelconque de l'autre, et au moins égal au minimum de la distance d'un point quelconque fixe sur l'une à un point variable sur l'autre ($\mathrm{n^o}$~82). Ainsi nous voyons que \textit{tout ensemble compact de courbes est contenu dans un domaine fini}. Mais nous touchons maintenant à la plus grande différence qui existe entre les ensembles ponctuels (même à une infinité dénombrable de dimensions) et les ensembles de courbes. En effet, contrairement à ce qui se passe pour les ensembles ponctuels, \textit{un ensemble de courbes situées dans un même domaine fini n'est pas nécessairement un ensemble compact}. Il suffit pour s'en rendre compte de considérer par exemple l'ensemble $E$ des courbes 
$$C_{n} \qquad\qquad x=2 \pi t, \quad y=\sin 2^{n} \pi t, \quad z=0 \qquad\qquad (0 \leqslant t \leqslant 1)\,,$$
toutes contenues dans le même cercle $\displaystyle x^{2}+y^{2} \leqslant 5 \pi^{2}$.

Il est impossible que l'on puisse tirer de cet ensemble de courbes une suite de courbes ayant une limite, car l'écart de deux quelconques d'entre elles est au moins égal à 1. On peut toujours, en effet, trouver dans une correspondance continue entre deux quelconques d'entre elles $C_{n}$ et $C_{p}$ un point $M$ sur $C_{n}$ dont la distance au point correspondant soit $\geqslant 1$. Pour le voir, observons qu'il y a sur la sinusoïde $C_{n}, 2^{n-1}$ points $A_{1}, A_{2}, \ldots, A_{2^{n-1}}$ dont l'ordonnée est 1 , et $2^{n-1}$ points $A_{1}^{\prime}, A_{2}^{\prime}, \ldots, A_{2^{n-1}}^{\prime}$ dont l'ordonnée est $-1$. Supposons $n>p$; il nous suffira de montrer que, dans une correspondance continue quelconque, l'un au moins des points $A_{1}, A_{2}, \ldots$ de $C_{n}$ correspond à un point de $C_{p}$ d'ordonnée négative ou nulle, ou que l'un des points $A_{1}^{\prime}$, $A_{2}^{\prime}, \ldots$ de $C_{n}$ correspond à un point de $C_{p}$ d'ordonnée positive ou nulle; alors on aurait bien deux points correspondants dont la distance serait supérieure ou égale à 1. 
Or, admettons qu'il existe une correspondance $G$ où il n'en soit pas ainsi, et appelons $b_{1}, b_{2}, \ldots, b_{1}^{\prime}, b_{2}^{\prime}, \ldots$ les points de $C_{p}$ qui correspondent à $A_{1}, A_{2}, \ldots$ et à $A_{1}^{\prime}$, $A_{2}^{\prime}, \ldots$, dans la correspondance considérée $G$. 
Les ordonnées de $b_{1}, b_{2}, \ldots$ seraient positives, celles de $b_{1}^{\prime}, b_{2}^{\prime}, \ldots$ seraient négatives, et on rencontrerait ces points dans l'ordre $b_{1}, b_{1}^{\prime}, b_{2}, b_{2}^{\prime}, \ldots$, en parcourant $C_{p}$. 
Il y aurait donc un point d'intersection de $C_{p}$ avec $O x$ aux deux extrémités et sur chacun des arcs distincts $b_{1} b_{1}^{\prime}, b_{1}^{\prime} b_{2}, b_{2} b_{2}^{\prime}$, $b_{2}^{\prime} b_{3}, \ldots, b_{2^{n-1}} b_{2^{n-1}}^{\prime}$; en tout au moins $2^{n}+1$ points d'intersection de $C_{p}$ avec $O x$; ce qui est impossible, puisque $C_{p}$ rencontre $O x$ en $2^{p}+1$ points et que $p<n$.\\

\textbf{86.} 
\textit{\textbf{Condition pour qu'un ensemble de courbes soit compact.}} --- Ce qui précède montre qu'il y a lieu de chercher une condition supplémentaire qui permette d'affirmer qu'un ensemble de courbes contenues dans un domaine fini est un ensemble compact. M. \textsc{Arzelà} a obtenu cette condition suffisante par une application immédiate de son théorème sur les fonctions également continues (\textsc{v}, page 344). Il résulte en effet de ce théorème que, lorsque l'on considère un système $R$ de représentations simultanées
$$
C \qquad\qquad\qquad\qquad x=f(t), \quad y=g(t), \quad z=b(t) \qquad\qquad\qquad(0 \leqslant t \leqslant 1)
$$
d'un ensemble $E$ de courbes $C$, on pourra affirmer que cet ensemble de courbes est compact si $R$ est formé de fonctions $f, g, h, \ldots$, également continues et bornées dans leur ensemble.

Ce théorème extrêmement important se prête à un grand nombre d'applications. Mais il y a lieu de le compléter à deux points de vue. D'abord, il serait bon d'énoncer sous forme géométrique une proposition qui s'applique à des éléments géométriques comme les courbes. Ensuite M. \textsc{Arzelà} n'a pas donné de réciproque à son théorème. Or celle-ci pourrait se comprendre de deux manières : on pourrait d'abord penser que, si l'on considère un système $R$ de représentations simultanées de courbes d'un ensemble $E$, les fonctions de $R$ seront nécessairement bornées dans leur ensemble et également continues lorsque $E$ est compact. \textit{Cet énoncé est inexact}. En effet, considérons une courbe non fermée $C$:
\begin{equation*}
x=f(t), \quad y=g(t), \quad z=h(t) \tag{$0\leqslant t\leq1$}
\end{equation*}
et le système $R$ de représentations
$$
x=\cfrac{1}{n}+f\left(e^{-n\left(\frac{1-u^{2}}{u^{2}}\right)}\right), \quad y=\cfrac{1}{n}+g\left(e^{-n\left(\frac{1-u^{2}}{u^{2}}\right)}\right), \quad z=\cfrac{1}{n}+h\left(e^{-n\left(\frac{1-u^{2}}{u^{2}}\right)}\right),
$$
qui fournit, pour chaque valeur de $n$, une représentation acceptable d'une courbe $C_{n}$. L'ensemble $E$ des courbes $C_{n}$ est compact, car une autre représentation acceptable de $C_{n}$ est
$$
x=\cfrac{1}{n}+f(t), \quad y=\cfrac{1}{n}+g(t), \quad z=\cfrac{1}{n}+h(t) \qquad\qquad (0 \leqslant t \leqslant 1)
$$
et on voit que $C_{n}$ tend vers $C$ quand $n$ croît indéfiniment.

Pourtant les fonctions de $R$ ne sont pas également continues, car, quels que soient les nombres positifs $\varepsilon$ et $\eta$ on peut toujours trouver un nombre $u$ et un entier $p$ tel que l'on ait
$$
0<1-u<\eta \qquad\left|f_{n}(u)-f_{n}(1)\right|>\varepsilon,
$$
pour $n>p$, en posant
$$
f_{n}(u) \equiv \cfrac{1}{n}+f\left(e^{-n\left(\frac{1-\mathrm{u}^{2}}{u^{2}}\right)}\right)\,.
$$

La seconde manière d'énoncer la réciproque qu'on pourrait être tenté de donner au théorème d'\textsc{Arzelà} (et qui, cette fois-ci, est exacte) est la suivante: \textit{si un ensemble de courbes est compact, il existe toujours au moins un système de représentations simultanées de ces courbes}
$$
x=f(t),\; y=g(t),\; z=h(t) \qquad\qquad(0 \leqslant t \leqslant 1)
$$
\textit{tel que les fonctions $f, g, h, \ldots$ soient bornées dans leur ensemble et également continues.}

On pourrait trouver cette proposition directement, mais nous scinderons la démonstration en deux parties, dont l'une nous permettra d'énoncer ensuite \textit{sous forme géométrique} la condition pour qu'un ensemble de courbes soit compact.\\

\textbf{87.} 
\textit{\textbf{Ensembles de courbes uniformément divisibles.}} --- Pour arriver à la proposition annoncée, nous commencerons par transformer la condition de M. \textsc{Arzelà} en une autre qu'on peut énoncer géométriquement, c'est-à-dire qui ne fait intervenir aucune représentation paramétrique déterminée des courbes de l'ensemble.

Nous appellerons d'abord \textit{oscillation d'un arc} $P\,Q$ d'une courbe $A\,B$ le maximum de la distance de deux points quelconques appartenant à cet arc. Nous dirons alors que les courbes d'un ensemble $E$ sont \textit{uniformément divisibles} lorsque, quel que soit le nombre $\varepsilon>0$, on peut trouver un entier $n$ tel que toute courbe de $E$ puisse être décomposée en $n$ arcs consécutifs dont les oscillations soient toutes inférieures à $\varepsilon$.

Il est facile de voir que, \textit{si un ensemble de courbes est compact, les courbes de cet ensemble sont uniformément divisibles}. En effet, dans le cas contraire on pourrait trouver un nombre $\varepsilon>0$ tel que, quel que soit $n$, il existe au moins une courbe $C_{n}$ de l'ensemble, qui ne puisse être décomposée en $n$ arcs dont les oscillations soient inférieures à $\varepsilon$. Or l'ensemble étant compact, on peut extraire de la suite $C_{1}, C_{2}, \ldots$ une suite $C_{n_{1}}, C_{n_{2}}, \ldots, C_{n_{p}}, \ldots$ ayant une limite $C$ et on sait ($\mathrm{n^o}$ 81) qu'on pourra choisir les représentations de $C_{n_{p}}$ et de $C$:
$$
\left.\begin{array}{ll}
x=F_{p}(t), \quad y=G_{p}(t), \quad z=H_{p}(t) \\
x=F(t), \;\quad y=G(t), \;\,\quad z=H(t)
\end{array}\;\right\} \qquad\qquad 0 \leqslant t \leqslant 1
$$
de façon que $F_{p}, G_{p}, H_{p}$, tendent uniformément vers $F, G, H$. Alors, quel que soit $\varepsilon$, on pourra choisir $p$ assez grand pour que l'on ait, quel que soit $t$:
$$
\left|F_{p}(t)-F(t)\right|<\cfrac{\varepsilon}{9}\,, \quad\left|G_{p}(t)-G(t)\right|<\cfrac{\varepsilon}{9}\,, \quad\left|H_{p}(t)-H(t)\right|<\cfrac{\varepsilon}{9} \,.
$$

D'autre part, divisons $C_{n_{p}}$ en $n_{p}$ arcs successifs déterminés par les valeurs de $t: 0,\, \cfrac{1}{n_{p}},\, \cfrac{2}{n_{p}},\, \cfrac{3}{n_{p}}, \ldots, 1$. Si $t, t^{\prime}$ appartiennent à l'un de ces intervalles, on aura $\left|t-t^{\prime}\right| \leqslant \cfrac{1}{n_{p}}$. Or on peut choisir $p$ assez grand pour que l'inégalité $\left|t-t^{\prime}\right| \leqslant \cfrac{1}{n_{p}}$ entraîne:
$$
\left|F(t)-F\left(t^{\prime}\right)\right|<\cfrac{\varepsilon}{9}\,, \quad\left|G(t)-G\left(t^{\prime}\right)\right|<\cfrac{\varepsilon}{9}\,, \quad\left|H(t)-H\left(t^{\prime}\right)\right|<\cfrac{\varepsilon}{9} \,;
$$
alors, pour $p$ assez grand on aura dans chacun des $n_{p}$ arcs en lesquels on aura décomposé $C_{n_{p}}$:
$$
\left|F_{p}(t)-F_{p}\left(t^{\prime}\right)\right|<\left|F_{p}(t)-F(t)\right|+\left|F\left(t^{\prime}\right)-F_{p}\left(t^{\prime}\right)\right|+\left|F(t)-F\left(t^{\prime}\right)\right|<\cfrac{\varepsilon}{3}
$$
et de même pour $G, H$; d'où:
$$
\sqrt{\left|F_{p}(t)-F_{p}\left(t^{\prime}\right)\right|^{2}+\left|G_{p}(t)-G_{p}\left(t^{\prime}\right)\right|^{2}+\left|H_{p}(t)-H_{p}\left(t^{\prime}\right)\right|^{2}}<\varepsilon .
$$

Dès lors, on arrive à une contradiction, car on aurait divisé $C_{n_{p}}$ en $n_{p}$ arcs dont les oscillations sont au plus égales à $\varepsilon$.\\

\textbf{88.} 
Alors pour démontrer la réciproque par laquelle nous complétons le théorème de M. \textsc{Arzelà}, il nous suffira démontrer la proposition suivante:

\textsc{\textbf{Théorème.}} --- \textit{La condition nécessaire et suffisante pour que les courbes d'un ensemble $E$ soient uniformément divisibles et contenues dans un même domaine fini, est qu'il. existe au moins un système de représentations simultanées des courbes de $E$:}
\begin{equation*}
x=f(t), \quad y=g(t), \quad z=h(t) \qquad\qquad(0 \leqslant t \leqslant 1) \tag{9}
\end{equation*}
\textit{tel que les fonctions $f, g, h, \ldots$ soient également continues et bornées dans leur ensemble.}

Il est facile de voir que la condition est suffisante. Montrons qu'elle est nécessaire. Pour cela, nous partirons d'un premier système de représentations simultanées des courbes de l'ensemble, soit pour la courbe $C$:
\begin{equation*}
x=F(v), \quad y=G(v), \quad z=H(v) \qquad\qquad (0 \leqslant v \leqslant 1) \tag{10}
\end{equation*}

Nous pourrons supposer que $F, G, H$, ne sont constantes dans aucun intervalle, car en ce qui concerne les courbes de l'ensemble qui sont réduites à des points, l'oscillation est évidemment nulle. Ceci étant, cherchons à former la représentation (9) à partir de la représentation (10). Autrement dit, cherchons à déterminer pour chaque courbe $C$ une fonction $v=\psi(t)$ continue et croissante de 0 à 1 , de telle façon que toutes les fonctions $F[\psi(t)], G[\psi(t)], H[\psi(t)]$ soient également continues [elles seront toujours bornées dans leur ensemble quel que soit $\psi(t)$].

Or, d'après l'hypothèse, on peut, pour chaque courbe $C$, déterminer une suite de valeurs croissantes de $v$:
$$
0, \quad u_{1}^{(p)}, \quad u_{2}^{(p)}, \ldots, u_{n_{p}}^{(p)}, \quad 1,
$$
telles que les oscillations des arcs correspondants de $C$ soient toutes inférieures à $\cfrac{1}{p}$, les quantités $u_{q}^{(p)}$ variant avec la courbe $C$, mais leur nombre $n_{p}$, restant le même pour toutes les courbes $C$. En intercalant au besoin de nouveaux nombres dans la suite $S_{p}: 0, u_{1}^{(p)}, u_{2}^{(p)}, \ldots 1$, on voit facilement qu'on peut supposer vérifiées les conditions supplémentaires suivantes: la suite $S_{p+1}$ contient la suite $S_{p}$ et possède le même nombre de termes dans chacun des intervalles déterminés par $S_{p}$.

Ceci étant, faisons correspondre à chaque nombre $u_{q}^{(p)}$, le nombre $\tau_{q}^{(p)}=\cfrac{q}{n_{p}}$; il est facile de voir que si deux nombres $u: u_{q}^{(p)}, u_{q^{\prime}}^{\left(p^{\prime}\right)}$ ($p$ nécessairement différent de $p^{\prime}$) sont égaux, il en sera de même des nombres $\tau$ correspondants, et que si $u_{q}^{(p)}<u_{q^{\prime}}^{(p \prime)}$, on a $\tau_{q}^{(p)}<\tau_{q^{\prime}}^{\left(p^{\prime}\right)}$.\\

\textbf{89.} 
Nous allons maintenant définir, pour chaque courbe $C$, la fonction continue $t=\varphi(v)$ inverse de la fonction cherchée $v=\psi(t)$. Je dis qu'il suffit de la définir pour les valeurs de $v$ qui sont limites des quantités $u_{q}^{(p)}$. Autrement dit, si $v$ est un nombre quelconque de l'intervalle $(0,1)$, on peut trouver une suite de nombres $u_{q_{1}}^{(p_{1})}$, $u_{q_{2}}^{\left(p_{2}\right)}, \ldots$ qui tendent vers $v$. En effet, dans le cas contraire il y aurait un nombre $\varepsilon$ tel que, quel que soit $p$, chacun des arcs $(v-\varepsilon, v),(v, v+\varepsilon)$ soit compris dans un des $\operatorname{arcs}\left(u_{q}^{(p)}, u_{q+1}^{(p)}\right)$. Alors les oscillations des arcs $(v-\varepsilon, v)$ et $(v, v+\varepsilon)$ seraient inférieures à $\cfrac{1}{n_{p}}$ quel que soit $p$; par suite $F(v), G(v), H(v)$, seraient constants de $v-\varepsilon$ à $v+\varepsilon$, ce ${ }^{p}$ qui est contraire à l'hypothèse.

Alors, appelons $u_{q}^{\prime(p)}, u_{q}^{\prime \prime(p)}$ les nombres $u$ qui sont, les uns inférieurs, les autres supérieurs à $v$. Les nombres $\tau_{q}^{\prime(p)}, \tau_{q}^{\prime \prime(p)}$ correspondants forment deux classes de \textsc{Dirichlet}; c'est-à-dire que tout nombre de la première classe est inférieur à tout nombre de la seconde et qu'on peut trouver deux nombres, un dans chaque classe, dont la différence soit aussi petite que l'on veut. Il y a donc un nombre $t$, et un seul, compris entre ces deux classes. C'est ce nombre que nous allons prendre pour valeur de $\varphi(v)$. Dans le cas où $v$ est un des nombres $u_{q}^{(p)}$, la valeur de $\varphi(v)$ sera évidemment le nombre correspondant $\tau_{q}^{(p)}$.\\

\textbf{90.} 
On voit immédiatement que cette fonction $\varphi(v)$, bien définie pour toute valeur de $v$ entre 0 et 1, est croissante et croit de 0 à 1. Elle est aussi continue. En effet, soit $\omega$ un nombre positif quelconque; en prenant $p$ assez grand, on aura $n_{p}>\cfrac{2}{\omega}$. Le nombre $p$ étant ainsi choisi, soit $u_{q}^{(p)}$ le plus grand nombre de la suite $S_{p}$ qui est inférieur à $v$; alors les deux nombres $v-u_{q}^{(p)}, u_{q+2}^{(p)}-v$ seront positifs ; soit $\eta$ le plus grand. Je dis qu'on a pour $\left|v-v^{\prime}\right|<\eta$:
$$
\left|\varphi(v)-\varphi\left(v^{\prime}\right)\right|<\omega .
$$

En effet $v$ et $v^{\prime}$ se trouveront alors entre $u_{q}^{(p)}$ et $u_{q+2}^{(p)}$, donc:
$$
\left|\varphi(v)-\varphi\left(v^{\prime}\right)\right|<\varphi\left(u_{q+2}^{(p)}\right)-\varphi\left(u_{q}^{(p)}\right)=\cfrac{2}{n_{p}}<\omega .
$$

Ainsi nous avons bien formé, pour chaque courbe $C$, une fonction continue $t=\varphi(v)$ qui croît constamment de 0 à 1 . Alors la fonction inverse $v=\psi(t)$ est aussi croissante et continue, et on pourra former un système $R$ de représentations simultanées:
$$
x=f(t), \quad y=g(t), \quad z=h(t) \qquad\qquad (0\leqslant t \leqslant 1),
$$
en posant:
$$
f(t) \equiv F[\psi(t)], \quad g(t) \equiv G[\psi(t)], \quad h(t) \equiv H[\psi(t)] .
$$

Les fonctions du système $R$ seront bien également continues; en effet, d'après la formation de $\psi(t)$, l'oscillation de la courbe sera inférieure $\cfrac{1}{p}$ dans chacun des arcs limités par les valeurs de $t: 0, \cfrac{1}{n_{p}}, \cfrac{2}{n_{p}}, \ldots 1$ et les oscillations de $f(t), g(t), h(t)$ sont inférieures à celles de $C$. Dés lors on voit que, quel que soit $p$, on peut déterminer un nombre $\cfrac{1}{n_{p}}$ indépendant de la courbe $C$ considérée et tel que l'inégalité : $\left|t^{\prime}-t^{\prime \prime}\right|<\cfrac{1}{n_{p}}$ entraîne:
$$
\left|f\left(t^{\prime}\right)-f\left(t^{\prime \prime}\right)\right|<\cfrac{1}{p}\,, \quad\left|g\left(t^{\prime}\right)-g\left(t^{\prime \prime}\right)\right|<\cfrac{1}{p}\,, \quad\left|h\left(t^{\prime}\right)-h\left(t^{\prime \prime}\right)\right|<\cfrac{1}{p} \,.
$$

\textbf{91.}
En combinant les énoncés précédents, on obtient la condition nécessaire et suffisante pour qu'un ensemble de courbes soit compact sous une forme qui ne fait intervenir aucune représentation paramétrique des courbes de cet ensemble.

\textsc{\textbf{Théorème.}} --- \textit{La condition nécessaire et suffisante pour qu'un ensemble de courbes soit compact est que les courbes de cet ensemble soient contenues dans un même domaine fini et également divisibles.}\\

\textbf{92.} 
\textit{\textbf{Application aux courbes rectifiables.}} --- Appelons ligne polygonale inscrite dans une courbe, une ligne brisée ayant mêmes extrémités que la courbe et dont les sommets sont des points de la courbe que l'on trouve dans le même ordre quand on parcourt la courbe ou la ligne brisée. On démontre (\textsc{iv}, page 59) que, lorsque le maximum de la longueur des côtés d'une ligne polygonale inscrite dans un arc $A\, B$ tend vers zéro, le périmètre de cette ligne polygonale tend vers la limite supérieure des longueurs des lignes polygonales inscrites dans $A\, B$, et on appelle cette limite \textit{la longueur de la courbe}. On dit que la courbe est \textit{rectifiable} lorsque cette limite est finie.

Le théorème précédent permet d'affirmer qu'un ensemble de courbes rectifiables et contenues dans un même domaine fini est compact toutes les fois que les longueurs de ces courbes sont bornées dans leur ensemble\footnote{Un cas particulier de ce théorème a été démontré directement par M. \textsc{Hilbert} (\textsc{xx}). Puis la généralisation a été effectuée par M. \textsc{Lebesgue} dans sa Thèse (\textsc{xvii}).}. En effet, supposons que l'on divise chaque courbe de l'ensemble en $n$ arcs de longueurs égales. La longueur d'une courbe quelconque $C$ de l'ensemble est inférieure à un nombre fixe $L$ indépendant de $C$; donc chacun des arcs égaux sera de longueur inférieure à $\cfrac{L}{n}$. Or l'oscillation d'un arc est évidemment inférieure à la longueur de cet arc. Donc, en prenant $n$ assez grand $\left(n>\cfrac{L}{\varepsilon}\right)$, chaque courbe $C$ se trouvera divisée en arcs de longueurs inférieures à $\varepsilon$. Alors les courbes $C$ sont uniformément divisibles et leur ensemble est compact.\\

\textbf{93.} 
On pourrait se demander si la condition suffisante que nous venons d'énoncer est aussi nécessaire. La réponse est négative: \textit{On peut donner un exemple de courbes rectifiables situées dans un même domaine fini et formant un ensemble compact, sans que leurs longueurs soient bornées dans leur ensemble.}

Soit en effet:
$$
x=f(t), \quad y=g(t), \quad z=0 \qquad\qquad\qquad (0 \leqslant t \leqslant 1)\,,
$$
une représentation déterminée d'une courbe $C$ non rectifiable, mais dont les arcs: $\cfrac{1}{n} \leqslant t \leqslant 1$ sont rectifiables quel que soit $n$. Il nous suffira de considérer les courbes $C_{n}$ :
$$
\begin{gathered}
x=\cfrac{1}{n}+f\left[\cfrac{1}{n}+u\left(1-\cfrac{1}{n}\right)\right], \quad y=\cfrac{1}{n}+g\left[\cfrac{1}{n}+u\left(1-\cfrac{1}{n}\right)\right], \quad z=0 \\
(0 \leqslant u \leqslant 1) .
\end{gathered}
$$

Ces courbes forment un ensemble compact, car il est évident que $C_{1}, C_{2}, \ldots$ tendent vers $C$. Elles sont rectifiables et contenues dans un même domaine fini. Leurs longueurs qui sont celles des arcs $\cfrac{1}{n} \leqslant t \leqslant 1$ de la courbe $C$ ne sont cependant pas bornées dans leur ensemble.

Il est d'ailleurs bien facile de construire une courbe telle que celle dont nous avons admis l'existence; on peut prendre par exemple la spirale hyperbolique obtenue en posant:
$$
f(t) \equiv t \cos \cfrac{1}{t}, \quad g(t) \equiv t \sin \cfrac{1}{t}\,.
$$

\textit{On peut même donner un exemple de courbes contenues dans un même domaine fini et formant un ensemble compact sans qu'aucune d'elles soit rectifiable.}

Il suffit de reprendre la courbe $C$ que nous venons de considérer, et de considérer les courbes $C_{n}$ :
$$
x=\cfrac{1}{n}+f(t), \quad y=\cfrac{1}{n}+g(t), \quad z=0 \qquad\qquad(0 \leqslant t \leqslant 1) .
$$

\subsection*{Application des théorèmes généraux.}
Nous pouvons maintenant appliquer les résultats de la Première Partie aux ensembles de courbes et aux fonctions de lignes.

\textbf{94.} 
\textit{\textbf{Ensembles de courbes.}}

\textsc{\textbf{Théorème.}} --- \textit{Soit $E$ un ensemble quelconque d'arcs de courbes continues. ${1^\circ}$ L'ensemble dérivé de $E$ est fermé. $2^{\circ}$ On peut extraire de $E$, une suite dénombrable $D$ de courbes de $E$, telle que toute courbe de $E$ appartienne à $D$, ou soit une courbe limite de D. $3^{\circ}$ Ou bien $E$ est dénombrable ou bien il existe une courbe $C_{1}$ de $E$ telle que, pour toute valeur de $\varepsilon$, il $y$ ait une infinité non dénombrable de courbes de $E$ contenues entièrement dans le volume engendré par une sphère de rayon $\delta$ et dont le centre parcourt $C_{1}$.}

\textsc{\textbf{Théorème.}} --- \textit{Soit $G$ un ensemble de courbes uniformément divisibles $(\mathrm{n^o}\; 87)$ et contenues dans un même domaine fini: Les éléments de $G$, qui ne sont pas des limites de courbes de $G$, forment un ensemble dénombrable.}

\textsc{\textbf{Théorème.}} --- \textit{Si l'ensemble précédent $G$ est aussi fermé, autrement dit, si $G$ est un ensemble extrémal quelconque: $1^{\circ}$ on peut le décomposer en un ensemble dénombrable et un ensemble parfait ou nul sans éléments communs; $2^{\circ}$ il existe un ensemble de courbes dont l'ensemble dérivé coïncide avec $E$.}

\textsc{\textbf{Théorème.}} --- \textit{Tout ensemble parfait de courbes a la puissance du continu.}

On pourra aussi énoncer les théorèmes des $\mathrm{n^{os}}\; 40,42,43,45, \ldots$ en prenant comme éléments des courbes continues.\\

\textbf{95.} 
\textit{\textbf{Fonctions de lignes.}} --- Les opérations qui portent sur des arcs de courbes ont reçu de M. \textsc{Voiterra} le nom de \textit{fonctions de lignes}.

M. \textsc{Voiterra} a réussi à montrer comment on pourrait définir la dérivée d'une fonction de lignes et a obtenu, à ce point de vue, des résultats extrêmement intéressants (\textsc{xv}).

Dans un article des Annales scientifiques de l'École Normale (\textsc{xxvii}), j’ai donné quelques propriétés de fonctions de lignes dont les dérivées au sens de M. Volterra ont une forme spéciale donnée.

Je laisserai ici de côté ce genre de recherches qui s'écartent un peu de notre objet actuel: l'étude des propriétés communes aux opérations continues \textit{les plus générales}.

Les résultats généraux s'appliquent encore aux fonctions de lignes.

\textsc{\textbf{Théorème.}} --- Toute fonction de lignes, continue dans un ensemble extrémal de courbes : $1^{\circ}$ est bornée dans cet ensemble, $2^{\circ}$ y atteint chaque extremum. \textit{Inversement, si toutes les fonctions de lignes continues dans un même ensemble $E$ de courbes, $1^{\circ}$ sont chacune bornée, $2^{\circ}$ atteignent chacune leur extremum en au moins une courbe de l'ensemble, cet ensemble est nécessairement extrémal.}

\textsc{\textbf{Théorème.}} --- \textit{Soit $E$ un ensemble fermé de courbes contenues dans un même domaine fini et uniformément divisibles: $1^{\circ}$ Pour qu'une suite de fonctions de lignes $U_{1}, U_{2}, \ldots$ continues dans $E$ converge vers une fonction de lignes qui soit continue dans $E$, il faut et il suffit que la suite converge quasi-uniformément. $2^{\circ}$ Pour que des fonctions de lignes, continues dans $E$ forment une famille $\mathfrak{F}$ telle que l'on puisse extraire de toute infinité d'éléments de $\mathfrak{F}$ une suite de fonctions de lignes qui convergent uniformément dans $E$, il faut et il suffit que les fonctions de lignes de $\mathfrak{F}$ soient bornées dans leur ensemble et également continues dans $E$.}

\subsection*{Ensembles et fonctions de surfaces.}

\textbf{96.}
On peut développer pour les surfaces une théorie qui nous mènerait à des propositions entièrement analogues à celles qui précèdent. Mais il y a au début des précautions à prendre, qui conduisent à quelques longueurs. Aussi, pour ne pas allonger ce Mémoire, renverrons-nous sur ce point à une publication ultérieure.

\section*{NOTE I.}
\subsection*{Construction d'une fonction continue non décroissante qui n'est constante que dans des intervalles donnés.}

\textbf{97.}
Considérons un ensemble $G$ d'intervalles $I$ sans points communs situés sur l'axe des $x$ dans le segment fondamental $(0, 1)$. Nous allons montrer que l'on peut former une fonction continue $\varphi(x)$ qui va sans jamais décroître de 0 à 1 et qui n'est constante que dans chacun des intervalles $I$ \footnote{Nous utilisons cette proposition au $\mathrm{n^o}$ 84.}.

En effet, observons d'abord que l'ensemble $G$ est dénombrable, car c'est l'ensemble des ensembles $G_{n}$ formés chacun par les intervalles $I$ dont les longueurs sont supérieures à $\cfrac{1}{n+1}$, et au plus égales à $\cfrac{1}{n}$. Or il $y$ a évidemment un nombre fini ($\leqslant n$) d'intervalles $I$ dans $G_{n}$, puisque les $I$ n'ont aucun point commun.

On peut donc ranger ces intervalles en une suite dénombrable $I_{1}, I_{2}, I_{3}, \ldots$; d'après ce qui précède la longueur de $I_{n}$ tendra vers zéro avec $\cfrac{1}{n}$, à moins qu'il n'y ait qu'un nombre fini de ces intervalles. Dans ce dernier cas, il n'y a aucune difficulté à former $\varphi(x)$.\\

\textbf{98.} 
Supposons donc qu'il y ait une infinité d'intervalles $I$. L'ensemble $P$ des points du segment $(0,1)$ qui ne sont intérieurs au sens étroit à aucun des intervalles $I$, est un ensemble parfait (\textsc{ii}, page 12).

$1^{\circ}$. Examinons d'abord le cas où $P$ comprend les points 0 et 1 et n'est dense dans aucun intervalle entre 0 et 1. On sait alors (\textsc{ii}, page 14), que l'on peut établir une correspondance univoque et réciproque entre tous les intervalles $I$, d'une part, et tous les nombres rationnels positifs $<1$, d'autre part, et cela de telle façon que deux éléments correspondants soient disposés de la même manière sur $O x$. 
Appelons $u_{n}$ le nombre rationnel que l'on fait ainsi correspondre à $I_{n}$. Soit maintenant $x$ un point quelconque du segment $(0,1)$, autre que 0 et 1. 
Appelons $I^{\prime}$ un quelconque des intervalles $I$ qui ne sont pas complètement à droite de $x, I^{\prime \prime}$ un quelconque des intervalles $I$ qui ne sont pas entièrement à gauche de $x$. Si l'on appelle $u^{\prime}$ et $u^{\prime \prime}$ les nombres rationnels correspondants, on voit que tout nombre rationnel compris entre 0 et 1 doit être un $u^{\prime}$ ou un $u^{\prime \prime}$, et que l'on a toujours $u^{\prime} \leqslant u^{\prime \prime}$. 
On définit ainsi deux classes de nombres qui comprennent entre elles un seul nombre que nous appellerons $\varphi(x)$. 
Si nous posons en outre $\varphi(0)=0$, $\varphi(1)=1$, on voit que nous avons défini $\varphi(x)$ en tout point du segment $(0, 1)$. En particulier, en tout point d'un intervalle $I_{n}$, on aura $\varphi(x)=u_{n}$. 
La fonction $\varphi(x)$ est donc constante dans chacun des intervalles $I_{n}$. Je dis maintenant que si $x<x^{\prime}$, on a nécessairement $\varphi(x)<\varphi\left(x^{\prime}\right)$, si $x$ et $x^{\prime}$ n'appartiennent pas à un même intervalle $I$. En effet, il suffit d'observer que, sous cette hypothèse, il y a au moins un intervalle $I_{n}$ qui est entièrement compris à l'intérieur de ($x, x^{\prime}$). Alors, d'après le mode de construction de $\varphi(x)$, on aura:
$$
\varphi(x)<u_{n}<\varphi\left(x^{\prime}\right) .
$$

Ainsi $\varphi(x)$ est une fonction non décroissante qui va de 0 à 1 et qui n'est constante que dans chacun des intervalles $I$. Par suite, on peut définir, en chaque point $x$, la limite supérieure $\varphi(x-0)$ des valeurs de $\varphi\left(x^{\prime}\right)$ pour $x^{\prime}<x$, et on aura $\varphi(x-0) \leqslant \varphi(x)$. Or $\varphi(x-0)$ est au moins égale à la limite supérieure $\varphi(x)$ des valeurs de $\varphi\left(x^{\prime}\right)$ quand $x^{\prime}$ est dans un quelconque des intervalles $I$ et reste $<x$. Donc $\varphi(x)=\varphi(x-0)$. Autrement dit, $\varphi(x)$ est continue à gauche; de même, elle est continue à droite. En définitive, la fonction $\varphi(x)$ est continue et répond bien aux conditions annoncées.

$2^{\circ}$. Supposons maintenant que $P$, comprenant encore 0 et 1, puisse être dense dans certains intervalles. Alors on pourra former une seconde suite d'intervalles $K_{1}, K_{2}, \ldots$ dont tous les points, extrémités comprises, sont des points de $P$, et telle que l'ensemble $Q$ des points qui n'appartiennent au sens étroit ni aux $K$, ni aux $I$, ne soit dense dans aucun intervalle. Plaçons alors dans chaque intervalle $K_{n}$ une suite d'intervalles sans points communs: $K_{n}^{(1)}, K_{n}^{(2)}, \ldots$, telle que l'ensemble des points de $K_{n}$ qui n'appartiennent à aucun des intervalles $K_{n}^{(1)}, K_{n}^{(2)}, \ldots$ soit de mesure nulle (\textsc{ii}, page 16) \footnote{Par exemple, on pourra placer dans $K_{n}$ un ensemble d'intervalles semblable à l'ensemble complémentaire [dans le segment $(0,1)$] de l'ensemble de \textsc{Cantor} cité plus loin.}. Enfin appelons $R$ l'ensemble des points qui n'appartiennent au sens étroit à aucun des intervalles $I_{1}, I_{2}, \ldots ; K_{1}^{(1)}, K_{1}^{(2)}, \ldots ; K_{2}^{(1)}, K_{2}^{(2)}, \ldots$

D'après leur formation, ces intervalles n'ont aucun point commun (au contraire un $I$ et un $K$ pourraient avoir une extrémité commune). L'ensemble $R$ est donc parfait, contient 0 et 1, et n'est dense dans aucun intervalle. On peut donc former une fonction continue non décroissante $\varphi_{1}(x)$ qui n'est constante que dans les intervalles $I_{n}$ ou $K_{n}^{(p)}$. Appelons d'autre part $\varphi_{2}(x)$ la mesure de l'ensemble des points de $P$ compris entre $0$ et $x$. 
C'est une fonction continue non décroissante; de plus cette fonction est constante dans les intervalles $I$ et elle est certainement croissante dans les intervalles $K_{n}^{(p)}$. 
Donc la fonction $\varphi(x)=\cfrac{\varphi_{1}(x)+\varphi_{2}(x)}{\varphi_{1}(1)+\varphi_{2}(1)}$ est une fonction continue non décroissante qui va de 0 à 1 et qui n'est constante que dans les intervalles $I$; elle répond donc à la question.

$3^{\circ}$. Enfin si $P$ ne contient pas à la fois 0 et 1, autrement dit si l'un des intervalles $I$ est terminé en 0 ou en 1, on est ramené aux cas précédents en supprimant cet intervalle.\\

\textbf{99.} 
Il y a un cas particulier intéressant où l'on peut former explicitement la fonction $\varphi(x)$. C'est celui où $P$ est l'ensemble de \textsc{Cantor} de mesure nulle (\textsc{ii}, page 12). Considérons un nombre quelconque $x$ compris entre $0$ et $1$ et écrivons sa valeur dans le système de numération de base 3:
$$
x=0, a_{1} a_{2} a_{3} \ldots
$$

Les nombres $a_{1}, a_{2}, \ldots$ ne pourront prendre que les valeurs 0, 1, 2 et on peut toujours supposer que l'on ait écrit un nombre tel que:
$$
0,\, a_{1}\, a_{2}\, \ldots a_{n}\, 0\, 2\, 2\, 2 \ldots
$$
ou
$$
0,\, b_{1}\, b_{2}\, \ldots b_{p}\, 2\,0\,0\,0 \ldots
$$
sous la forme respectivement équivalente:
$$
0, \, a_{1} \, a_{2}\, \ldots a_{n}\, 1\,0\,0\,0 \ldots
$$
ou
$$
0,\, b_{1}\, b_{2}\, \ldots b_{p}\, 1\,2\,2\,2 \ldots
$$

Ceci étant, nous poserons toujours:
$$
\varphi\left(0, a_{1}\, a_{2} \ldots\right)=0^{\prime}, b_{1}\, b_{2} \ldots,
$$
$0^{\prime}, \ldots$ indiquant qu'on passe dans le système de base 2 et en prenant en général pour $b_{n}$ un nombre égal à 0 si l'un des nombres $a_{1}, a_{2}, \ldots, a_{n-1}$ est égal à 1, et dans le cas contraire égal à 1 si $a_{n}=2$, et égal à $a_{n}$ si $a_{n} \neq 2$. Autrement dit, nous posons:
$$
\begin{gathered}
\varphi\left(\cfrac{a_{1}}{3}+\cfrac{a_{2}}{3^{2}}+\cdots \cfrac{a_{n}}{3^{n}}+\cdots\right) \\
=\cfrac{\alpha\left(a_{1}\right)}{2}+\cfrac{\alpha\left(a_{2}\right) \beta\left(a_{1}\right)}{2^{2}}+\cdots+\cfrac{\alpha\left(a_{n}\right) \beta\left(a_{1}\right) \ldots \beta\left(a_{n-1}\right)}{2^{n}}+\cdots,
\end{gathered}
$$
avec les conditions:
$$
\alpha(0)=0, \quad \alpha(1)=\alpha(2)=1, \quad \beta(1)=0, \quad \beta(0)=\beta(2)=1 .
$$

Il est facile de voir qu'on fait ainsi correspondre une même valeur de $\varphi(x)$ à tous les nombres $x$ tels que
$$
x=0, c_{1}\, c_{2} \ldots c_{n} \,1 \,\lambda_{1} \, \lambda_{2} \ldots,
$$
où $c_{1}, c_{2}, \ldots, c_{n}$ restent fixes et tous différents de $1$.

Ces points forment un intervalle; la correspondance ainsi établie entre cet intervalle et la valeur constante de $\varphi(x)$ est précisément celle qu'a indiquée M. \textsc{Cantor} pour prouver que l'ensemble $P$ a la puissance du continu.

\section*{NOTE II.}
\subsection*{Sur le calcul effectif de l'écart de deux courbes.}

\textbf{100.}
La théorie que nous avons développée dans la \textsc{Première Partie} montre qu'une fois établie l'existence d'un écart, la valeur même de cet écart n'a plus une très grande importance. Autrement dit, il suffit de savoir qu'on peut définir un nombre satisfaisant aux conditions générales de l'écart ($\mathrm{n^o}$ 49), sans avoir à se préoccuper de la manière dont on pourrait le calculer effectivement. Cela est d'autant plus vrai qu'on pourrait choisir une infinité d'autres définitions de l'écart moyennant lesquelles la théorie générale pourrait se développer exactement de la même manière et qui ne changeraient pas les courbes limites d'un ensemble de courbes. Par exemple, si $e$ est l'écart de deux courbes tel que nous l'avons défini, on pourrait le remplacer partout par $3 e$ ou par $\sqrt{e}$ ou par $\cfrac{e}{1+e}$. Mais la définition primitive a l'avantage de donner pour l'écart de deux courbes réduites à deux points une quantité égale à la distance de ces deux points; et pour deux courbes, l'une fixe, l'autre qui s'éloigne à l'infini un nombre qui tend vers l'infini.

La définition de l'écart que nous avons donnée ne fait pas prévoir comment on pourrait le calculer effectivement, et ce calcul serait certainement très difficile en général. On peut cependant donner des exemples simples où ce calcul est possible. En général, on devra procéder de la manière suivante. On prouvera que, dans toute correspondance continue entre les deux courbes, le maximum $d$ de la distance de deux points correspondants est supérieur ou égal à un nombre fixe e. On montrera ensuite qu'il existe au moins une de ces correspondances où ce maximum $d$ est exactement égal à $e$.

Par exemple, considérons deux segments rectilignes $\overline{A B}, \overline{A^{\prime} B^{\prime}}$ et soit $\Delta$ la plus grande des deux longueurs $A A^{\prime}, B B^{\prime}$. On a toujours $d \geqslant \Delta$ et l'on a $d=\Delta$ lorsque la correspondance est telle que deux points correspondants $M, M^{\prime}$ divisent l'un $\overline{A B}$, l'autre $\overline{A^{\prime} B^{\prime}}$, dans le même rapport. Donc l'écart des deux segments est égal à $\Delta$.

On peut être aussi amené à définir l'écart de deux courbes fermées. On le considérera alors comme la limite inférieure de tous les écarts qu'on obtiendrait en les considérant de toutes les manières possibles comme des arcs de courbes ayant chacun deux extrémités en coïncidence. On verrait alors facilement que si l'on considère deux circonférences de rayons $R_{1}, R_{2}$, de centres $O_{1}, O_{2}$, situées dans le même plan et orientées de la même façon, leur écart est $O_{1} O_{2}+\left|R_{1}-R_{2}\right|$.

Un exemple moins particulier est le suivant. Considérons dans un même plan deux courbes \textit{convexes} $C_{1}$ et $C_{2}$, la courbe $C_{1}$ étant supposée à tangente continue et toute entière contenue dans $C_{2}$. Dans ces conditions, on peut voir que l'écart de $C_{1}$ et de $C_{2}$ est égal au maximum du segment intercepté par $C_{2}$ sur la normale extérieure à $C_{1}$.

Dans ces exemples, on vérifie immédiatement que l'évanouissement de l'écart est la condition nécessaire et suffisante pour que les deux courbes coïncident, ce qui permet souvent de prévoir la valeur probable de l'écart.\\

Paris, le 2 avril 1906.\\

\textsc{Maurice Fréchet.}

\newpage
\subsection*{AUTEURS CITÉS.}
{\small 

\noindent\textbf{Collection de Monographies sur la Théorie des fonctions}

\noindent Publiée sous la direction de \textsc{Émile Borel} (Paris, Gauthier-Villars):
\begin{enumerate}
    \item[(\textsc{i})] \textsc{Borel}, \emph{Leçons sur la théorie des fonctions. Éléments de la théorie des ensembles et applications}, 1898.
    \item[(\textsc{ii})] \textsc{Borel}, \emph{Leçons sur les fonctions de variables réelles et les développements en séries de polynômes}, 1905.
    \item[(\textsc{iii})] \textsc{Baire}, \emph{Leçons sur les fonctions discontinues}, 1905.
    \item[(\textsc{iv})] \textsc{Lebesgue}, \emph{Leçons sur l'intégration et la recherche des fonctions primitives}, 1904.
\end{enumerate}

\medskip

\noindent\textbf{Articles de M.~\textsc{Arzelà}}
\begin{enumerate}
    \item[(\textsc{v})] \emph{Funzioni di linee}, \emph{Rendiconti della R.~Accademia dei Lincei}, 1889, vol.~V, 1\textsuperscript{o} semestre, pp.~342--348.\\
    \emph{Sulle funzioni di linee}, \emph{Memorie della R.~Accademia delle Scienze dell'Istituto di Bologna, sezione delle Scienze Fisiche e Matematiche}, s.~V, t.~V (1895), pp.~55--74.
    
    \item[(\textsc{vi})] \emph{Sull'integrabilità delle equazioni differenziali ordinarie}, \emph{Ibid.}, s.~V, t.~V (1895), pp.~75--88.\\
    \emph{Sull'esistenza degli integrali nelle equazioni differenziali ordinarie}, \emph{Ibid.}, s.~V, t.~VI (1896), pp.~33--42.
    
    \item[(\textsc{vii})] \emph{Sulle serie di funzioni}, \emph{Ibid.}, s.~V, t.~VIII (1899--1900), pp.~3--58, 91--134.
    
    \item[(\textsc{viii})] \emph{Sull'inversione di un sistema di funzioni}, \emph{Rendiconto delle sessioni della R.~Accademia delle Scienze dell'Istituto di Bologna}, nuova serie, vol.~VII (1902--1903), pp.~182--201.\\
    \emph{Sulle serie di funzioni ugualmente oscillanti}, \emph{Ibid.}, nuova serie, vol.~VIII (1903--1904), pp.~143--154.\\
    \emph{Sul principio di Dirichlet}, \emph{Ibid.}, nuova serie, vol.~I (1896--1897), pp.~71--84.
    
    \item[(\textsc{ix})] \emph{Sulle serie di funzioni di variabili reali}, \emph{Ibid.}, nuova serie, vol.~VII (1902--1903), pp.~22--32.
    
    \item[(\textsc{x})] \emph{Sulle serie di funzioni analitiche}, \emph{Ibid.}, nuova serie, vol.~VII (1902--1903), pp.~33--42.
\end{enumerate}

\medskip

\noindent\textbf{Divers}
\begin{enumerate}
    \item[(\textsc{xi})] \textsc{Hadamard}, \emph{Sur les opérations fonctionnelles}, \emph{Comptes Rendus de l'Académie des Sciences}, t.~CXXXVI (1\textsuperscript{er} semestre 1903), pp.~351--354.
    
    \item[(\textsc{xii})] \textsc{Hadamard}, \emph{Sur certaines applications possibles de la théorie des ensembles}, \emph{Verhandlungen des ersten Internationalen Mathematiker-Kongresses} (1897), pp.~201--202.
    
    \item[(\textsc{xiii})] \textsc{Borel}, \emph{Contribution à l'analyse arithmétique du continu}, \emph{Journal de Mathématiques pures et appliquées}, 5\textsuperscript{e} série, t.~IX (1903), pp.~329--375.
    
    \item[(\textsc{xiv})] \textsc{Borel}, \emph{Sur quelques points de la théorie des fonctions}, \emph{Annales scientifiques de l'École Normale supérieure}, 3\textsuperscript{e} série, t.~XII (1895), pp.~9--55.
    
    \item[(\textsc{xv})] \textsc{Volterra}, \emph{Sur une généralisation de la théorie des fonctions d'une variable imaginaire}, \emph{Acta Mathematica}, t.~XII (1889), pp.~233--286.
    
    \item[(\textsc{xvi})] \textsc{Pincherle}--\textsc{Amaldi}, \emph{Le operazioni distributive e le loro applicazioni all'Analisi} (Bologna, 1901).
    
    \item[(\textsc{xvii})] \textsc{Lebesgue}, \emph{Intégrale, Longueur, Aire}, \emph{Annali di Matematica pura ed applicata}, s.~III, t.~VII (1902), pp.~231--359.
    
    \item[(\textsc{xviii})] \textsc{Le Roux}, \emph{Les fonctions d'une infinité de variables indépendantes}, \emph{Nouvelles Annales de Mathématiques}, 4\textsuperscript{e} série, t.~IV (1904), pp.~448--458.
    
    \item[(\textsc{xix})] \textsc{Le Roux}, \emph{Recherches sur les équations aux dérivées partielles}, \emph{Journal de Mathématiques pures et appliquées}, 5\textsuperscript{e} série, t.~IX (1903), pp.~403--455.
    
    \item[(\textsc{xx})] \textsc{Hilbert}, \emph{Sur le principe de Dirichlet} (traduction de M.~Laugel), \emph{Nouvelles Annales de Mathématiques}, 3\textsuperscript{e} série, t.~XIX (1900), pp.~337--344.
    
    \item[(\textsc{xxi})] \textsc{Drach}, \emph{Essai sur une théorie générale de l'intégration et sur la classification des transcendantes}, \emph{Annales scientifiques de l'École Normale supérieure}, 3\textsuperscript{e} série, t.~XV (1898), pp.~243--384.
    
    \item[(\textsc{xxii})] \textsc{Ascoli}, \emph{Le curve limiti di una varietà data di curve}, \emph{Memorie della classe di Scienze Fisiche, Matematiche e Naturali della R.~Accademia dei Lincei}, vol.~XVIII (1883), pp.~521--586.
    
    \item[(\textsc{xxiii})] \textsc{Zoretti}, \emph{Sur les fonctions analytiques uniformes qui possèdent un ensemble parfait discontinu de points singuliers}, \emph{Journal de Mathématiques pures et appliquées}, 6\textsuperscript{e} série, t.~I (1905), pp.~1--51.
    
    \item[(\textsc{xxiv})] \textsc{de Séguier}, \emph{Éléments de la théorie des groupes abstraits} (Paris, Gauthier-Villars, 1904).
    
    \item[(\textsc{xxv})] \textsc{Montel}, \emph{Sur les suites de fonctions analytiques}, \emph{Comptes Rendus de l'Académie des Sciences}, t.~CXXXVIII (1\textsuperscript{er} semestre 1904), pp.~469--471.
    
    \item[(\textsc{xxvi})] \textsc{Bourlet}, \emph{Sur les opérations en général et les équations différentielles linéaires d'ordre infini}, \emph{Annales scientifiques de l'École Normale supérieure}, 3\textsuperscript{e} série, t.~XIV (1897), pp.~133--190.
    
    \item[(\textsc{xxvii})] \textsc{Fréchet}, \emph{Sur les fonctions de lignes fermées}, \emph{Annales scientifiques de l'École Normale supérieure}, 3\textsuperscript{e} série, t.~XXI (1904), pp.~557--571.\\
    \emph{Sur une extension de la méthode de Jacobi--Hamilton}, \emph{Annali di Matematica pura ed applicata}, s.~III, t.~XI (1905), pp.~187--199.\\
    \emph{Sur les opérations linéaires}, \emph{Transactions of the American Mathematical Society}, t.~V (1904), pp.~493--499; t.~VI (1905), pp.~134--140.
\end{enumerate}
}

\end{document}
