# Supplementary material for: A Brief History of Fr\'echet Distances: From Curves and Probability Laws to FID
Source: arXiv:2604.21745 source file (2026-04-23)
Supplement: Supplementary file 2 [file frechet1957_fr.tex]

% !TeX program = pdflatex

\documentclass[10pt]{article}
\usepackage[utf8]{inputenc}
\usepackage[T1]{fontenc}
\usepackage[english,french]{babel}

\usepackage{libertinus}
\usepackage{libertinust1math}

\usepackage{amsmath}
\usepackage{amsfonts}
\usepackage{amssymb}
\usepackage[version=4]{mhchem}
\usepackage{stmaryrd}
\usepackage{mathrsfs}
\usepackage{bbold}
\usepackage{newunicodechar}
\usepackage[hidelinks]{hyperref}
\usepackage{anyfontsize}

\setlength{\parskip}{0.6\baselineskip}%

\title{\Large SUR LA DISTANCE DE DEUX LOIS DE PROBABILIT\'E}
\author{Maurice Fr\'echet}
\date{}

%New command to display footnote whose markers will always be hidden
\let\svthefootnote\thefootnote
\newcommand\blfootnotetext[1]{%
  \let\thefootnote\relax\footnote{#1}%
  \addtocounter{footnote}{-1}%
  \let\thefootnote\svthefootnote%
}

%Overriding the \footnotetext command to hide the marker if its value is `0`
\let\svfootnotetext\footnotetext
\renewcommand\footnotetext[2][?]{%
  \if\relax#1\relax%
    \ifnum\value{footnote}=0\blfootnotetext{#2}\else\svfootnotetext{#2}\fi%
  \else%
    \if?#1\ifnum\value{footnote}=0\blfootnotetext{#2}\else\svfootnotetext{#2}\fi%
    \else\svfootnotetext[#1]{#2}\fi%
  \fi
}

\sloppy

\begin{document}
\maketitle

\noindent RESUME: L'auteur indique une expression explicite de la distance de deux lois de probabilités, selon la première définition de Paul Lévy. Il indique aussi une modification commode de cette définition.

\subsection*{INTRODUCTION}
M. Paul Lévy a résolu tant de problèmes qu'il n'a pas toujours eu le temps d'exploiter toutes ses idées.

Par exemple, il a donné \footnote{Voir p. 329 de la 2e édition de notre ouvrage: "Recherches théoriques modernes sur le Calcul des Probabilités (Premier livre), chez Gauthier-Villars, 1950.} trois intéressantes définitions de la distance "de deux lois de probabilité" en laissant aux lecteurs le soin de les utiliser.

J'ai pensé qu'une bonne manière de rendre hommage à l'oeuvre si riche de M. Paul Lévy, consisterait à prolonger son étude.

Après une brève comparaison de ses trois définitions, j'étudierai plus particulièrement la première.

Mon étude a été facilitée par les résultats énoncés dans ma note aux C.R. \footnote{Tome 242, 1956, p. 2426-2428.} \underline{"Sur les tableaux de corrélation dont les marges sont données"} et par l'application qui en a été donnée par Bass \footnote{C.R. 21 février 1955, tome 240, n$^{\circ}$ 8.} et par Dall'Aglio \footnote{Sugli estremi dei momenti delle funzione di ripartizione doppia (Ann. Scuole Norm. Sup. di Pisa, Sc. Fis. a Mat., série III, Vol. X, 1956, p. 35-74)}.\\

\noindent \underline{\textbf{Rappel}:}

Rappelons que :

Une distance est définie sur un ensemble $E$ si l'on associe à tout couple $a, b$ d'éléments de $E$, un nombre réel appelé distance de $a$ et de $b$ et représenté par la notation ($a, b$), de façon à vérifier les conditions suivantes :

$1^{\circ}\; ({a}, {b})=({b}, {a}) \geqslant 0 ;$

$2^{\circ}\;({a}, {b}) \neq 0$ si $a$ et $b$ sont considérés comme distincts dans $E$ et inversement;

$3^{\circ}\;$ Pour 3 éléments quelconques ${a}, {b}, {c}$ de $E$ , on a "l'inégalité triangulaire":
$$
(a, b) \leqslant(a, c)+(c, b) .
$$

En outre, dire que $a_{n}$ de $E$ \underline{converge} vers $a$ de $E$, c'est dire que la distance $\left(a_{n}, a\right)$ tend vers zéro avec $\frac{1}{n}$.\\

\noindent \underline{\textbf{Distinction entre deux "distances"}:}

Appliquons cette définition au Calcul des Probabilités. Dans cette théorie, il y a deux distances à distinguer. Soient $X, Y$ deux éléments aléatoires, déterminés \underline{simultanément} dans chaque épreuve d'une catégorie déterminée.

On peut définir une distance $(X, Y)$ de $X, Y$ dans une épreuve déterminée. Mais il y a aussi intérêt à définir une "distance globale" de $X$ et $Y$ dans \underline{l'ensemble} des épreuves. Nous représenterons cette distance globale par la notation:
$$
(\,[{X}],\,[{Y}]\,) .
$$

Il faudra s'assurer à chaque fois que les conditions $1^{\circ}, 2^{\circ}, 3^{\circ}$ sont vérifiées. Mais en général, on conviendra, en ce qui concerne la condition $2^{\circ}$, de considérer comme non distincts deux éléments aléatoires qui ne sont que "presque certainement" identiques. Par exemple, nous avons prouvé que:
$$
\operatorname{Prob}(X \neq Y)
$$
est une distance globale.

Une distance globale plus souvent considérée est rappelée en note ci-après. Pour nous en tenir au cas où $X$, $Y$ sont deux \underline{nombres} aléatoires, observons que pour déterminer une distance globale, il ne suffit pas de connaître les fonctions de répartitions respectives:
$$
F(x)=\operatorname{Prob}(x<x) ;\; G(y)=\operatorname{Prob}(Y<y)
$$
qui déterminent les lois de probabilité $L, L^{\prime}$ de $X$ et de $Y$, mais aussi la fonction de répartition:
$$
H(x, y)=\operatorname{Prob}(x<x \text { et } Y<y)
$$
du couple ordonné ${X}, {Y}$ \footnote{ Par exemple, on prend souvent comme "distance globale" de $X$ et de $Y$, la quantité
$$
\sqrt{\mathfrak{M}_{H}(X-Y)^{2}}=\sqrt{\int_{-\infty}^{+\infty} \int_{-\infty}^{+\infty}(x-y)^{2} d_{x} d_{y} H(x, y)}
$$}.

Au contraire, la distance ($L, L^{\prime}$) des deux lois $L, L^{\prime}$, doit être déterminée indépendamment de $H(x, y)$ par $F(x)$ et $G(y)$.

Les deux dernières définitions de ($L, L^{\prime}$) par $P$. Lévy sont purement analytiques. Elles se présentent comme modifications de définitions traditionnelles en Analyse de la distance de deux fonctions $F$ et $G$, modifications motivées par les discontinuités possibles des deux fonctions $F$ et $G$.

La première définition proposée par M. Paul Lévy est, au contraire, une définition qui pourrait légitimement paraître arbitraire et artificielle (si on l'énonçait sous forme purement analytique) à un mathématicien ignorant du Calcul des Probabilités. Elle fait, en effet, appel à la notion de nombre aléatoire et c'est quand on fait effectivement appel à cette notion qu'elle prend, au contraire, un sens intuitif et naturel.

Il va être curieux de constater que cette première définition conduit à une expression explicite assez simple de la distance, contrairement à ce qu'on aurait pu attendre.\\

\noindent \underline{\textbf{Rappel}:}

La première définition proposée par M. Paul Lévy est la suivante:

La distance de deux lois de probabilité ${L}, {L}^{\prime}$, dont les fonctions de répartition sont ${F}({x}), {G}({y})$, est la borne inférieure des "distances globales" de deux nombres aléatoires $X, Y$ dont la fonction de répartition $H(x, y)$ est quelconque pourvu qu'elle donne à ${X}, {Y}$, séparément, les fonctions de répartition $F(x), G(y)$.\\

\noindent \underline{\textbf{Marges}:}

On peut dire, si l'on veut, que ${F}({x}), {G}({y})$ sont les "marges" du "tableau de corrélation" défini par ${H}({x}, {y})$.

Il nous sera précieux d'utiliser le résultat énoncé dans notre Note aux C.R. du 14 mai 1956 rappelée ci-dessus, suivant lequel, l'ensemble des fonctions ${H}({x}, {y})$ n'est autre que celui des fonctions de répartition comprises (extremités incluses) entre les fonctions de répartition $H_{0}(x, y)$ et $H_{1}(x, y),\left(H_{0} \leqslant H_{1}\right)$, définies par
$$
\begin{aligned}
& H_{0}(x, y)=\operatorname{Sup}[(F(x)+G(y)-1), 0] \\
& H_{1}(x, y)=\operatorname{Inf}[F(x), G(y)] .
\end{aligned}
$$

Observons que dans cette première définition intervient une distance globale de $X$ et de $Y$ qui peut s'interpréter de différentes façons. Nous en avons donné un premier exemple p. 2 et un second en Note (1), p. 2. Autre exemple: pour obtenir une distance globale de $X$ et $Y$, soit:
$$
(\,[{X}],\,[{Y}]\,)
$$
qui tende vers zéro quand $X$ tend vers $Y$ en probabilité et réciproquement, nous avons proposé de prendre pour cette distance la borne inférieure quand le nombre positif $\varepsilon$ varie, de la somme
$$
\varepsilon+\operatorname{Prob}(|X-Y|>\varepsilon)
$$

On peut aussi prendre pour distance globale de $X$ et de $Y$ , la valeur moyenne de $f(|X-Y|)$ où $f$ est une fonction continue, croissante bornée, définie pour $x \geqslant 0$, nulle pour $x=0$ et telle que $f(a+b) \leqslant f(a)+f(b)$ (On peut d'ailleurs se contenter de conditions un peu plus générales; voir $2^{\circ}$ et $3^{\circ}$ parties de mon article paru en 1957 dans le Giornale Italiane Attuari). J'ai donné comme exemples de $f(x)$ les fonctions $\dfrac{x}{1+x}$, |th $x,\left|1-e^{-x}\right|(1)$. \footnote{Voir pour ces deux définitions, les p. 205 et 226 de la $2^{{e}}$ Edition de mes \underline{"Recherches théoriques modernes, sur le Calcul des Probabilités"}, Gauthier-Villars , (1950).}\\

\noindent \textbf{\underline{Les conditions d'existence d'une distance:}}

Pour sa première définition de la distance de deux lois $L, L^{\prime}$, Lévy montre que cette distance satisfait à la condition $3^{\circ}$ ci-dessus p. 2. Il est évident que la condition $1^{\circ}$ est satisfaite. La question est moins simple pour la condition $2^{\circ}$.

Il est clair cependant que si deux lois $L, L^{\prime}$ sont identiques, l'un des couples $X, Y$ satisfaisant respectivement à ces deux lois sera le couple $X$, $X$ dont la distance est nulle. La borne inférieure des distances ($[{X}],[{Y}]$) sera donc nulle et ($L, L^{\prime}$) sera ainsi nul. Le point le plus délicat est la proposition inverse. Quand $\left(L, L^{\prime}\right)=0$, $L, L^{\prime}$ sont-elles nécessairement identiques?

Précisons par la notation $([{X}],[{Y}])_{{H}}$ le fait qu'il s'agit de la distance globale de $X$ et $Y$ quand la fonction de répartition de leur couple est $H(x, y)$.

Dans le cas où cette distance \underline{atteint} sa borne inférieure ($L, L^{\prime}$) pour au moins une fonction $H$ particulière, soit $K(x, y)$, alors, par définition de $([{X}],[{Y}])_{{H}}$ si cette quantité est nulle, $X$ et $Y$ sont non distincts (ou bien identiques dans toute épreuve ou bien "presque certainement" égaux) et alors $F(x) \equiv G(y)$, c'est-à-dire $L \equiv L^{\prime}$. Mais si la borne inférieure n'est pas atteinte, le raisonnement est moins simple.

Dire que $\left(L, L^{\prime}\right)=0$, c'est dire qu'il existe pour tout $n$ entier, un couple $X_{n}, Y_{n}$ \underline{admissible} (\underline{c'est-à-dire} tel que $X_{n}, Y_{n}$ aient pour lois respectives $L, L^{\prime}$) pour lequel la distance :
\begin{equation*}
\left(\left[X_{n}\right],\left[Y_{n}\right]\right)<\frac{1}{n} . \tag{1}
\end{equation*}

Mais on n'a pas prescrit d'avance le choix adopté pour cette dernière distance. Et nous avons montré qu'on peut en concevoir beaucoup qui vérifient les conditions $1^{\circ}, 2^{\circ}, 3^{\circ}$ ci-dessus et qui soient conformes à notre intuition.

Par exemple, nous avons montré qu'on peut définir des distances $([{X}],[{Y}])$ très différentes ayant la propriété commune suivante:

La condition nécessaire et suffisante pour que:
$$
\lim_{n \rightarrow \infty}\left(\left[x_{n}\right],[x]\right)=0
$$
est que $X_{n}$ converge "en probabilité" vers $X$ quand $n \rightarrow \infty$.

Adoptons une telle définition dans l'énoncé de la définition de la distance de deux lois $L, L^{\prime}$.

Partons de (1),on a, pour tout ${r}>0$:
\begin{align*}
G(x-\varepsilon) & =\operatorname{Prob}\left[Y_{n}<x-\varepsilon\right] \leqslant \operatorname{Prob}\left[X_{n}<x\right]+\operatorname{Prob}\left[\left|X_{n}-Y_{n}\right|>\varepsilon\right]  \tag{2}\\
& =F(x)+\operatorname{Prob}\left(\left|X_{n}-Y_{n}\right|>\varepsilon\right) .
\end{align*}

Pour les différentes définitions que nous avons données d'une distance de deux nombres aléatoires, compatible avec la convergence en probabilité, on a aussi:
\begin{equation*}
([{X}],[{Y}])=([{X}-{Y}], 0) . \tag{3}
\end{equation*}

Par suite, d'après (1) et (3), on a:
$$
\left(\left[X_{n}-Y_{n}\right], 0\right)<\frac{1}{n}
$$
donc $X_{n}-Y_{n}$ converge vers zéro en probabilité c'est-à-dire que:
\begin{equation*}
0=\lim_{n \rightarrow \infty} \operatorname{Prob}\left(\left|X_{n}-Y_{n}\right|>\varepsilon\right) \tag{4}
\end{equation*}
pour tout $\varepsilon>0$. Alors d'après (2), en faisant croître $n$ vers l'infini, on a:
$$
G(x-\varepsilon) \leqslant F(x) \;\, \text { pour tout } \;\; \varepsilon>0 .
$$
Et comme ${G}({x})$ est continu à gauche:
$$
G(x) \leqslant F(x) .
$$
Mais on verrait de même que:
$$
F(x) \leqslant G(x) \,;
$$
donc: $F(x)=G(x)$.

Ainsi, s'il n'était pas évident que la condition $2^{\circ}$ soit satisfaite, cela est maintenant démontré, au moins quand la définition de ($L, L^{\prime}$) est appliquée dans le cas où la distance de deux nombres aléatoires satisfait aux conditions ci-dessus.

\noindent \underline{\textbf{Cas où ( $[{X}],[{Y}]$ ) était égal à l'écart quadratique moyen de $X$ et $Y$.}}

Dans la suite, nous prendrons d'abord comme distance globale de deux nombres aléatoires $X$ et $Y$, leur écart quadratique moyen
$$
\sqrt{\mathfrak{M}_{H}(X-Y)^{2}}\, .
$$
(Pour préciser, nous écrirons $\mathfrak{M}_{{H}}$ pour rappeler qu'il s'agit de la moyenne quand la fonction de répartition du couple ($X, Y$) est $H(x, y)$).

Alors la distance $\Delta$ des lois de probabilité $L, L'$ caractérisées par les fonctions de répartition $F(x)$ et $G(y)$ pourra être représentée par la formule:
$$
\Delta^{2}=\underset{H}{\operatorname{Inf}}\,\mathfrak{M}_{H}(X-Y)^{2}
$$

Observons qu'on a:
$$
(X-Y)^{2} \leqslant 2\left(X^{2}+Y^{2}\right) \text { d'où : } \mathfrak{M}_{H}(X-Y)^{2} \leqslant 2 \mathfrak{M}_{H} X^{2}+2 \mathfrak{M}_{H} Y^{2} .
$$

Donc si $\mathfrak{M}_{H}(X-Y)^{2}$ est infini, l'une au moins des quantités:
$$
\int_{-\infty}^{+\infty} x^{2} d F(x)=\mathfrak{M}_{H} X^{2} \quad \int_{-\infty}^{+\infty} y^{2} d G(y)=\mathfrak{M}_{H} Y^{2}, \text { est infinie. }
$$

Pour éviter des complications, nous supposerons que $F(x)$ et $G(x)$ sont les fonctions de répartition de nombres aléatoires ayant chacun un \underline{écart quadratique moyen fini}. Alors $\mathfrak{M}_{{H}}({X}-{Y})^{2}$ sera nécessairement fini. De plus, $X$ et $Y$ pris séparément, ont, sous la même hypothèse, des moyennes finies et déterminées:
$$
{a}=\mathfrak{M} {X} \quad, \quad {a}^{\prime}=\mathfrak{M} {Y} ;
$$
soient aussi $\sigma, \sigma^{\prime}$, leurs écarts quadratiques moyens. Alors,
$$
{Z}=\frac{{X}-{a}}{\sigma} \quad, \quad {T}=\frac{{Y}-{a}^{\prime}}{\sigma^{\prime}}
$$
seront les nombres aléatoires \underline{réduits} correspondant à $X$ et $Y$. C'est-à-dire que les moyennes de $Z$ et $T$ sont nulles et leurs écarts quadratiques moyens égaux à l'unité. On aura:
$$
\begin{gathered}
\mathfrak{M}_{{H}}({X}-{Y})^{2}=\mathfrak{M}\left({a}-{a}^{\prime}+\sigma {Z}-\sigma^{\prime} {T}\right)^{2} \\
=\left({a}-{a}^{\prime}\right)^{2}+2\left({a}-{a}^{\prime}\right)\left(\sigma \mathfrak{M} {Z}-\sigma{ }^{\prime} \mathfrak{M} {T}\right)+\sigma^{2} \mathfrak{M} {Z}^{2}-2 \sigma \sigma^{\prime} \mathfrak{M} {ZT}+\sigma^{\prime 2} \mathfrak{M} {~T}^{2}
\end{gathered}
$$
qui, d'après ce qui précède, se réduit à \footnote{Cette expression a été donnée déjà dans le cas de nombres aléatoires discrets par Salvemini dans: "L'indice quadratico di dissomiglianza era distribuzione gaussiane". Atti della XIV Reunione Scientifica, Societa Italiana di Statistica, 1954.
}
\begin{equation*}
\left(a-a^{\prime}\right)^{2}+\sigma^{2}-2 \sigma \sigma^{\prime} r+\sigma^{\prime 2} 
\end{equation*} 
en désignant, quand $\sigma \sigma^{\prime} \neq 0$, par $r$ le coefficient de corrélation (linéaire) de $X$ et de $Y$. On sait que $|r| \leqslant 1$. On peut donc poser $r=\cos \theta$, d'où
\begin{equation*}
\sqrt{\mathfrak{M}_{H}(X-Y)^{2}}=\sqrt{\left(a-a^{\prime}\right)^{2}+\left(\sigma^{2}-2 \sigma \sigma^{\prime} \cos \theta+\sigma^{\prime 2}\right)} . \tag{5}
\end{equation*}

Cette quantité peut donc être décrite comme l'hypoténuse d'un triangle rectangle, dont un côté a pour longueur l'écart $|{a}-{a}^{\prime}|$ entre les moyennes de $X$ et de $Y$ et dont l'autre côté est le troisième côté d'un triangle dont deux côtés ont pour longueurs $\sigma$ et $\sigma{ }^{\prime}$, l'angle compris entre ces deux côtés étant égal à $\theta$ (ou encore le cosinus de cet angle étant égal au coefficient de corrélation (linéaire) de $X$ et de $Y$).

On observera que, dans l'espression (5), $a, a^{\prime}, \sigma, \sigma$ ' sont \underline{déterminés connaissant} $F$ et $G$ et \underline{c'est seulement} $r=\cos \theta$ qui dépend de ${H(x, y) \text {. Le }}$ minimum de $\mathfrak{M}_{{H}}({X}-{Y})^{2}$ aura donc lieu quand ${r}=\cos \theta$ sera le plus grand possible. Plus précisément la distance entre les deux lois de probabilités est donc:
\begin{equation*}
\left(L, L^{\prime}\right)=\sqrt{\left(a-a^{\prime}\right)^{2}+\left(\sigma^{2}-2 \sigma \sigma^{\prime} \rho+\sigma^{\prime^{2}}\right)} \tag{6}
\end{equation*}
où $\rho$ est la borne supérieure du coefficient de corrélation (linéaire) entre $X$ et $Y$ , quand la loi de probabilité du couple ${X}, {Y}$ varie de façon à laisser fixes les lois de probabilité de $X$ et de $Y$ pris séparément.

Observons d'ailleurs que:
$$
r=\frac{\iint(x-a)\left(y-a^{\prime}\right) \mathrm{d}  H(x, y)}{\sqrt{\left[(x-a)^{2} \mathrm{d} F\right]\left[\int\left(y-a^{\prime}\right)^{2} \mathrm{d}  G\right]}}\,.
$$

Posons: $h(z, t)=H\left(a+\sigma z, a^{\prime}+\sigma{ }^{\prime} t\right)$. Alors : $r=\dfrac{\iint \sigma \sigma^{\prime}z t \mathrm{d} h(z, t)}{\sqrt{\ldots}}$ d'où:
\begin{equation*}
r=\iint_{\text{P}} z t \mathrm{d} h(z, t) . \tag{7}
\end{equation*}

De sorte que r est aussi le coefficient de corrélation (linéaire) de $Z$ et de $T$ et est exprimé par la formule (7) où $h(z, t)$ est une fonction de répartition dont les marges sont données et identiques à
$$
\varphi(z) \equiv F(a+\sigma z) \qquad \psi(t) \equiv G\left(a^{\prime}+\sigma^{\prime} t\right)
$$

Tout le problème est ramené à trouver la borne supérieure de l'expression:
\begin{equation*}
r=\int_{-\infty}^{+\infty} \int_{-\infty}^{+\infty} z t \mathrm{d} h(z, t) \tag{8}
\end{equation*}
quand $h$ est une fonction de répartition dont les marges $\varphi(z)$ et $\psi(t)$ sont données. On sait, que $r=\cos \theta=+1$ dans le cas où il y a une relation fonctionnelle \underline{linéaire} croissante
$$
{Y}={m} {X}+{p} \quad \text { avec } {m > 0}\,,
$$
entre $X$ et $Y$. Dans ce cas, on a donc plus simplement
\begin{equation*}
\left(L, L^{\prime}\right)=\sqrt{\left(a-a^{\prime}\right)^{2}+\left(\sigma-\sigma^{\prime}\right)^{2}} . \tag{9}
\end{equation*}

Dans l'article de 1954 cité en note plus haut, Salvemini avait conjecturé que le minimum de:
$$
J=\int_{-\infty}^{+\infty} \int_{-\infty}^{+\infty}(x-y)^{2} \mathrm{d}_x \mathrm{d}_y H(x, y)
$$
est atteint pour $H$ identique à la fonction ${H}_{1}({x}, {y})$.citée plus haut.

En 1955, Bass a énoncé dans sa note citée plus haut, ce résultat équivalent (d'après la formule (6)), que le maximum du coefficient de corrélation (linéaire) est obtenu pour ${H} \equiv {H}_{1}$. Sa démonstration(qu'il a bien voulu me communiquer par écrit) suppose que $X$ et $Y$ \underline{sont bornées}.

L'année suivante, dans son article cité plus haut, Dall'Aglio démontre que $J$ est minimum pour $H=H_{1}$, dans l'hypothèse \underline{plus générale} où
$$
\begin{aligned}
& 0=\lim_{x \rightarrow-\infty} x^{\gamma} F(x)=\lim_{y \rightarrow-\infty} y^{\gamma} \\
& 0=\lim_{x \rightarrow+\infty} x^{\gamma}[1-F(x)]=\lim_{y \rightarrow+\infty} y^{\gamma}[1-G(y)]
\end{aligned}
$$
pour $\gamma \geqslant 2$.

Il donne même l'expression suivante du minimum M soit:
\begin{align*}
M & =2 \int_{-\infty}^{+\infty} \mathrm{d} y \int_{y}^{+\infty} \operatorname{Sup}\{G(y)-F(x), 0\} \mathrm{d} x\,+  \tag{10}\\
& +\,2 \int_{-\infty}^{+\infty} \mathrm{d} x \int_{x}^{+\infty} \operatorname{Sup}\{F(x)-G(y), 0\} \mathrm{d} y
\end{align*}

Mais on peut donner une expression plus commode de ce minimum (qui est égal à $\Delta^{2}$).

On peut arriver dedeux façons à cette autre expression de $\Delta^{2}$. Faisons le calcul de $\Delta^{2}$ dans le cas où $F(x), G(y)$ sont partout continus et ne sont constants, l'un ou l'autre, dans aucun intervalle. Alors l'équation:
$$
F(x)=G(y)
$$
représente une courbe $\Gamma$ qui est coupée en un point et un seul par toute parallèle à l'un des axes et sur laquelle y croît avec $x$ et réciproquement. On a $H_{1}(x, y)=F(x)$ au-dessus (vers les y positifs) de $\Gamma$ et $H_{1}(x, y)=G(y)$ au-dessous de $\Gamma$.

Considérons une suite de nombres $\ldots x_{-h}, \ldots x_{-1}, x_{0}, x_{1}, \ldots x_{k} \ldots$ croissent de $-\infty$ à $+\infty$; les nombres $y_{j}$ correspondants, tels que:
$$
F\left(x_{j}\right)=G\left(y_{j}\right)
$$
croitront aussi de $-\infty$ à $+\infty$. La courbe $\Gamma$ sera contenue dans la suite $S$ de rectangles:
$$
x_{j} \leqslant x<x_{j+1} \quad ; \quad y_{j} \leqslant y<y_{j+1}\,.
$$

Au-dessus de ces rectangles, $H_{1}(x, y)=F(x)$ et au-dessous ${H}_{1}({x}, {y})={G}({y})$. Dès lors, l'intégrale:
$$
\iint_{B}(x-y)^{2} \mathrm{d} x \mathrm{d} y H_{1}(x, y)
$$
étendue à la région $B$ extérieure aux rectangles de $S$ est nulle et on a
$$
\int_{-\infty}^{+\infty} \int_{-\infty}^{+\infty}(x-y)^{2} \mathrm{d}^{2} H_{1}(x, y)=\iint_{s}(x-y)^{2} \mathrm{d}^{2} H_{1}(x, y)
$$

On a donc:
$$
\begin{gathered}
\quad \mathfrak{M}_{H_{1}}(X-Y)^{2}=\lim \sum_{i=-\infty}^{i=+\infty} \sum_{j=-\infty}^{j=+\infty}\left(x_{i}-y_{j}\right)^{2} \Delta_{i j} H_{1} \\
=\lim \sum_{i}\left(x_{i}-y_{i}\right)^{2}\left[H_{1}\left(x_{i+1}, y_{j+1}\right)-H_{1}\left(x_{i+1}, y_{i}\right)-H_{1}\left(x_{i}, y_{i+1}\right)+H\left(x_{i}, y_{i}\right)\right] .
\end{gathered}
$$
Or
$$
\begin{aligned}
& H_{1}\left(x_{i+1}, y_{i+1}\right)=F\left(x_{i+1}\right)=G\left(y_{i+1}\right) \\
& H_{1}\left(x_{i}, y_{i}\right)=F\left(x_{i}\right)=G\left(y_{i}\right) \\
& H_{1}\left(x_{i+1}, y_{i}\right)=G\left(y_{i}\right), \quad H_{1}\left(x_{i}, y_{i+1}\right)=G\left(y_{i}\right)=F\left(x_{i}\right) .
\end{aligned}
$$

Donc le crochet est égal à:
$$
F\left(x_{i+1}\right)-F\left(x_{i}\right)
$$
et par suite:
$$
\mathfrak{M}_{H_{1}}(X-Y)^{2}=\lim \sum_{i}\left(x_{i}-y_{i}\right)^{2}\left[F\left(x_{i+1}\right)-F\left(x_{i}\right)\right] .
$$

Puisque l'équation
\begin{equation*}
F(x)=G(y) \tag{11}
\end{equation*}
a une solution continue et croissante en $y$:
$$
y=\lambda(x), \text { on voit qu'on aura: }
$$
$$
\Delta^{2}=\mathfrak{M}_{H_{1}}(X-Y)^{2}=\int_{-\infty}^{+\infty}[x-\lambda(x)]^{2} \mathrm{d} F(x)
$$
En tirant, au contraire, de (11)
$$
x=\mu(y)
$$
on pourrait aussi écrire:
$$
\Delta^{2}=\int_{-\infty}^{+\infty}[\mu(y)-y]^{2} \mathrm{d} G(y)
$$

De la même façon, la borne supérieure $\rho$ de $r$ est déterminée par la formule
$$
\sigma \sigma^{\prime} \rho=\int_{-\infty}^{+\infty}(x-a)\left[\lambda(x)-a^{\prime}\right] \mathrm{d} F(x)=\int_{-\infty}^{+\infty}\left(y-a^{\prime}\right)[\mu(y)-a] \mathrm{d} G(y) .
$$

On peut obtenir encore plus facilement ces expressions en observant que si la fonction de répartition est $H_{1}(x, y)$, il y a presque certainement une relation fonctionnelle entre les deux nombres aléatoires $X$ et $Y$ , à savoir:
$$
Y=\lambda(X) .
$$
Dès lors:
$$
\mathfrak{M}_{H_{1}}(X-Y)^{2}=\mathfrak{M}_{H_{1}}[\lambda(X)-X]^{2}
$$

\begin{equation*}
\left(L, L^{\prime}\right)^{2}=\int_{-\infty}^{+\infty}[\lambda(x)-x]^{2} \mathrm{d} F(x) \tag{12}
\end{equation*}

En posant $W=F(X)=G(Y), X$ et $Y$ sont deux fonctions continues croissantes de $W$:
$$
{X}=l({W}) \quad ; \quad {Y}={m}(W)
$$
et $W$ a une densité de probabilité constamment égale à 1 sur 0,1 . On a alors
\begin{equation*}
\left(L, L^{\prime}\right)^{2}=\int_{0}^{1}[l(t)-m(t)]^{2} \mathrm{d} t \tag{13}
\end{equation*}

Dans les notations précédentes, 
$$
 \Delta^{2}=\left(a^{\prime}-a\right)^{2}+\left(\sigma^{2}-2 \sigma \sigma^{\prime} \rho+\sigma^{\prime 2}\right)$$
où
$$
 \rho=\int_{-\infty}^{+\infty} \int_{-\infty}^{+\infty} z t \mathrm{d} h (z, t)
$$
on aura:
$$
\rho=\int_{-\infty}^{+\infty} z v(z) \mathrm{d} \varphi(z)
$$
si $t=v(z)$ est équivalent à: $\varphi(z)=\psi(t)$.

\noindent \underline{\textbf{Remarque}:}

La formule (10) de Dall'Aglio et les formules (12), (13) résolvent le problème posé (en note) par Salvemini dans son article cité plus haut.

\noindent \underline{\textbf{Exemple}:}

Supposons que $X$ et $Y$ soient telles que leurs variables "réduites" $Z$ et $T$ aient la même loi de probabilité. Alors, parmi les couples $X, Y$ il y aura un couple pour lequel $Z=T$. Alors, il y a une relation fonctionnelle linéaire croissante entre $X$ et $Y$ pour $H=H_{1}$ et on aura encore comme à la formule (9).

\begin{equation*}
\Delta=\sqrt{\left(a-a^{\prime}\right)^{2}+\left(\sigma-\sigma^{\prime}\right)^{2}} \,. \tag{14}
\end{equation*}

On a ainsi un résultat particulièrement simple. La formule (14) convient, quand, par exemple, les marges ont une distribution dite normale. Mais elle convient aussi quand les marges vérifient toutes deux la lère loi de Laplace, ou sont toutes deux uniformes, etc...

Elle convient encore, plus généralement, quand $X$ et $Y$ ont une même loi réduite de probabilité comportant un écart quadratique moyen fini.\\

\noindent \underline{\textbf{Généralisation}:}

Dall'Aglio a montré que si l'on prenait
$$
([{X}],[{Y}])_{{H}}=\sqrt[s]{\mathfrak{M}_{{H}}|{X}-{Y}|^{s}}
$$
le minimum est, pour $s \geqslant 1$ atteint pour $H \equiv H_{1}$.

On voit comme plus haut, $p_{.}=$que si $F(x)$ et $G(y)$ sont continus et croissants, l'on a alors
$$
\left(L, L^{\prime}\right)^{s}=\int_{-\infty}^{+\infty}| \lambda(x)-x|^s \mathrm{d} F(x) \, \text{ ou } \, \left(L, L^{\prime}\right)^{s}=\int_{-\infty}^{+\infty}|l(t)-m(t)|^{s} \mathrm{d} t .
$$

\subsection*{UNE QUATRIÈME DÉFINITION DE LA DISTANCE DE DEUX LOIS DE PROBABILITÉ}

La première des trois définitions de ($L, L^{\prime}$) dues à Lévy est très séduisante. Car elle explicite d'une façon très simple et très naturelle la notion intuitive que nous pouvons avoir de la distance (${L}, {L}^{\prime}$) de deux lois de probabilité $L, L^{\prime}$.

Son plus grand inconvénient, c'est que, variant avec la définition adoptée comme point de départ de la distance globale de deux nombres aléatoires, elle exigera à chaque fois la détermination \underline{préalable} du \underline{minimum} de cette distance quand varie la corrélation de ces deux nombres.\\

\noindent \underline{\textbf{Une quatrième définition}:}

Nous allons donc proposer une quatrième définition de ($L, L^{\prime}$), pour \underline{esquiver} cette difficulté. Nous ne considérons donc pas notre définition comme meilleure mais seulement comme d'application plus immédiate. Nous verrons d'ailleurs ensuite que les deux définitions sont équivalentes dans un cas étendu. Elles sont probablement équivalentes dans des cas plus généraux encore, sinon dans tous les cas.\\

\noindent \underline{\textbf{Nouvelle définition de (${L}, {L}^{\prime}$)}:}

Prenons encore comme point de départ, l'une des définitions admissibles, de la distance "globale", $([{X}],[{Y}])_{{H}}$, de deux nombres aléatoires $X, Y$ --- déterminés simultanément dans chaque épreuve d'une catégorie déterminée, correspondant à la fonction de répartition ${H}({X}, {Y})$ du couple ${X}, {Y}$.

Ceci étant, nous prendrons comme nouvelle définition de la distance de deux lois $L, L^{\prime}$ la quantité :
\begin{equation*}
\left(L, L^{\prime}\right)=([X],[Y])_{H_{1}} \tag{15}
\end{equation*}
où ${X}, {Y}$ obéis sent aux deux lois ${L}, {L}^{\prime}$. Ainsi nous appelons distance de 2 lois de probabilité $L, L'$, la valeur que prend une distance "globale" de deux nombres aléatoires ${X}, {Y}$, obéissant séparément aux lois ${L}, {L}^{\prime}$, quand la fonction ${H}({x}, {y})$ de répartition du couple ${X}, {Y}$ atteint sa valeur maximum ${H}_{1}({x}, {y})$ précisée par la formule $(2)$.

Il faut maintenant prouver que cette quantité ($L, L^{\prime}$) est bien "une distance"; c'est-à-dire satisfait aux trois conditions bien connues, rappelées pages 1,2, sous les n$^{\circ} 1,2^{\circ}, 3^{\circ}$. On aura ainsi une justification partielle a posteriori de la définition que nous venons de poser dogmatiquement.

Par hypothèse, pour toute fonction de corrélation ${H}({x}, {y})$ admettant pour marges les fonctions de répartition $F(x), G(y)$ des lois $L, L^{\prime}$, la distance globale de $[X]$ et $[Y]$ vérifie les conditions:
$$
\begin{aligned}
  &1^{\circ}\; ([{X}],[{Y}])_{{H}}=([{Y}],[{X}])_{{H}} \geqslant 0\\
  &2^{\circ}\; ([X],[Y])_{H} \text{ est positif si } X \text{ et } Y \text{ sont "distincts" et inversement.}  \\
\end{aligned}
$$
(On considère, en général, comme non distincts deux nombres aléatoires qui sont "presque certainement" égaux, c'est-à-dire tels que:
$
\{\operatorname{Prob}({X}={Y})\}=1
$.)

C'est aussi la condition nécessaire et suffisante pour que $F(x) \equiv G(x)$. Dès lors en appliquant au cas où ${H} \equiv {H}_{1}$
$$
\begin{aligned}
& 1^{\circ}\;\left(L, L^{\prime}\right)=\left(L^{\prime}, L\right) \geqslant 0 \\
& 2^{\circ}\;\left(L, L^{\prime}\right)=0 \text { si } L \equiv L^{\prime} \text { et inversement. }
\end{aligned}
$$
En ce qui concerne la condition $3^{\circ}$, nous devons faire intervenir trois lois de probabilité $L, L^{\prime}, L^{\prime \prime}$, correspondant à trois fonctions de répartition ${F}({x}), {G}({y}), {K}({z})$. Introduisons une corrélation particulière entre trois nombres aléatoires ${X}, {Y}, {Z}$, obéissant respectivement aux trois lois $L, L^{\prime}$, $L^{\prime \prime}$. Nous choisissons à cet effet la corrélation définie par la fonction de répartition:
$$
E(x, y, z)=\min [F(x), G(y), H(z)]\,.
$$

On voit bien que si le système $X, Y, Z$ a pour fonction de répartition $E(x, y, z), X, Y, Z$ auront bien $F(x), G(y), H(z)$ comme fonctions de répartition. Car, par exemple,
$$
\begin{aligned}
& \operatorname{Prob}(X<x)=\operatorname{Prob}(X<x, Y<+\infty, Z<+\infty) \\
& =E(x,+\infty,+\infty)=\min (F(x),+1,+1)=F(x)
\end{aligned}
$$
On aura de plus:
$$
E(x, y,+\infty)=\min [F(x), G(y),+1]=H_{1}(x, y)
$$
et de même les fonctions maximées de répartition de $(X, Z)$ et de $(Y, Z)$ seront
$$
\begin{aligned}
& H_{1}^{\prime}(x, z)=E(x,+\infty, z) \\
& H_{1}^{\prime \prime}(y, z)=E(+\infty, y, z)\,.
\end{aligned}
$$
Ceci étant, on a:
\begin{equation*}
([X],[Y])_{H_{1}}=([X],[Y])_{E(x, y,+\infty)}=([X],[Y])_{E(x, y, z)} \tag{16}
\end{equation*}

Or, par hypothèse, pour n'importe quelle fonction de répartition à trois variables, $U(x, y, z)$, ayant les marges données $F, G, K$ on a:
$$
([{X}],[{Y}])_{{U}} \leqslant([{X}],[{Z}])_{{U}}+([{T}],[{Z}])_{{U}} .
$$

Donc, en prenant en particulier E pour U et utilisant les deux égalités analogues à (4), on a:
$$
([{X}],[{Y}])_{{H}_{1}} \leqslant([{X}],[{Z}])_{{H}_{1}^{\prime}}+([{Y}],[{Z}])_{{H}_{1}^{\prime \prime}}
$$
c'est-à-dire:
$$
\left(L, L^{\prime}\right) \leqslant\left(L, L^{\prime \prime}\right)+\left(L^{\prime}, L^{\prime \prime}\right) .
$$

\noindent \underline{\textbf{Equivalence}:}

Il résulte des démonstrations de Bass et de Dall'Aglio que \underline{dans le cas} où l'on a pris:
$$
([{X}],[{Y}])_{{H}}=\sqrt{\mathfrak{M}_{{H}}({X}-{Y})^{2}}
$$
et sous les restrictions très générales et qui,d'ailleurs, ne sont peut-être pas nécessaires, la valeur de ($L, L^{\prime}$) reste la même qu'on emploie la première définition de Paul Lévy ou la nôtre.

\noindent \underline{\textbf{Calcul général de (${L}, {L}^{\prime}$)}:}

Considérons le cas où $F(x)$ et $G(y)$ sont des fonctions partout \underline{continues} et \underline{croissantes}. Alors la courbe $\Gamma$:
$$
F(x)=G(y)
$$
va séparer la région $R$ où $H_{1}=F(\leqslant G)$ de celle, $Q_{1}$, où $H_{1}=G(\leqslant F)$. Si l'on pose:
$$
F(x)=G(y)=t
$$
on voit comme plus haut que $x$ et $y$ seront des fonctions continues et croissantes de $t$, soit:
$$
x=l(t) \qquad\qquad y=m(t) .
$$

Quand la fonction de répartition est : $H_{1}(x, y)=\min [F(x), G(x)]$, la différence seconde de $H_{1}$ sera nulle à l'intérieur de $R$ et à l'intérieur de $Q$, c'est-à-dire que le point (${X}, {Y}$) est presque certainement sur $\Gamma$.

Autrement dit, ily a dans ce cas une relation fonctionnelle presque certaine entre $X$ et $Y$, à savoir:
$$
F(x)=G(y) .
$$

Le nombre aléatoire $T$ égal à la valeur commune de $F$ et $G$ sur $\Gamma$ reste entre 0 et 1 avec une densité de probabilité constante et égale à 1.

Il en résulte l'expression de ($L, L^{\prime}$):
$$
\left({L}, {~L}^{\prime}\right)=([l({T})],[{m}({T})]) .
$$

\noindent \underline{\textbf{Exemple}:}

Par exemple, si l'on part de l'expression:
$$
([X],[Y])_{H}=\sqrt[\alpha]{\int_{-\infty}^{+\infty} \int_{-\infty}^{+\infty}|x-y|^{\alpha} \mathrm{d}_{x} \mathrm{d}_{y} H(x, y)}=\sqrt[\alpha]{\mathfrak{M}_{H}|X-Y|^{\alpha}}
$$
avec
$$
\alpha \geqslant 1,
$$
on aura:
$$
\left(L, L^{\prime}\right)^{\alpha} =\mathfrak{M}|l(T)-m(T)|^{\alpha} \quad, \quad \text { d'où : }$$
$$
\left(L, L^{\prime}\right)^{\alpha} =\int_{0}^{1}|l(t)-m(t)|^{\alpha} \mathrm{d} t .
$$

On peut aussi résoudre:
$$
F(x)=G(y)
$$
en $y=\lambda(x)$,
où $\lambda(x)$ sera, comme $F$ et $G$, une fonction continue croissante. On pourra alors écrire:
$$
\left(L, L^{\prime}\right)^{\alpha}=\int_{-\infty}^{+\infty}|x-\lambda(x)|^{\alpha} \mathrm{d} F(x)
$$

\subsection*{L'INDICE DE DISSEMBLANCE DE GINI}

Pour deux suites également nombreuses de nombres non décroissants;

$$
a_{1} \leqslant a_{2} \leqslant \ldots \leqslant a_{n} \quad, \quad b_{1} \leqslant b_{2} \leqslant \ldots \leqslant b_{n},
$$
cet indice est posé égal à
$$
I_{\alpha}=\sqrt[\alpha]{\frac{1}{n} \sum_{h=1}^{n}\left|a_{h}-b_{h}\right|^{\alpha}} \quad \begin{aligned}
& \alpha=1 \text { : indice simple } \\
& \alpha=2 \text { : indice quadratique }
\end{aligned}
$$
Mais on peut prendre n'importe quel $\alpha \geqslant 1$.

Les a n'étant pas nécessairement distincts, leurs valeurs distinctes sont répétées, $r_{1}$ fois,... $r_{n}$ fois. Elles peuvent être considérées comme les valeurs prises par une grandeur statistique $X$ dans $n$ épreuves. Les valeurs distinctes de ${X}: {x}_{1}<{x}_{2}<\ldots$ auront les fréquences:
$$
f_{1}=\frac{r_{1}}{n}, \quad f_{2}=\frac{r_{2}}{n}, \ldots \quad \text { La suite }\left\{\begin{array}{l}
x_{1}, x_{2}, \ldots \\
f_{1}, f_{2}, \ldots
\end{array}\right.
$$
définit ainsi une loi de fréquence $L$. De même, la suite des valeurs distinctes $y_{1}, y_{2} \ldots$ prises par les $b_{j}$ avec les fréquences: $\varphi_{1}=\dfrac{s_{1}}{n}, \varphi_{2}=\dfrac{s_{2}}{n}, \ldots$ définit une loi de fréquence $L^{\prime}$.

En permuttant les $b_{h}$, on obtient une suite $b_{1}^{\prime}, b_{2}^{\prime}, \ldots$ qui n'est plus nécessairement non décroissante. Si chaque épreuve associait à un $a_{h}$, $b_h$, on aurait une loi $H$ de fréquence du couple ${X}, {Y}$. En associant ${b}_{{h}}$ à ${a}_{{h}}$, on a une loi particulière, ${H}^{\prime}$, de fréquence de ce couple. Nous allons montrer que ${H}^{\prime}={H}_{1}$, de sorte que l'indice de dissemblance de Gini deviendra identique à ce à quoi se réduit notre distance de $L$ et de $L^{\prime}$ dans le cas particulier où $L$, $L'$ sont les lois de deux grandeurs statistiques (ayant chacune un nombre fini de valeurs).

En effet, supposons d'abord:
$$
a_{1}<x \leqslant a_{n} \quad, \quad b_{1}<y \leqslant b_{n}
$$
alors ily aura un $h$ et un $j$ tels que
$$
a_{h}<x \leqslant a_{h+1} \quad, \quad b_{j}<y \leqslant b_{j+1}\,.
$$
On aura
$$
H^{\prime}(x, y)=\operatorname{Prob}(x<x, Y<y)=\operatorname{Prob}\left(X<a_{h+1}, Y<b_{j+1}\right)
$$
et puisque ${H}^{\prime}$ correspond au cas où $b_j$ est associé à $a_j$, alors si $j<{h}$
$$
H^{\prime}(x, y)=\operatorname{Prob}\left(Y<b_{j+1}\right)=\operatorname{Prob}(Y<y)=G(y)
$$
et
$$
F(x)=\operatorname{Prob}\left(x<a_{h+1}\right) \geqslant \operatorname{Prob}\left(Y<b_{j+1}\right)=\operatorname{Prob}(Y<y) .
$$

Donc: si ${j} \leqslant {h}$
$$
\begin{gathered}
H^{\prime}(x, y)=G(y) \leqslant F(x) \\
H^{\prime}(x, y)=\min [F(x), G(y)]=H_{1}(x, y)\,.
\end{gathered}
$$

En répétant le même raisonnement pour ${h} \leqslant {j}$, on voit que dans les deux cas:
\begin{equation*}
{H}^{\prime}({x}, {y})={H}_{1}({x}, {y}) . \tag{1$^\prime$}
\end{equation*}

Dans le cas où $x\leqslant a_{1}$, on aurait évidemment:
$$
H^{\prime}(x, y)=F(x)=0 \leqslant G(y)
$$
et par suite (1$^\prime$) subsisterait; de même si $y \leqslant b$, raisonnement analogue pour ${x}>{a}_{{n}}$ ou ${y}>{b}_{{n}}$. Ainsi dans tous les cas \footnote{ Nous ne faisons ici que reprendre un peu plus en détail le raisonnement de Salvemini qui, du reste, ne s'occupe pas de la notion de distance.
}
\begin{equation*}
{H}^{\prime}({x}, {y}) \equiv {H}_{1}({x}, {y}) .
\end{equation*}

L'indice simple $(\alpha=1)$ ou quadratique $(\alpha=2)$ de dissemblance, habilement choisi par Gini, se trouve ainsi être en même temps une "distance", de deux lois de fréquence. Plus précisément, il rentre dans la catégorie plus générale de la quatrième définition de la distance de deux lois de probabilité absolument quelconques (discrètes ou continues ou intermédiaires) précisée p.11. Il présente, d'autre part, cet intérêt d'offrir un mode de calcul plus simple que celui qui résulterait directement de la formule:
$$
I_{\alpha}=\sqrt[\alpha]{\mathfrak{M}_{H_{1}}|X-Y|^{\alpha}}\,.
$$

\end{document}
