# Supplementary material for: A Brief History of Fr\'echet Distances: From Curves and Probability Laws to FID
Source: arXiv:2604.21745 source file (2026-04-23)
Supplement: Supplementary file 3 [file levy1950_fr.tex]

%! LW recipe=xelatex

\documentclass[10pt]{article}
\usepackage[french]{babel}
\usepackage[utf8]{inputenc}
\usepackage[T1]{fontenc}
\usepackage{amsmath}
\usepackage{amsfonts}
\usepackage{amssymb}
\usepackage[version=4]{mhchem}
\usepackage{stmaryrd}
\usepackage{bm}

%New command to display footnote whose markers will always be hidden
\let\svthefootnote\thefootnote
\newcommand\blfootnotetext[1]{%
  \let\thefootnote\relax\footnote{#1}%
  \addtocounter{footnote}{-1}%
  \let\thefootnote\svthefootnote%
}

%Overriding the \footnotetext command to hide the marker if its value is `0`
\let\svfootnotetext\footnotetext
\renewcommand\footnotetext[2][?]{%
  \if\relax#1\relax%
    \ifnum\value{footnote}=0\blfootnotetext{#2}\else\svfootnotetext{#2}\fi%
  \else%
    \if?#1\ifnum\value{footnote}=0\blfootnotetext{#2}\else\svfootnotetext{#2}\fi%
    \else\svfootnotetext[#1]{#2}\fi%
  \fi
}

\begin{document}
% demonstration précédente). Sans démontrer ce supprimer $\varepsilon$ dans la qualte aisément du fait que les lois de propoint, indiquons qu'il i que l'on peut considérer lorsque le babilité à deux variables X , forment un ensemble compact.

\textbf{Définitions directes de la distance des deux lois.} --- La définition qui précède présente l'inconvénient qu'il peut être très difficile de déterminer la distance de deux lois données par leurs fonctions des probabilités totales. Il est donc utile d'avoir des définitions directes. Nous allons en indiquer deux.\\

$1^{\circ}$ La première 
est celle que j'ai indiquée ou 
plutôt utilisée (sans prononcer le mot de distance) en 1925 
(Calcul des probabilités, p. 199--200). Définissons la loi $\bm{L}$ dont dépend une variable aléatoire $\bm{X}$  par la courbe $\bm{\Gamma}$ représentant la fonction des probabilités totales
$$
y=\operatorname{Pr}[\bm{X}<x]
$$
avec toutefois cette convention qu'à chaque valeur de $x$ pour laquelle cette fonction est discontinue, nous ferons correspondre le segment
$$
\operatorname{Pr} [\bm{X}<x] \leqq y \leqq \operatorname{Pr} [\bm{X} \leqq x]\,.
$$

La courbe est alors continue, et manifestement coupée en un point et un seul par n'importe quelle parallèle à la droite
$$
x+y=0
$$

Deux lois $\bm{L}$ et $\bm{L}^{\prime}$ étant ainsi représentées par deux courbes $\bm{\Gamma}$ et $\bm{\Gamma}^{\prime}$ que la droite $x+y=c$ coupe respectivement en $\bm{A}$ et $\bm{A}^{\prime}$, la distance $\left(\bm{L}, \bm{L}^{\prime}\right)=\left(\bm{\Gamma}, \bm{\Gamma}^{\prime}\right)$ sera le maximum de $\bm{AA}^{\prime}$ quand $c$ varie de $-\infty$ à $+\infty$. Ce maximum est sûrement atteint, à cause de la continuité des courbes $\bm{\Gamma}$ et $\bm{\Gamma}^{\prime}$.

% \footnotetext{dic que (L,L') tend vers zéro est plus délicate. Prenons par exemple pour $X$ une variable aléatoi pouvant prendre les valeurs $2,4, \ldots, 2 n$, toutes ces valeurs étant ggalement probables, et pour Y une variable admettant de mème $n$ valeurs possibles et egalement probables : $1,3, \ldots, 2 n-1$; quelle que soit la corrélation entre $X$ et $Y$, on a súrement $|X-\bm{Y}| \geqslant 1$, et $\left(\bm{L}, \bm{L}^{\prime}\right)$ ne tend pas vers zéro pour $n$ infini. En Prenant au contraire les définitions de la distance que nous indiquons plus loin, on trouverait que la distance des deux mémes lois tend vers zéro.
% }

Pour justifier cette définition, il suffit d'observer que l'inégalité triangulaire (2) est une conséquence de l'inégalité
\begin{equation*}
\bm{A} \bm{A}^{\prime} \leqq \bm{A}\bm{A}^{\prime\prime} + \bm{A}^{\prime}\bm{A}^{\prime \prime} \,, \tag{3}
\end{equation*}
écrite pour la valeur de $c$ qui rend $\bm{AA}^{\prime}$ maximum, done égal à ($\bm{L}, \bm{L}^\prime$). La droite $x+y=c$ coupant en $\bm{A}^{\prime \prime}$ la courbe $\bm{\Gamma}^{\prime \prime}$ qui correspond à $\bm{L}^{\prime \prime}$, on a bien
$$
\bm{A}\bm{A}^{\prime \prime} \leqq\left(\bm{L}, \bm{L}^{\prime \prime}\right), \quad \bm{A}^{\prime} \bm{A}^{\prime \prime} \leqq\left(\bm{L}^{\prime}, \bm{L}^{\prime \prime}\right),
$$
et (2) en résulte.\\

$2^{\circ}$ Voici maintenant une deuxième définition possible, qui comprend en fait une infinité de définitions, car elle utilise la notion de distance de deux points $\bm{A}$ et $\bm{A}^{\prime}$ du plan, et il n'est pas nécessaire que cette distance soit la distance euclidienne; nous supposerons seulement qu'elle tende vers zéro en même temps que la distance euclidienne. De toute façon, la distance ($\bm{A}, \bm{\Gamma}^{\prime}$) de $\bm{A}$ à $\bm{L}^{\prime}$ sera le minimum de $\bm{AA}^{\prime}$ quand $\bm{A}^{\prime}$ décrit $\bm{\Gamma}^{\prime}$, et la distance $\left(\bm{L}, \bm{L}^{\prime}\right)=\left(\bm{\Gamma}, \bm{\Gamma}^{\prime}\right)$ sera le plus grand des deux nombres suivants : maximum de ($\bm{A}, \bm{\Gamma}^{\prime}$) quand $\bm{A}$ décrit $\bm{\Gamma}$, et maximum de ($\bm{A}^{\prime}, \bm{\Gamma}$) quand $\bm{A}^{\prime}$ décrit $\bm{\Gamma}^{\prime}$.

Montrons que l'inégalité (2) est bien vérifiée. Prenons pour $\bm{A}$ un point quelconque de $\bm{\Gamma}$, pour $\bm{A}^{\prime \prime}$ le point de $\bm{\Gamma}^{\prime \prime}$ le plus voisin de $\bm{A}$ (ou un de ces points, s'il y en a plusieurs), et pour $\bm{A}^{\prime}$ le point de $\bm{\Gamma}^{\prime}$ le plus voisin de $\bm{A}^{\prime \prime}$. On a
$$
\left(\bm{A}, \bm{\Gamma}^{\prime}\right) \leqq \bm{A} \bm{A}^{\prime} \leqq \bm{A} \bm{A}^{\prime \prime}+\bm{A}^{\prime} \bm{A}^{\prime \prime} \leqq\left(\bm{L}, \bm{L}^{\prime \prime}\right)+\left(\bm{L}^{\prime}, \bm{L}^{\prime \prime}\right)\,.
$$

La même borne supérieure s'appliquant à ($\bm{A}, \bm{\Gamma}$), quel que soit $\bm{A}^{\prime}$ sur $\bm{\Gamma}^{\prime}$, l'inégalité (2) en résulte.

Cette définition de ($\bm{\Gamma}, \bm{\Gamma}^{\prime}$) peut s'appliquer à des courbes quelconques, mais ne serait pas sans inconvénient. Elle conduirait, en effet, si, par exemple, une ellipse a son petit axe très petit, à considérer l'ellipse complète, et la demi-ellipse située d'un côté déterminé du grand axe, comme deux courbes très peu différentes. M. Fréchet a donné une définition de la distance de deux courbes qui s'applique aux courbes de Jordan les plus générales et évite l'inconvénient que nous signalons. Nous n'en avons pas besoin ici, la définition qui précède suffisant pour les courbes très particulières que nous avons à considérer.

\textbf{Nouveau rapprochement entre la distance de deux lois et celle de deux variables aléatoires.} --- Nous ne considérerons ici que les définitions de la distance ($\bm{X}, \bm{Y}$) qui ne dépendent que de la nature de la variable aléatoire $\bm{Z=|X-Y|}$; alors
\begin{equation*}
(\bm{X}, \bm{Y})=(\bm{0}, \bm{Z}) . \tag{(4)}
\end{equation*}

Or, nous avons remarqué que, la notion de corrélation disparaissant lorsque l'une des variations cesse d'être aléatoire, il n'y a plus lieu de distinguer dans ce cas le voisinage des deux variables et celui des deux lois correspondantes. Peut-être même peut-on, $\bm{L}_{0}$ et $\bm{L}_{1}$ désignant respectivement les lois dont dépendent zéro et la variable non négative $\bm{Z}$, réaliser l'égalité des deux distances dont il s'agit:
\begin{equation*}
(\bm{o}, \bm{Z})=\left(\bm{L}_{0}, \bm{L}_{1}\right) . \tag{5}
\end{equation*}

Cette remarque conduit à poser les deux problèmes suivants :\\

\textbf{Premier problème.} --- \textit{Étant donnée une définition de ($\left.\bm{L}, \bm{L}^{\prime}\right)$ acceptable (c'est-à-dire vérifiant l'inégalité triangulaire), la définition de $(\bm{X, Y})$ que l'on en déduit par les formules (4) et (5) est-elle acceptable?}\\

\textbf{Deuxième problème.} --- \textit{Étant donnée une définition acceptable de $(\bm{X}, \bm{Y})$, peut-on donner de $\left(\bm{L}, \bm{L}^{\prime}\right)$ une définition acceptable et se réduisant dans le cas de la distance $\left(\bm{L}_{0}, \bm{~L}_{1}\right)$ à celle qui résulte des formules (4) et (5)?}\\

Nous nous contentons ici de poser ces questions générales et d'indiquer une manière particulière de réaliser les conditions (4) et (5), Il n'y a qu'à prendre pour ($\bm{A}, \bm{A}^{\prime}$), non la distance euclidienne de ces deux points, mais la somme
$$
\left|x-x^{\prime}\right|+\left|y-y^{\prime}\right|\,,
$$
$x, y$ étant les coordonnées de $\bm{A}$, et $x^{\prime}$ et $y^{\prime}$ celles de $\bm{B}$, puis à définir $\left(\bm{L}, \bm{L}^{\prime}\right)$ en partant de $\left(\bm{A}, \bm{A}^{\prime}\right)$ comme nous l'avons fait au $2^{\circ}$ du précédent paragraphe. On vérifie sans peine que la distance ($\bm{L}_{0}, \bm{L}_{1}$) est alors la distance du point $x=0,\, y=1$ à la courbe $\bm{\Gamma}_{1}$ correspondant à $\bm{L}_{1}$, c'est-à-dire le minimum, ɛ variant de o à $+\infty$, de la somme
$$
\varepsilon+\operatorname{Pr} \left[ | \bm{X}-\bm{Y} > \varepsilon \right],
$$
ce qui revient au même que de dire la borne inférieure de
$$
\varepsilon+\operatorname{Pr} \left[|\bm{X}-\bm{Y}| \geqq \varepsilon \right]
$$

C'est précisément la première des définitions de $(\bm{X}, \bm{Y})$, indiquée dans cet ouvrage (p. 205).\\

\textbf{L'espace des variables aléatoires.} --- Nous avons réservé pour la fin une remarque par laquelle il eût été plus logique de commencer; 
mais nous n'avons pas voulu risquer dès le début de décourager le lecteur par une notion assez abstraite et difficile à bien comprendre: 
si la notion de la distance de deux variables aléatoires est bien claire, celle d'espace des variables aléatoires l'est beaucoup moins. 
Il existe \textit{des espèces de variables aléatoires}; 
mais parler de \textit{l'espace des variables aléatoires}, 
sous-entendant par là qu'il s'agit d'un espace qui contienne toutes les variables aléatoires concevables, est aussi illusoire que de parler de l'ensemble de tous les ensembles concevables.

Je vais m'expliquer mieux. Lorsque nous parlons, par exemple, de l'espace des fonctions continues, nous pouvons le considérer comme préexistant, chaque point correspondant à une fonction bien déterminée, et nous ne risquons pas d'avoir jamais à considérer une fonction continue qui ne soit pas représentée par un point de cet espace. 
Au contraire, quelles que soient les variables aléatoires que nous ayons déjà considérées, 
quelque grande que soit la puissance de l'ensemble qu'elles forment, rien ne nous empêche de considérer une nouvelle variable aléatoire indépendante des précédentes. 
\textit{L'espace des variables aléatoires} est une construction qui n'est jamais terminée.

La définition donnée par M. Fréchet (p. 203) est, d'ailleurs, parfaitement correcte. En parlant d'\textit{une certaine catégorie d'épreuves}, il suppose arrêtée à un instant déterminé la construction de l'espace des variables aléatoires. Il m'a semblé qu'il n'était pas inutile d'indiquer plus explicitement la difficulté qu'il a ainsi écartée.

Je termine par une remarque relative au cas, surtout intéressant en pratique, où l'on ne considère que des variables aléatoires qui soient fonctions d'une infinité dénombrable de variables indépendantes. On sait (voir par exemple P. Lévy, Bull. Sc. Math., 1931 ; p. 87) que tous ces choix se ramènent au choix d'une seule variable $t$ choisie entre 0 et 1 (avec une répartition uniforme de la probabilité dans cet intervalle), et toutes les variables aléatoires considérées sont des fonctions mesurables de $t$. On peut alors considérer l'espace de variables aléatoires que l'on veut étudier comme appliqué sur l'espace des fonctions mesurables (et prendre dans ces deux espaces des définitions de la distance qui se correspondent). 
Cette application, possible d'une infinité de manières, ne supprime pas la difficulté signalée; car il suffit d'adjoindre aux précédentes une nouvelle variable aléatoire indépendante des autres pour que tout soit à recommencer; le mode d'application considéré devra être remplacé par un autre.

\end{document}
